# Supplementary material for: Automata and finite order elements in the Nottingham group
Source: arXiv:2008.04971 ancillary file (2020-10-01)

# Examples of automata of finite order elements of the Nottingham group

This Mathematica notebook accompanies the paper *Automata and finite order elements of the Nottingham group* by Jakub Byszewski, Gunther Cornelissen and Djurre Tijsma. The Package “IntegerSequences”, version 1.53 (30 May 2020) by Eric Rowland is used to represent automata. In this notebook, one finds all the automata discussed in the paper. The automata are ordered by the compositional order of the corresponding power series and then by their break sequence. For each finite order element we provide:

- the irreducible algebraic equation,
- the initial values and
- the corresponding automaton.

[written by Jakub Byszewski, Gunther Cornelissen and Djurre Tijsma, distributed under GNU Lesser General Public License v3.0]

```
Import[  
  "https://raw.githubusercontent.com/ericrowland/IntegerSequences/master/  
  IntegerSequences.m"];
```

---

## Order 2 elements

### Break sequence (1)

$\sigma_{V,1}$

```
fsigmaV1[t_, s_] := s + s^2 + t + s t + t^2 + s^3 t^3 + s^4 t^4
```

```
initsigmaV1[t_] := t + t^2 + 0[t]^3
```

```
automatonsigmaV1 = AutomaticSequenceAutomaton[AutomaticSequenceReduce[  
  AlgebraicSequence[SeriesRoot[{Function[s, fsigmaV1[t, s]], initsigmaV1[t]],  
    Modulus -> 2]][n], n, Method -> "Diagonal"]]
```

```
Out[*]= Automaton[{{1 -> 2, 0}, {1 -> 3, 1}, {2 -> 4, 0}, {2 -> 5, 1}, {6 -> 7, 0}, {6 -> 5, 1},  
  {7 -> 8, 0}, {7 -> 9, 1}, {4 -> 10, 0}, {4 -> 6, 1}, {8 -> 11, 0}, {8 -> 2, 1},  
  {10 -> 10, 0}, {10 -> 12, 1}, {11 -> 11, 0}, {11 -> 11, 1}, {12 -> 2, 0}, {12 -> 11, 1},  
  {3 -> 13, 0}, {3 -> 3, 1}, {9 -> 14, 0}, {9 -> 15, 1}, {16 -> 17, 0}, {16 -> 5, 1},  
  {5 -> 9, 0}, {5 -> 12, 1}, {13 -> 16, 0}, {13 -> 2, 1}, {14 -> 18, 0}, {14 -> 2, 1},  
  {17 -> 15, 0}, {17 -> 6, 1}, {15 -> 15, 0}, {15 -> 12, 1}, {18 -> 18, 0}, {18 -> 11, 1}},  
  1, {1 -> 0, 2 -> 0, 3 -> 1, 4 -> 0, 5 -> 1, 6 -> 0, 7 -> 0, 8 -> 0, 9 -> 1, 10 -> 0, 11 -> 0,  
  12 -> 0, 13 -> 1, 14 -> 1, 15 -> 1, 16 -> 1, 17 -> 1, 18 -> 1}, InputAlphabet -> {0, 1}]
```

```

edge[x_, ___] := {Arrowheads[0.030], Arrow[x, 0.1]}
AutomatonGraph[automatonsigmaV1, VertexSize → 0.3, EdgeShapeFunction → edge]

```

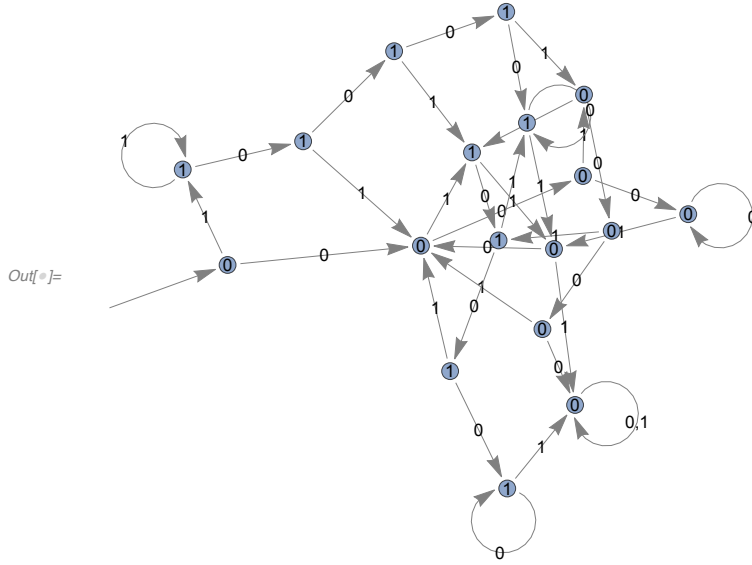
 $\sigma_{V,3}$ 

```

fsigmaV3[t_, s_] :=
  s + s^3 + t + s t + s^2 t + s^3 t + s t^2 + s^2 t^2 + s^3 t^2 + t^3 + s t^3 + s^2 t^3 + s^3 t^3 + s^4 t^4
initsigmaV3[t_] := t + t^2 + t^3 + 0[t]^5
automatonsigmaV3 = AutomaticSequenceAutomaton[AutomaticSequenceReduce[
  AlgebraicSequence[SeriesRoot[{Function[s, fsigmaV3[t, s]], initsigmaV3[t]],
    Modulus → 2]] [n], n, Method → "Diagonal"]]

```

Out[\*]= Automaton[{{1 → 2, 0}, {1 → 3, 1}, {4 → 5, 0}, {4 → 6, 1}, {2 → 7, 0}, {2 → 6, 1}, {5 → 8, 0}, {5 → 9, 1}, {10 → 8, 0}, {10 → 11, 1}, {12 → 13, 0}, {12 → 14, 1}, {15 → 5, 0}, {15 → 14, 1}, {7 → 10, 0}, {7 → 4, 1}, {8 → 16, 0}, {8 → 12, 1}, {13 → 17, 0}, {13 → 15, 1}, {16 → 16, 0}, {16 → 16, 1}, {17 → 17, 0}, {17 → 18, 1}, {18 → 12, 0}, {18 → 16, 1}, {3 → 19, 0}, {3 → 6, 1}, {20 → 21, 0}, {20 → 22, 1}, {23 → 24, 0}, {23 → 23, 1}, {6 → 20, 0}, {6 → 23, 1}, {9 → 24, 0}, {9 → 11, 1}, {22 → 20, 0}, {22 → 11, 1}, {19 → 9, 0}, {19 → 4, 1}, {11 → 11, 0}, {11 → 18, 1}, {25 → 25, 0}, {25 → 16, 1}, {21 → 11, 0}, {21 → 15, 1}, {24 → 25, 0}, {24 → 12, 1}, {14 → 9, 0}, {14 → 18, 1}}, 1, {1 → 0, 2 → 0, 3 → 1, 4 → 0, 5 → 0, 6 → 1, 7 → 0, 8 → 0, 9 → 1, 10 → 0, 11 → 1, 12 → 0, 13 → 0, 14 → 1, 15 → 0, 16 → 0, 17 → 0, 18 → 0, 19 → 1, 20 → 1, 21 → 1, 22 → 1, 23 → 1, 24 → 1, 25 → 1}, InputAlphabet → {0, 1}]

```

edge[x_, ___] := {Arrowheads[0.020], Arrow[x, 0.1]}
AutomatonGraph[automatonsigmaV3, VertexSize -> 0.3, EdgeShapeFunction -> edge]

```

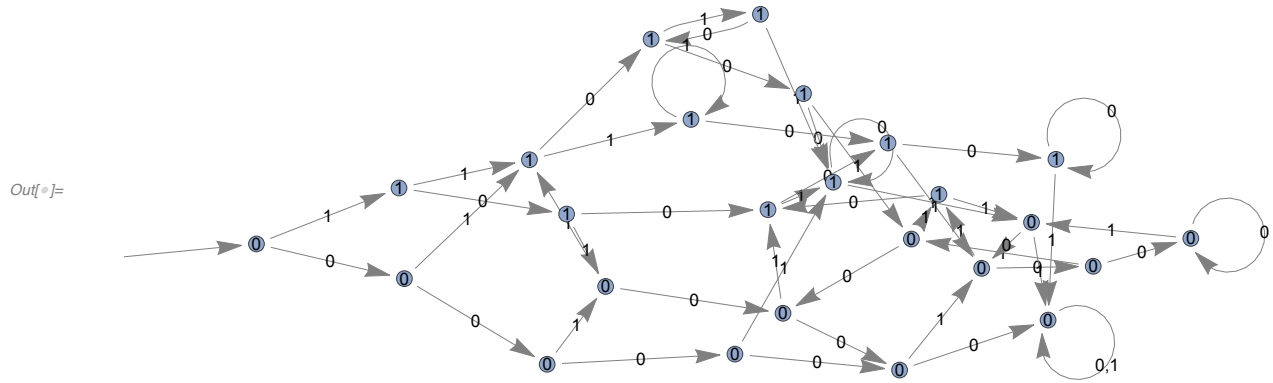

## Break sequence (3)

$\sigma_{K,3}$

```

fsigmaK3[t_, s_] := (t^3 + 1) s^3 + t^3

```

```

initsigmaK3[t_] := t + t^4 + 0[t]^5

```

```

automatonsigmaK3 = AutomaticSequenceAutomaton[AutomaticSequenceReduce[
    AlgebraicSequence[SeriesRoot[{Function[s, fsigmaK3[t, s]], initsigmaK3[t]],
        Modulus -> 2]] [n], n, Method -> "Diagonal"]]

```

```

Out[""]= Automaton[{{1 -> 2, 0}, {1 -> 3, 1}, {4 -> 5, 0}, {4 -> 6, 1}, {2 -> 1, 0}, {2 -> 5, 1},
    {5 -> 5, 0}, {5 -> 5, 1}, {3 -> 6, 0}, {3 -> 5, 1}, {6 -> 3, 0}, {6 -> 4, 1}},
    1, {1 -> 0, 2 -> 0, 3 -> 1, 4 -> 0, 5 -> 0, 6 -> 1}, InputAlphabet -> {0, 1}]

```

```

edge[x_, ___] := {Arrowheads[0.040], Arrow[x, 0.1]}

```

```

AutomatonGraph[automatonsigmaK3, VertexSize -> 0.3, EdgeShapeFunction -> edge]

```

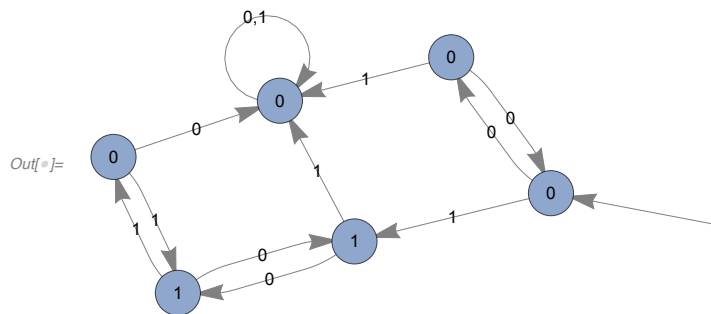

$\sigma_{CS}^{02}$ 

```

In[ ]:= fsigmaCS2[t_, s_] := s + s^2 + t + t^2 + s^2 t^2
initsigmaCS2[t_] := t + t^4 + 0[t]^5
automatonsigmaCS2 =
AutomaticSequenceAutomaton[AutomaticSequenceReduce[AlgebraicSequence[
SeriesRoot[{Function[s, fsigmaCS2[t, s]], initsigmaCS2[t]], Modulus -> 2]] [
n], n, Method -> "Diagonal"]]

Out[ ]:= Automaton[
{{1 -> 2, 0}, {1 -> 3, 1}, {4 -> 4, 0}, {4 -> 5, 1}, {2 -> 4, 0}, {2 -> 2, 1}, {6 -> 6, 0},
{6 -> 6, 1}, {3 -> 3, 0}, {3 -> 6, 1}, {5 -> 7, 0}, {5 -> 2, 1}, {7 -> 7, 0}, {7 -> 5, 1}},
1, {1 -> 0, 2 -> 0, 3 -> 1, 4 -> 0, 5 -> 1, 6 -> 0, 7 -> 1}, InputAlphabet -> {0, 1}]

In[ ]:= edge[x_, ___] := {Arrowheads[0.030], Arrow[x, 0.1]}
AutomatonGraph[automatonsigmaCS2, VertexSize -> 0.3, EdgeShapeFunction -> edge]

```

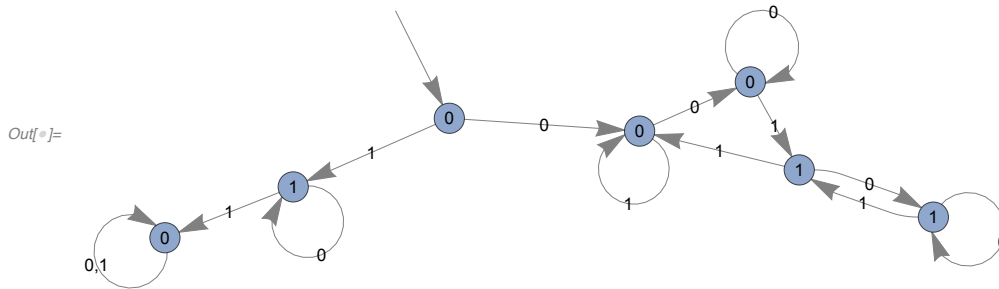

## Break sequence (5)

 $\sigma_{V,2}$ 

```

fsigmaV2[t_, s_] := s^4 + s^2 t + s t^2 + t^4 + s^4 t^4
initsigmaV2[t_] := t + t^6 + 0[t]^7
automatonsigmaV2 = AutomaticSequenceAutomaton[AutomaticSequenceReduce[
AlgebraicSequence[SeriesRoot[{Function[s, fsigmaV2[t, s]], initsigmaV2[t]],
Modulus -> 2]] [n], n, Method -> "Diagonal"]]

Out[ ]:= Automaton[{{1 -> 2, 0}, {1 -> 3, 1}, {4 -> 5, 0}, {4 -> 6, 1}, {7 -> 8, 0},
{7 -> 6, 1}, {8 -> 2, 0}, {8 -> 9, 1}, {2 -> 10, 0}, {2 -> 4, 1}, {5 -> 11, 0},
{5 -> 7, 1}, {10 -> 10, 0}, {10 -> 10, 1}, {11 -> 11, 0}, {11 -> 12, 1},
{12 -> 4, 0}, {12 -> 10, 1}, {3 -> 3, 0}, {3 -> 12, 1}, {13 -> 13, 0}, {13 -> 10, 1},
{6 -> 9, 0}, {6 -> 12, 1}, {14 -> 13, 0}, {14 -> 4, 1}, {9 -> 14, 0}, {9 -> 3, 1}},
1, {1 -> 0, 2 -> 0, 3 -> 1, 4 -> 0, 5 -> 0, 6 -> 1, 7 -> 0, 8 -> 0, 9 -> 1,
10 -> 0, 11 -> 0, 12 -> 0, 13 -> 1, 14 -> 1}, InputAlphabet -> {0, 1}]

```

```

edge[x_, ___] := {Arrowheads[0.030], Arrow[x, 0.1]}
AutomatonGraph[automatonsigmaV2, VertexSize → 0.3, EdgeShapeFunction → edge]

```

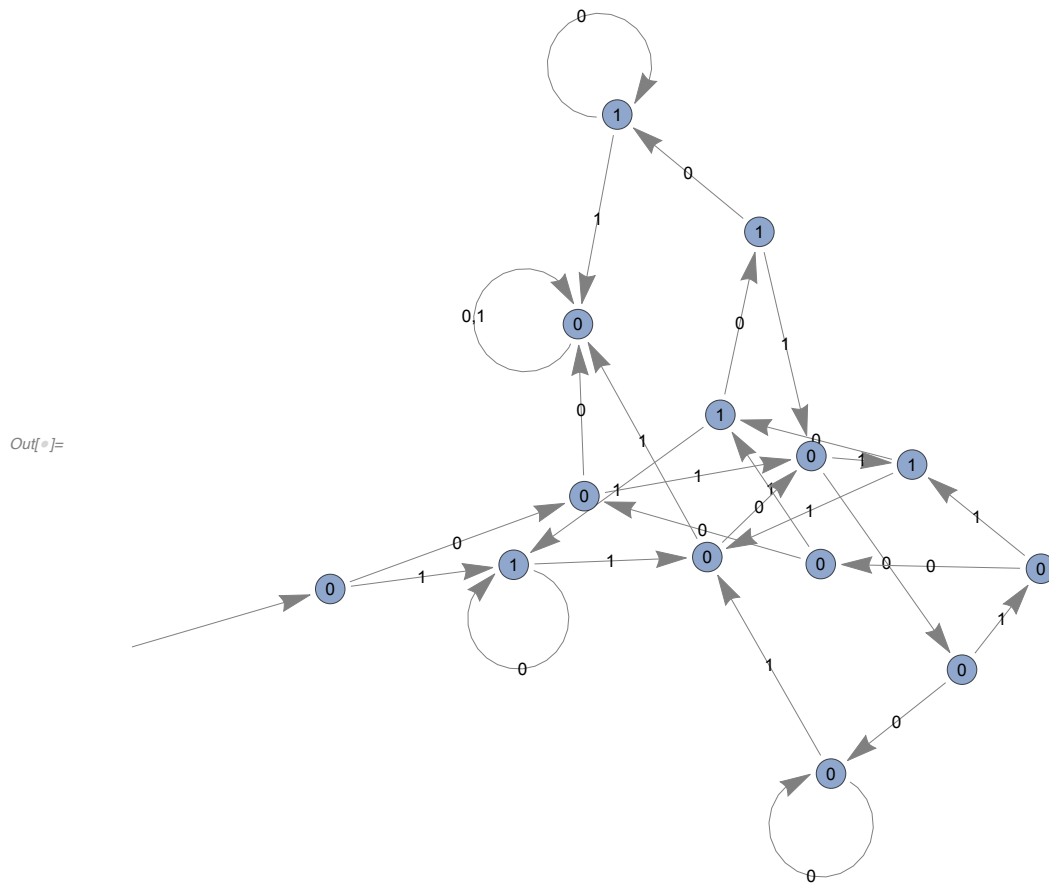

Break sequence ( $m = 2^\mu - 1$ )

$\sigma_{S,1}$

```
fsigmaS1[t_, s_] := t^2 s^2 + t s + s + t
```

```
initsigmaS1[t_] := t + t^2 + t^3 + 0[t]^5
```

```

automatonsigmaS1 = AutomaticSequenceAutomaton[AutomaticSequenceReduce[
  AlgebraicSequence[SeriesRoot[{Function[s, fsigmaS1[t, s]], initsigmaS1[t]],
    Modulus → 2]][n], n, Method → "Diagonal"]

```

```

Out[ ]= Automaton[{{1 → 2, 0}, {1 → 3, 1}, {2 → 4, 0}, {2 → 3, 1},
  {4 → 4, 0}, {4 → 4, 1}, {3 → 5, 0}, {3 → 3, 1}, {5 → 5, 0}, {5 → 4, 1}},
  1, {1 → 0, 2 → 0, 3 → 1, 4 → 0, 5 → 1}, InputAlphabet → {0, 1}]

```

```

edge[x_, ___] := {Arrowheads[0.080], Arrow[x, 0.1]}
AutomatonGraph[automatonsigmaS1, VertexSize -> 0.3, EdgeShapeFunction -> edge]

```

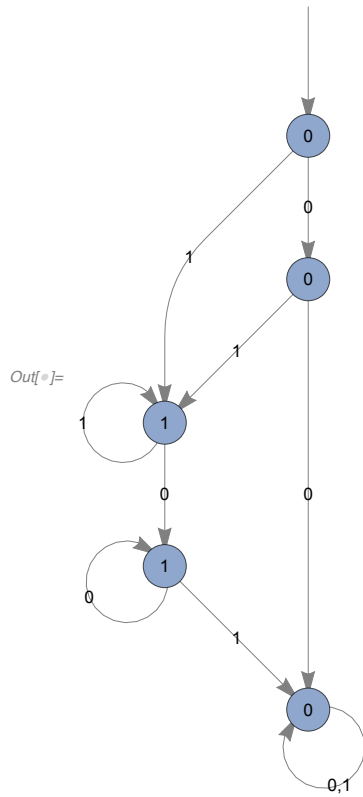

$\sigma_{S,m} (m \geq 2)$

The automaton below corresponds to the case  $\mu = 5, m = 31$ .

```

fsigmaSm[t_, s_] := (t s) ^ 16 + s + t
initsigmaSm[t_] := t + 0[t] ^ 5
automatonsigmaSm = AutomaticSequenceAutomaton[AutomaticSequenceReduce[
  AlgebraicSequence[SeriesRoot[{Function[s, fsigmaSm[t, s]], initsigmaSm[t]],
    Modulus -> 2]][n], n, Method -> "Diagonal"]

```

```

Out[ ]:= Automaton[{{1 -> 2, 0}, {1 -> 3, 1}, {4 -> 5, 0}, {4 -> 3, 1},
  {2 -> 6, 0}, {2 -> 5, 1}, {5 -> 5, 0}, {5 -> 5, 1}, {6 -> 7, 0}, {6 -> 5, 1},
  {7 -> 8, 0}, {7 -> 5, 1}, {8 -> 4, 0}, {8 -> 2, 1}, {3 -> 3, 0}, {3 -> 5, 1}}, 1,
  {1 -> 0, 2 -> 0, 3 -> 1, 4 -> 0, 5 -> 0, 6 -> 0, 7 -> 0, 8 -> 0}, InputAlphabet -> {0, 1}]

```

```
edge[x_, ___] := {Arrowheads[0.030], Arrow[x, 0.1]}
AutomatonGraph[automatonsigmaSm, VertexSize -> 0.3, EdgeShapeFunction -> edge]
```

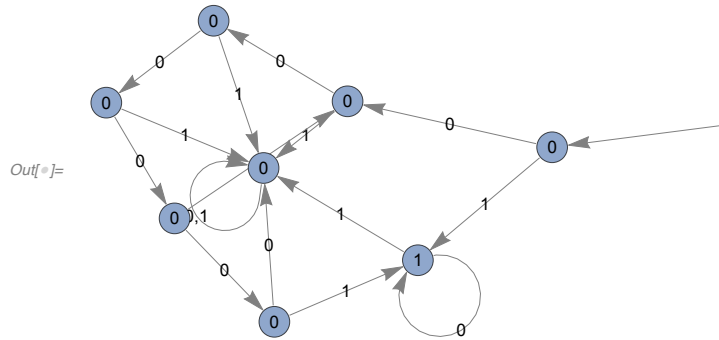

## Order 4 elements

### Break sequence (1, 3)

$\sigma_{\min}$

```
In[*]:= fsgmamin[t_, s_] := (t+1)^3 s^3 + (t^3+t) s^2 + (t^3+t+1) s + t^3+t
initsgmamin[t_] := t + t^2 + t^4 + t^5 + 0[t]^6
automatonsigmamin =
AutomaticSequenceAutomaton[AutomaticSequenceReduce[
  AlgebraicSequence[SeriesRoot[{Function[s, fsgmamin[t, s]],
    initsgmamin[t]], Modulus -> 2]][n], n, Method -> "Diagonal"]]
```

Out[\*]= Automaton[{{1 -> 1, 0}, {1 -> 2, 1}, {3 -> 3, 0}, {3 -> 4, 1},  
 {2 -> 5, 0}, {2 -> 3, 1}, {5 -> 5, 0}, {5 -> 2, 1}, {4 -> 2, 0}, {4 -> 4, 1}},  
 1, {1 -> 0, 2 -> 1, 3 -> 0, 4 -> 1, 5 -> 1}, InputAlphabet -> {0, 1}]

```
In[*]:= edge[x_, ___] := {Arrowheads[0.040], Arrow[x, 0.1]}
AutomatonGraph[automatonsigmamin, VertexSize -> 0.3, EdgeShapeFunction -> edge]
```

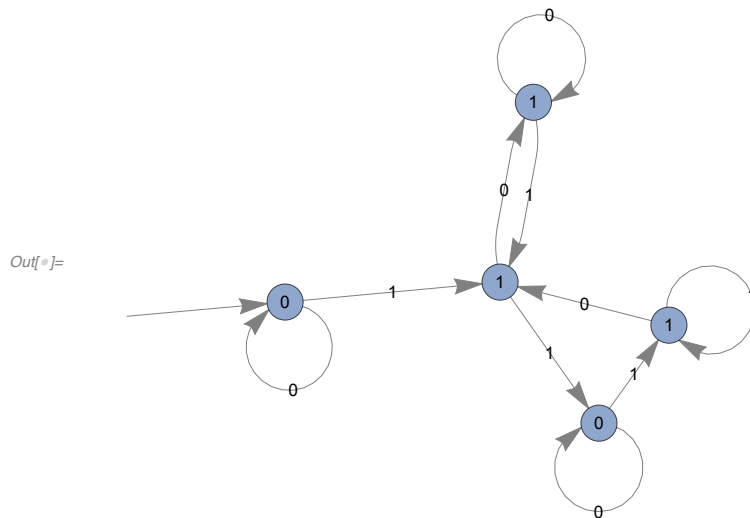

$\sigma_{CS}$ 

```

In[ ]:= fsigmaCS[t_, s_] := (t^2 + 1) s^2 + s + t
        initsigmaCS[t_] := t + t^2 + 0[t]^5
        automatsigmaCS = AutomaticSequenceAutomaton[AutomaticSequenceReduce[
            AlgebraicSequence[SeriesRoot[{Function[s, fsigmaCS[t, s]], initsigmaCS[t]],
            Modulus -> 2]][n], n, Method -> "Diagonal"]

```

```

Out[ ]:= Automaton[
    {{1 -> 2, 0}, {1 -> 3, 1}, {2 -> 4, 0}, {2 -> 5, 1}, {4 -> 4, 0}, {4 -> 2, 1}, {6 -> 6, 0},
    {6 -> 6, 1}, {3 -> 3, 0}, {3 -> 6, 1}, {7 -> 7, 0}, {7 -> 2, 1}, {5 -> 7, 0}, {5 -> 5, 1}},
    1, {1 -> 0, 2 -> 0, 3 -> 1, 4 -> 0, 5 -> 1, 6 -> 0, 7 -> 1}, InputAlphabet -> {0, 1}]

```

```

In[ ]:= edge[x_, ___] := {Arrowheads[0.040], Arrow[x, 0.1]}
        AutomatonGraph[automatsigmaCS, VertexSize -> 0.3, EdgeShapeFunction -> edge]

```

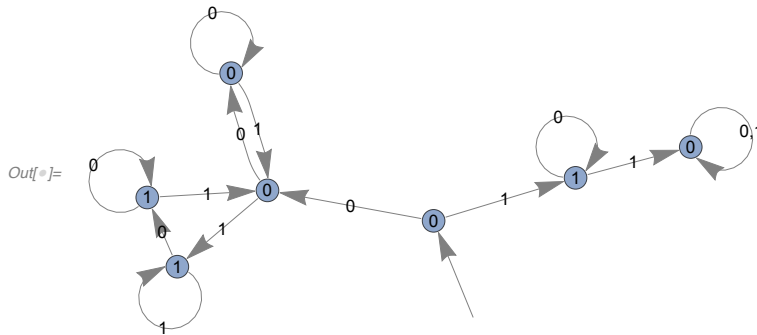 $\sigma_{CS}^{03}$ 

```

In[ ]:= fsigmaCS3[t_, s_] := t^2 s^2 + s + t^2 + t
        initsigmaCS3[t_] := t + t^2 + t^4 + 0[t]^5
        automatsigmaCS3 =
            AutomaticSequenceAutomaton[AutomaticSequenceReduce[AlgebraicSequence[
                SeriesRoot[{Function[s, fsigmaCS3[t, s]], initsigmaCS3[t]], Modulus -> 2]][
                n], n, Method -> "Diagonal"]

```

```

Out[ ]:= Automaton[
    {{1 -> 2, 0}, {1 -> 3, 1}, {2 -> 4, 0}, {2 -> 5, 1}, {4 -> 6, 0}, {4 -> 3, 1}, {6 -> 6, 0},
    {6 -> 6, 1}, {3 -> 3, 0}, {3 -> 6, 1}, {5 -> 7, 0}, {5 -> 5, 1}, {7 -> 3, 0}, {7 -> 3, 1}},
    1, {1 -> 0, 2 -> 0, 3 -> 1, 4 -> 0, 5 -> 1, 6 -> 0, 7 -> 1}, InputAlphabet -> {0, 1}]

```



```

In[ ]:= edge[x_, ___] := {Arrowheads[0.060], Arrow[x, 0.1]}
AutomatonGraph[automatonsigmaCS3, VertexSize -> 0.3, EdgeShapeFunction -> edge]

```

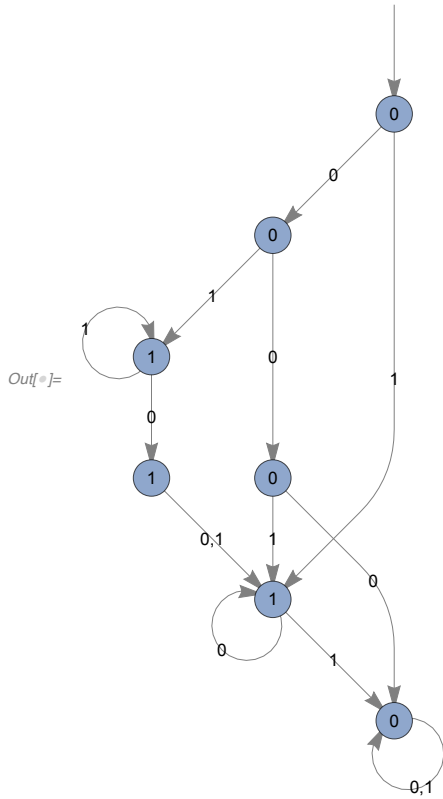

$\sigma_J$

```

In[ ]:= fsigmaJ[t_, s_] := (t+1) s^2 + (t^2+1) s + t
initsigmaJ[t_] := t + t^2 + 0[t]^5
automatonsigmaJ = AutomaticSequenceAutomaton[AutomaticSequenceReduce[
  AlgebraicSequence[SeriesRoot[{Function[s, fsigmaJ[t, s]], initsigmaJ[t]],
    Modulus -> 2]][n], n, Method -> "Diagonal"]]
Out[ ]:= Automaton[{{1 -> 2, 0}, {1 -> 3, 1}, {2 -> 4, 0}, {2 -> 5, 1}, {6 -> 7, 0}, {6 -> 8, 1},
  {4 -> 4, 0}, {4 -> 6, 1}, {7 -> 7, 0}, {7 -> 7, 1}, {3 -> 9, 0}, {3 -> 6, 1},
  {5 -> 8, 0}, {5 -> 7, 1}, {9 -> 9, 0}, {9 -> 5, 1}, {8 -> 8, 0}, {8 -> 8, 1}}, 1,
  {1 -> 0, 2 -> 0, 3 -> 1, 4 -> 0, 5 -> 1, 6 -> 0, 7 -> 0, 8 -> 1, 9 -> 1}, InputAlphabet -> {0, 1}]

```

```

In[ ]:= edge[x_, ___] := {Arrowheads[0.060], Arrow[x, 0.1]}
AutomatonGraph[automatonsigmaJ, VertexSize → 0.3, EdgeShapeFunction → edge]

```

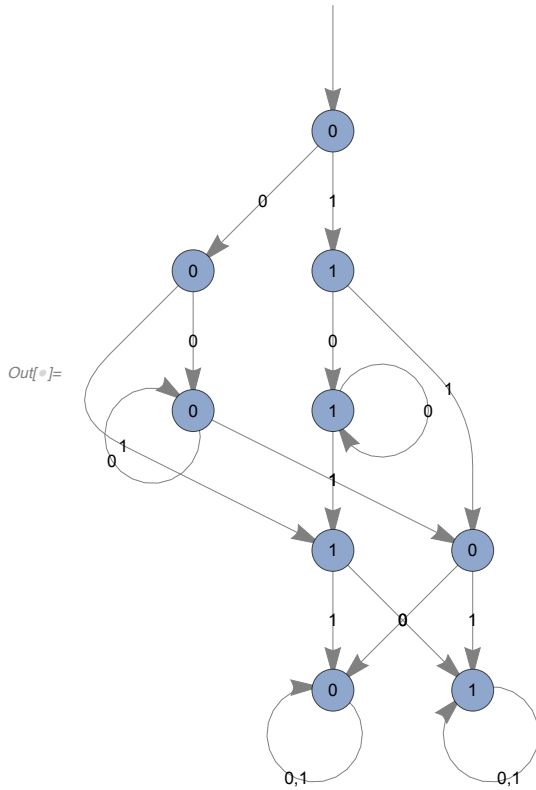

$\sigma_J^{03}$

```

In[ ]:= fsigmaJ3[t_, s_] := t s^2 + (t^2 + 1) s + t^2 + t
initsigmaJ3[t_] := t + t^2 + t^4 + 0[t]^5
automatonsigmaJ3 = AutomaticSequenceAutomaton[AutomaticSequenceReduce[
  AlgebraicSequence[SeriesRoot[{Function[s, fsigmaJ3[t, s]], initsigmaJ3[t]],
    Modulus → 2]][n], n, Method → "Diagonal"]

```

```

Out[ ]:= Automaton[{{1 → 2, 0}, {1 → 3, 1}, {2 → 2, 0}, {2 → 4, 1}, {5 → 6, 0},
  {5 → 7, 1}, {6 → 8, 0}, {6 → 4, 1}, {8 → 8, 0}, {8 → 8, 1}, {3 → 9, 0},
  {3 → 5, 1}, {10 → 10, 0}, {10 → 6, 1}, {11 → 4, 0}, {11 → 8, 1}, {4 → 4, 0},
  {4 → 4, 1}, {9 → 10, 0}, {9 → 11, 1}, {7 → 11, 0}, {7 → 7, 1}}, 1,
  {1 → 0, 2 → 0, 3 → 1, 4 → 1, 5 → 0, 6 → 0, 7 → 1, 8 → 0, 9 → 1, 10 → 1, 11 → 1},
  InputAlphabet → {0, 1}]

```

```
In[*]:= edge[x_, ___] := {Arrowheads[0.060], Arrow[x, 0.1]}
AutomatonGraph[automatonsigmaJ3, VertexSize -> 0.3, EdgeShapeFunction -> edge]
```

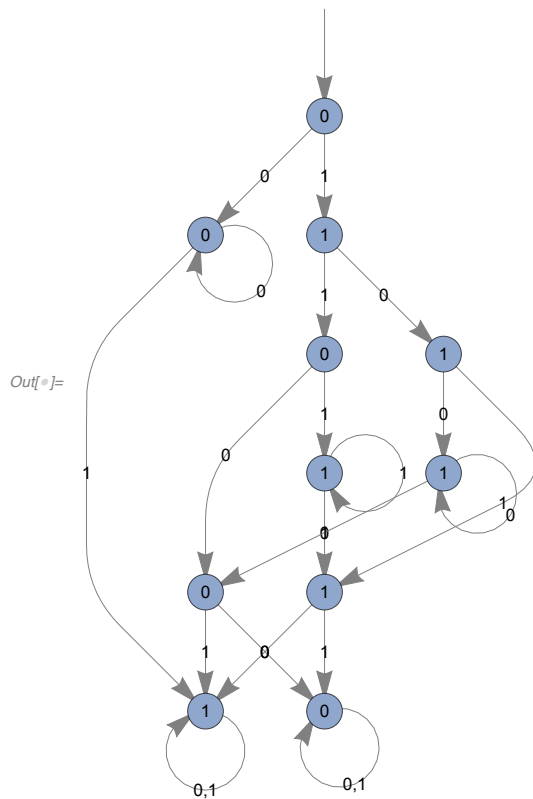 $\sigma_{T,1}$ 
$$\text{fsigmaT1}[t\_ , s\_ ] := t^2 s^4 + (t^4 + t^2 + t + 1) s^2 + (t^3 + t^2 + t) s + t^3$$
$$\text{initsigmaT1}[t_] := t + t^2 + 0[t]^5$$

```

automatonsigmaT1 = AutomaticSequenceAutomaton[AutomaticSequenceReduce[
  AlgebraicSequence[SeriesRoot[{Function[s, fsigmaT1[t, s] ], initsigmaT1[t] },
    Modulus -> 2]] [n] , n, Method -> "Diagonal"]

```

*Out[\*]=* Automaton[{{1 → 2, 0}, {1 → 3, 1}, {2 → 4, 0}, {2 → 5, 1}, {6 → 2, 0}, {6 → 5, 1},  
{4 → 4, 0}, {4 → 4, 1}, {3 → 7, 0}, {3 → 6, 1}, {8 → 8, 0}, {8 → 4, 1},  
{9 → 5, 0}, {9 → 4, 1}, {5 → 8, 0}, {5 → 5, 1}, {7 → 7, 0}, {7 → 9, 1}}, 1,  
{1 → 0, 2 → 0, 3 → 1, 4 → 0, 5 → 1, 6 → 0, 7 → 1, 8 → 1, 9 → 1}, InputAlphabet → {0, 1}]

```

edge[x_, ___] := {Arrowheads[0.080], Arrow[x, 0.1]}
AutomatonGraph[automatonsigmaT1, VertexSize -> 0.3, EdgeShapeFunction -> edge]

```

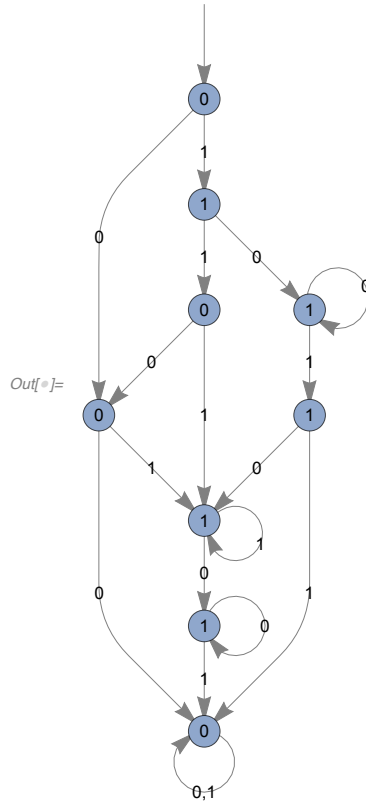

$\sigma_{T,2}$

```

fsigmaT2[t_, s_] := t^2 s^4 + (t+1) s^3 + (t^4 + t^2 + t) s^2 + (t^2 + t) s + t^2

```

```

initsigmaT2[t_] := t + t^2 + t^4 + t^5 + 0[t]^7

```

```

automatonsigmaT2 = AutomaticSequenceAutomaton[AutomaticSequenceReduce[
  AlgebraicSequence[SeriesRoot[{Function[s, fsigmaT2[t, s]], initsigmaT2[t]],
    Modulus -> 2]][n], n, Method -> "Diagonal"]]

```

```

Out[ ]:= Automaton[{{1 -> 2, 0}, {1 -> 3, 1}, {2 -> 4, 0}, {2 -> 5, 1}, {6 -> 6, 0},
  {6 -> 7, 1}, {4 -> 8, 0}, {4 -> 9, 1}, {10 -> 11, 0}, {10 -> 12, 1}, {13 -> 4, 0},
  {13 -> 9, 1}, {8 -> 8, 0}, {8 -> 8, 1}, {14 -> 6, 0}, {14 -> 14, 1}, {11 -> 6, 0},
  {11 -> 13, 1}, {3 -> 9, 0}, {3 -> 10, 1}, {15 -> 16, 0}, {15 -> 13, 1}, {5 -> 15, 0},
  {5 -> 14, 1}, {17 -> 17, 0}, {17 -> 8, 1}, {7 -> 9, 0}, {7 -> 8, 1}, {9 -> 17, 0},
  {9 -> 9, 1}, {12 -> 16, 0}, {12 -> 12, 1}, {16 -> 16, 0}, {16 -> 7, 1}}, 1,
{1 -> 0, 2 -> 0, 3 -> 1, 4 -> 0, 5 -> 1, 6 -> 0, 7 -> 1, 8 -> 0, 9 -> 1, 10 -> 0, 11 -> 0,
  12 -> 1, 13 -> 0, 14 -> 0, 15 -> 1, 16 -> 1, 17 -> 1}], InputAlphabet -> {0, 1}]

```

```

edge[x_, ___] := {Arrowheads[0.060], Arrow[x, 0.1]}
AutomatonGraph[automatonsigmaT2, VertexSize -> 0.3, EdgeShapeFunction -> edge]

```

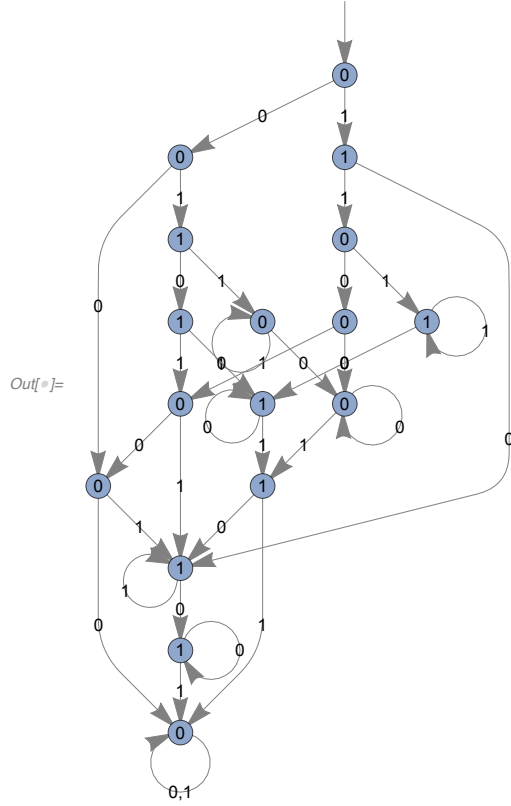

$\sigma_{T,3}$

```

fsigmaT3[t_, s_] := t^4 s^4 + (t^2 + 1) s^3 + (t^3 + t) s^2 + t^2 s + t^3
initsigmaT3[t_] := t + t^2 + t^6 + t^8 + t^10 + 0[t]^13
automatonsigmaT3 = AutomaticSequenceAutomaton[
  AutomaticSequenceReduce[AlgebraicSequence[SeriesRoot[
    Function[s, fsigmaT3[t, s]], initsigmaT3[t]], Modulus -> 2]][n], n]]

```

Out["]= Automaton[{{1 -> 2, 0}, {1 -> 3, 1}, {4 -> 4, 0}, {4 -> 3, 1}, {2 -> 5, 0},  
 {2 -> 6, 1}, {7 -> 8, 0}, {7 -> 9, 1}, {10 -> 11, 0}, {10 -> 3, 1}, {12 -> 7, 0},  
 {12 -> 6, 1}, {13 -> 13, 0}, {13 -> 9, 1}, {5 -> 10, 0}, {5 -> 14, 1}, {11 -> 11, 0},  
 {11 -> 11, 1}, {14 -> 15, 0}, {14 -> 12, 1}, {8 -> 8, 0}, {8 -> 4, 1}, {15 -> 13, 0},  
 {15 -> 4, 1}, {3 -> 3, 0}, {3 -> 11, 1}, {16 -> 16, 0}, {16 -> 4, 1}, {6 -> 17, 0},  
 {6 -> 6, 1}, {17 -> 16, 0}, {17 -> 9, 1}, {9 -> 9, 0}, {9 -> 3, 1}}, 1,  
 {1 -> 0, 2 -> 0, 3 -> 1, 4 -> 0, 5 -> 0, 6 -> 1, 7 -> 0, 8 -> 0, 9 -> 1, 10 -> 0, 11 -> 0,  
 12 -> 0, 13 -> 0, 14 -> 0, 15 -> 0, 16 -> 1, 17 -> 1}, InputAlphabet -> {0, 1}]

```
edge[x_, ___] := {Arrowheads[0.050], Arrow[x, 0.1]}
```

```
AutomatonGraph[automatonsigmaT3, VertexSize -> 0.3, EdgeShapeFunction -> edge]
```

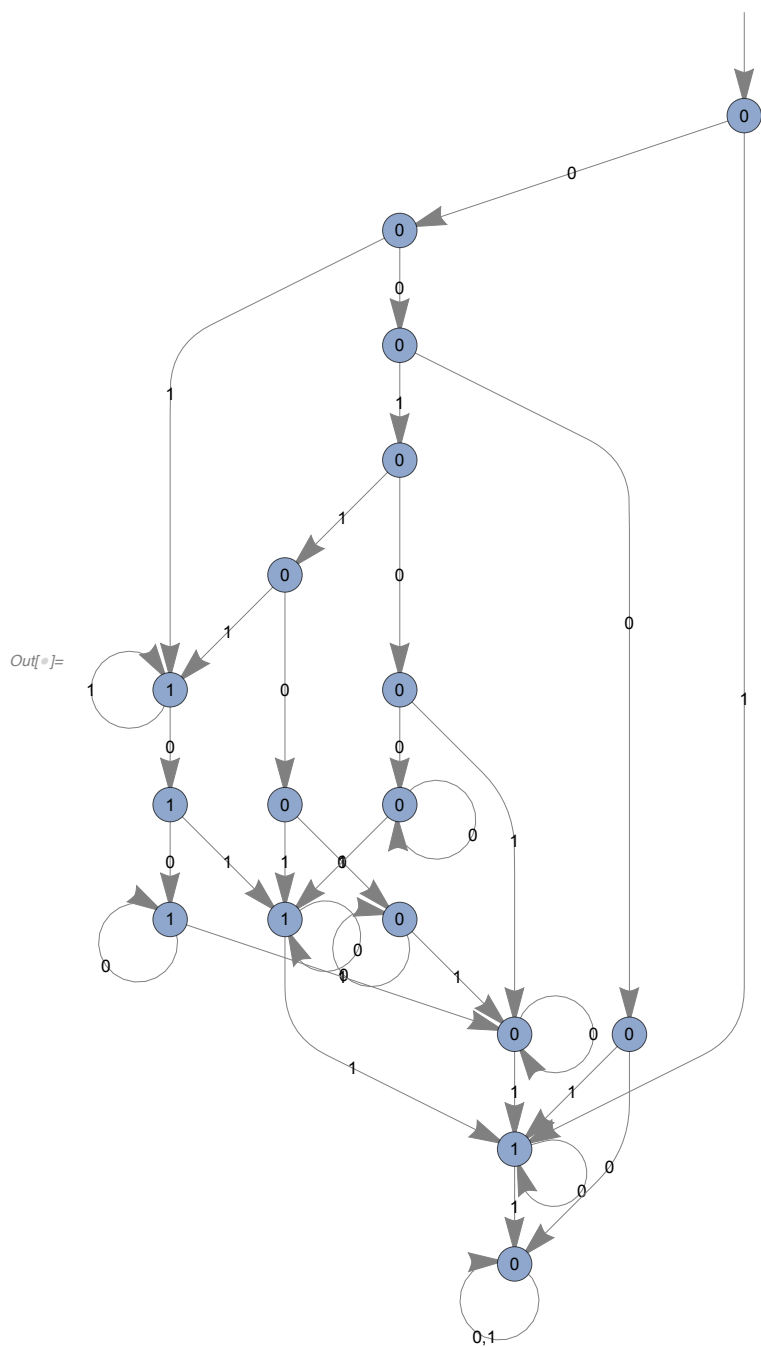

$\sigma_{T,4}$ 

```

fsigmaT4[t_, s_] := t^4 s^4 + (t^2 + 1) s^3 + (t^3 + t) s^2 + t^2 s + t^3
initsigmaT4[t_] := t + t^2 + t^4 + t^6 + t^8 + 0[t]^13
automatonsigmaT4 = AutomaticSequenceAutomaton[
  AutomaticSequenceReduce[AlgebraicSequence[SeriesRoot[
    {Function[s, fsigmaT4[t, s]], initsigmaT4[t]], Modulus -> 2]][n], n]]

```

```

Out[8]= Automaton[{{1 -> 2, 0}, {1 -> 3, 1}, {4 -> 5, 0}, {4 -> 6, 1}, {7 -> 7, 0},
  {7 -> 3, 1}, {2 -> 4, 0}, {2 -> 8, 1}, {9 -> 9, 0}, {9 -> 10, 1}, {5 -> 11, 0},
  {5 -> 3, 1}, {12 -> 13, 0}, {12 -> 8, 1}, {11 -> 11, 0}, {11 -> 11, 1}, {13 -> 9, 0},
  {13 -> 7, 1}, {3 -> 3, 0}, {3 -> 11, 1}, {6 -> 14, 0}, {6 -> 12, 1}, {15 -> 16, 0},
  {15 -> 7, 1}, {17 -> 17, 0}, {17 -> 7, 1}, {8 -> 15, 0}, {8 -> 8, 1}, {14 -> 17, 0},
  {14 -> 10, 1}, {16 -> 16, 0}, {16 -> 10, 1}, {10 -> 10, 0}, {10 -> 3, 1}}, 1,
  {1 -> 0, 2 -> 0, 3 -> 1, 4 -> 0, 5 -> 0, 6 -> 1, 7 -> 0, 8 -> 1, 9 -> 0, 10 -> 1, 11 -> 0,
  12 -> 0, 13 -> 0, 14 -> 1, 15 -> 1, 16 -> 1, 17 -> 1}, InputAlphabet -> {0, 1}]

```

```
edge[x_, ___] := {Arrowheads[0.050], Arrow[x, 0.1]}
```

```
AutomatonGraph[automatonsigmaT4, VertexSize -> 0.3, EdgeShapeFunction -> edge]
```

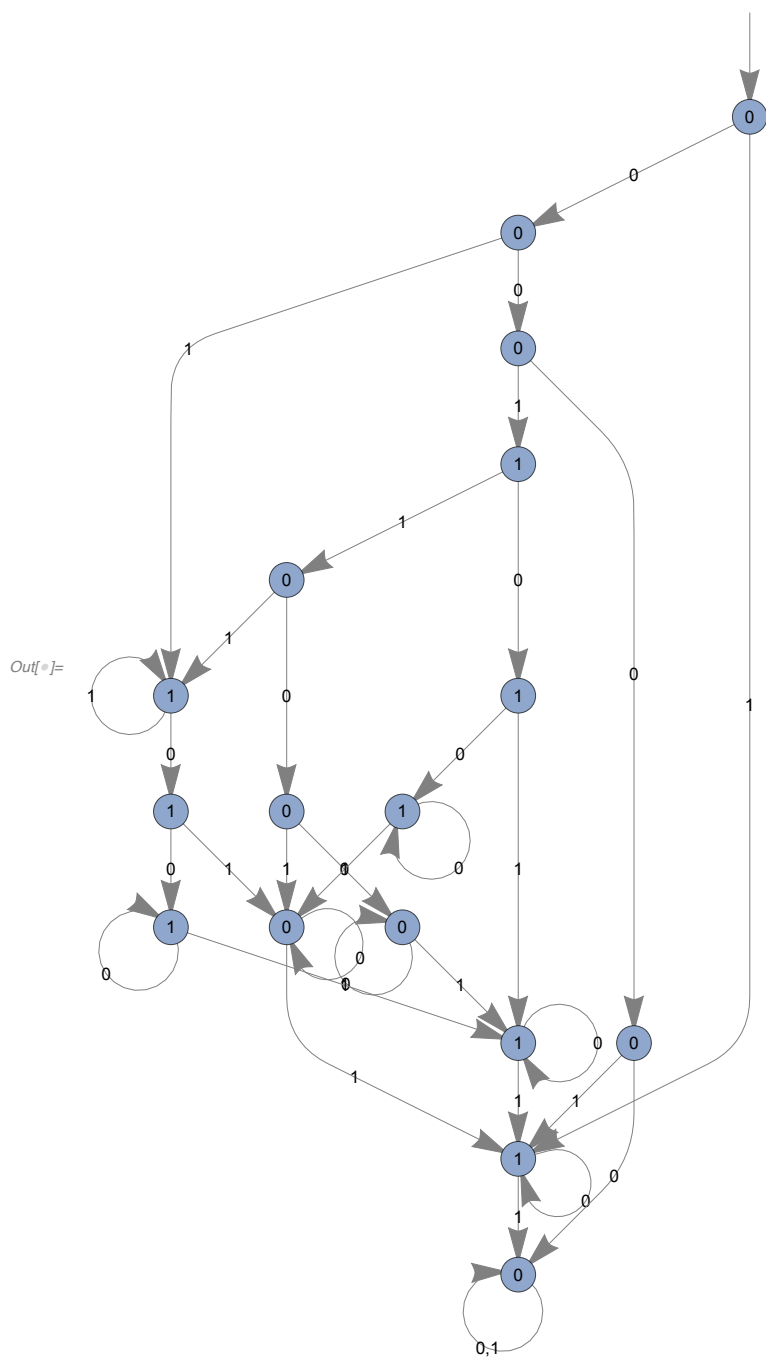



## Break sequence (1, 5)

$\sigma_{(1,5)}$

```
In[ ]:= fsigma15[t_, s_] := t^2 s^3 + (t+1)^3 s + t^3 + t
initsigma15[t_] := t + t^2 + t^3 + t^4 + t^6 + 0[t]^7
automatonsigma15 = AutomaticSequenceAutomaton[AutomaticSequenceReduce[
  AlgebraicSequence[SeriesRoot[{Function[s, fsigma15[t, s]], initsigma15[t]],
    Modulus -> 2]][n], n, Method -> "Diagonal"]]
```

```
Out[ ]:= Automaton[{{1 -> 1, 0}, {1 -> 2, 1}, {3 -> 4, 0}, {3 -> 5, 1},
  {4 -> 6, 0}, {4 -> 7, 1}, {8 -> 6, 0}, {8 -> 5, 1}, {9 -> 8, 0}, {9 -> 10, 1},
  {10 -> 10, 0}, {10 -> 10, 1}, {6 -> 10, 0}, {6 -> 8, 1}, {2 -> 11, 0},
  {2 -> 12, 1}, {5 -> 11, 0}, {5 -> 13, 1}, {13 -> 2, 0}, {13 -> 13, 1},
  {11 -> 7, 0}, {11 -> 3, 1}, {12 -> 5, 0}, {12 -> 9, 1}, {7 -> 7, 0}, {7 -> 9, 1}},
  1, {1 -> 0, 2 -> 1, 3 -> 0, 4 -> 0, 5 -> 1, 6 -> 0, 7 -> 1, 8 -> 0, 9 -> 0,
  10 -> 0, 11 -> 1, 12 -> 1, 13 -> 1}, InputAlphabet -> {0, 1}]
```

```
In[ ]:= edge[x_, ___] := {Arrowheads[0.030], Arrow[x, 0.1]}
AutomatonGraph[automatonsigma15, VertexSize -> 0.3, EdgeShapeFunction -> edge]
```

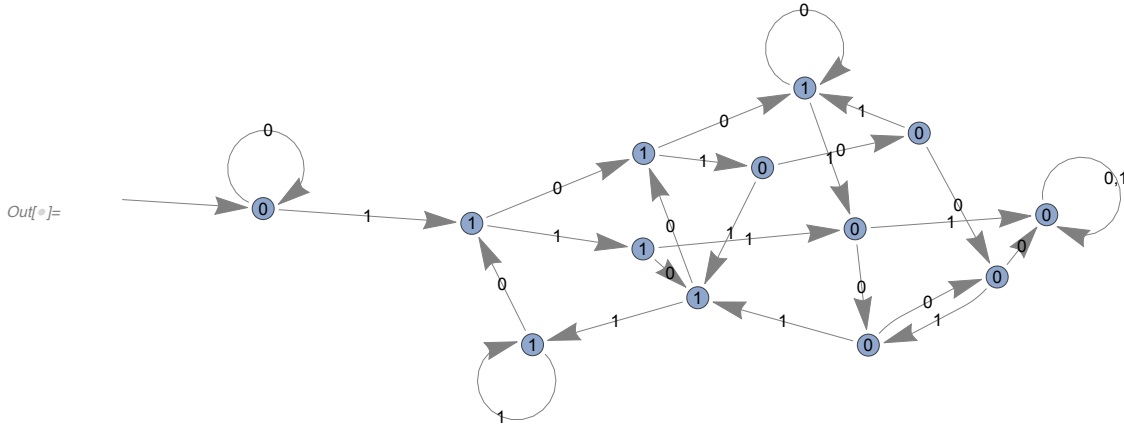

## Break sequence (1, 9)

$\sigma_{(1,9)}$

```
In[ ]:= fsigma19[t_, s_] := t^2 s^7 + t^3 s^6 + (t^5 + t^4 + t^2) s^5 +
  (t^5 + t^3) s^4 + (t^7 + t^5 + t^4 + t^3 + t) s^3 + t^5 s^2 + (t^3 + t + 1) s + t
initsigma19[t_] := t + t^2 + t^3 + t^4 + t^5 + t^6 + t^7 +
  t^9 + t^11 + t^12 + t^13 + t^17 + t^18 + 0[t]^19
automatonsigma19 = AutomaticSequenceAutomaton[AutomaticSequenceReduce[
  AlgebraicSequence[SeriesRoot[{Function[s, fsigma19[t, s]], initsigma19[t]],
    Modulus -> 2]][n], n, Method -> "Diagonal"]]
```

```
Out[ ]:= Automaton[{{1 -> 2, 0}, {1 -> 3, 1}, {4 -> 5, 0}, {4 -> 6, 1}, {2 -> 7, 0}, {2 -> 8, 1},
  {9 -> 10, 0}, {9 -> 11, 1}, {5 -> 12, 0}, {5 -> 13, 1}, {14 -> 15, 0}, {14 -> 16, 1},
  {17 -> 18, 0}, {17 -> 19, 1}, {7 -> 20, 0}, {7 -> 16, 1}, {21 -> 22, 0}, {21 -> 23, 1}},
  1, {1 -> 0, 2 -> 1, 3 -> 0, 4 -> 0, 5 -> 1, 6 -> 0, 7 -> 1, 8 -> 0, 9 -> 0,
  10 -> 0, 11 -> 1, 12 -> 1, 13 -> 1, 14 -> 0, 15 -> 0, 16 -> 1, 17 -> 0, 18 -> 0,
  19 -> 0, 20 -> 0, 21 -> 0, 22 -> 0, 23 -> 0}, InputAlphabet -> {0, 1}]
```

```

{24 → 20, 0}, {24 → 25, 1}, {26 → 27, 0}, {26 → 6, 1}, {28 → 29, 0}, {28 → 19, 1},
{18 → 30, 0}, {18 → 13, 1}, {31 → 22, 0}, {31 → 32, 1}, {33 → 34, 0}, {33 → 11, 1},
{35 → 7, 0}, {35 → 36, 1}, {10 → 24, 0}, {10 → 37, 1}, {38 → 7, 0}, {38 → 39, 1},
{12 → 24, 0}, {12 → 40, 1}, {41 → 42, 0}, {41 → 36, 1}, {43 → 22, 0}, {43 → 36, 1},
{15 → 20, 0}, {15 → 37, 1}, {44 → 45, 0}, {44 → 46, 1}, {47 → 22, 0}, {47 → 39, 1},
{42 → 20, 0}, {42 → 40, 1}, {20 → 48, 0}, {20 → 49, 1}, {48 → 50, 0}, {48 → 51, 1},
{52 → 53, 0}, {52 → 54, 1}, {55 → 49, 0}, {55 → 56, 1}, {50 → 50, 0}, {50 → 50, 1},
{57 → 58, 0}, {57 → 57, 1}, {54 → 59, 0}, {54 → 57, 1}, {56 → 51, 0}, {56 → 50, 1},
{22 → 48, 0}, {22 → 60, 1}, {61 → 60, 0}, {61 → 56, 1}, {58 → 62, 0}, {58 → 54, 1},
{63 → 30, 0}, {63 → 54, 1}, {49 → 35, 0}, {49 → 54, 1}, {64 → 43, 0}, {64 → 50, 1},
{53 → 21, 0}, {53 → 50, 1}, {65 → 21, 0}, {65 → 51, 1}, {45 → 31, 0}, {45 → 60, 1},
{34 → 31, 0}, {34 → 49, 1}, {51 → 48, 0}, {51 → 9, 1}, {59 → 66, 0}, {59 → 4, 1},
{67 → 65, 0}, {67 → 4, 1}, {29 → 62, 0}, {29 → 28, 1}, {66 → 21, 0}, {66 → 7, 1},
{60 → 38, 0}, {60 → 4, 1}, {62 → 21, 0}, {62 → 43, 1}, {27 → 35, 0}, {27 → 28, 1},
{68 → 47, 0}, {68 → 9, 1}, {30 → 31, 0}, {30 → 9, 1}, {3 → 3, 0}, {3 → 69, 1},
{70 → 70, 0}, {70 → 71, 1}, {16 → 8, 0}, {16 → 72, 1}, {19 → 73, 0}, {19 → 74, 1},
{72 → 75, 0}, {72 → 76, 1}, {77 → 70, 0}, {77 → 78, 1}, {74 → 79, 0}, {74 → 78, 1},
{79 → 77, 0}, {79 → 80, 1}, {75 → 81, 0}, {75 → 82, 1}, {76 → 69, 0}, {76 → 76, 1},
{78 → 83, 0}, {78 → 78, 1}, {11 → 84, 0}, {11 → 74, 1}, {6 → 85, 0}, {6 → 72, 1},
{86 → 77, 0}, {86 → 87, 1}, {8 → 88, 0}, {8 → 89, 1}, {81 → 88, 0}, {81 → 90, 1},
{23 → 91, 0}, {23 → 92, 1}, {87 → 93, 0}, {87 → 94, 1}, {95 → 91, 0}, {95 → 96, 1},
{73 → 97, 0}, {73 → 98, 1}, {69 → 8, 0}, {69 → 98, 1}, {99 → 77, 0}, {99 → 92, 1},
{71 → 100, 0}, {71 → 92, 1}, {83 → 70, 0}, {83 → 89, 1}, {101 → 77, 0},
{101 → 96, 1}, {100 → 70, 0}, {100 → 90, 1}, {25 → 81, 0}, {25 → 94, 1},
{80 → 102, 0}, {80 → 72, 1}, {82 → 103, 0}, {82 → 74, 1}, {84 → 39, 0}, {84 → 82, 1},
{13 → 104, 0}, {13 → 76, 1}, {85 → 91, 0}, {85 → 80, 1}, {32 → 88, 0}, {32 → 78, 1},
{88 → 79, 0}, {88 → 64, 1}, {89 → 99, 0}, {89 → 52, 1}, {98 → 16, 0}, {98 → 55, 1},
{105 → 86, 0}, {105 → 52, 1}, {106 → 86, 0}, {106 → 67, 1}, {37 → 23, 0},
{37 → 61, 1}, {91 → 79, 0}, {91 → 68, 1}, {92 → 36, 0}, {92 → 61, 1}, {36 → 105, 0},
{36 → 52, 1}, {102 → 106, 0}, {102 → 64, 1}, {94 → 107, 0}, {94 → 63, 1},
{93 → 106, 0}, {93 → 68, 1}, {108 → 105, 0}, {108 → 67, 1}, {46 → 40, 0},
{46 → 55, 1}, {90 → 101, 0}, {90 → 14, 1}, {40 → 95, 0}, {40 → 17, 1}, {104 → 23, 0},
{104 → 26, 1}, {103 → 109, 0}, {103 → 26, 1}, {109 → 105, 0}, {109 → 44, 1},
{39 → 106, 0}, {39 → 14, 1}, {96 → 108, 0}, {96 → 17, 1}, {107 → 110, 0},
{107 → 17, 1}, {110 → 105, 0}, {110 → 33, 1}, {97 → 106, 0}, {97 → 41, 1}, 1,
{1 → 0, 2 → 0, 3 → 1, 4 → 0, 5 → 0, 6 → 1, 7 → 0, 8 → 1, 9 → 0, 10 → 0, 11 → 1, 12 → 0,
13 → 1, 14 → 0, 15 → 0, 16 → 1, 17 → 0, 18 → 0, 19 → 1, 20 → 0, 21 → 0, 22 → 0, 23 → 1,
24 → 0, 25 → 1, 26 → 0, 27 → 0, 28 → 0, 29 → 0, 30 → 0, 31 → 0, 32 → 1, 33 → 0, 34 → 0,
35 → 0, 36 → 1, 37 → 1, 38 → 0, 39 → 1, 40 → 1, 41 → 0, 42 → 0, 43 → 0, 44 → 0,
45 → 0, 46 → 1, 47 → 0, 48 → 0, 49 → 0, 50 → 0, 51 → 0, 52 → 0, 53 → 0, 54 → 0,
55 → 0, 56 → 0, 57 → 0, 58 → 0, 59 → 0, 60 → 0, 61 → 0, 62 → 0, 63 → 0, 64 → 0,
65 → 0, 66 → 0, 67 → 0, 68 → 0, 69 → 1, 70 → 1, 71 → 1, 72 → 1, 73 → 1, 74 → 1,
75 → 1, 76 → 1, 77 → 1, 78 → 1, 79 → 1, 80 → 1, 81 → 1, 82 → 1, 83 → 1, 84 → 1,
85 → 1, 86 → 1, 87 → 1, 88 → 1, 89 → 1, 90 → 1, 91 → 1, 92 → 1, 93 → 1, 94 → 1,
95 → 1, 96 → 1, 97 → 1, 98 → 1, 99 → 1, 100 → 1, 101 → 1, 102 → 1, 103 → 1, 104 → 1,
105 → 1, 106 → 1, 107 → 1, 108 → 1, 109 → 1, 110 → 1}, InputAlphabet → {0, 1}]

```

```

In[ ]:= edge[x_, ___] := {Arrowheads[0.015], Arrow[x, 0.1]}
AutomatonGraph[automatonsigma19, VertexSize → 0.3, EdgeShapeFunction → edge]

```

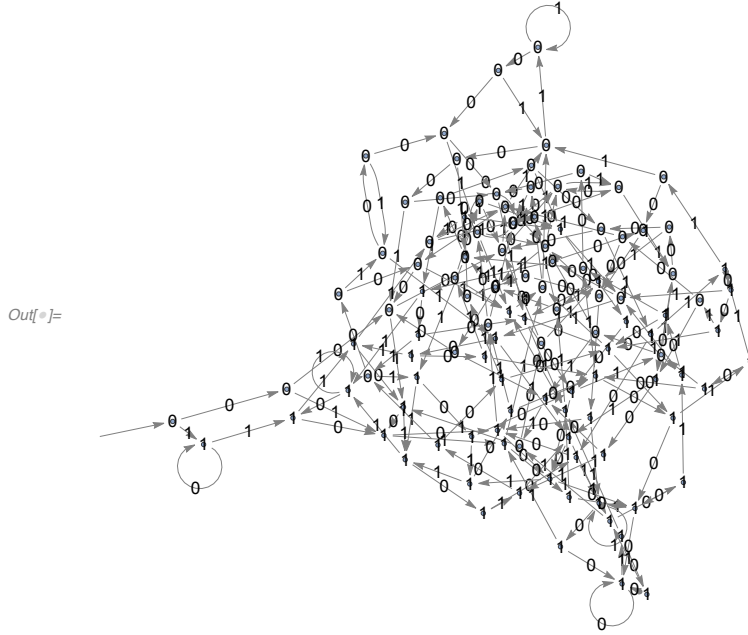

## Order 8 elements

Break sequence (1, 3, 11)

$\sigma_8$

```

In[ ]:= fsigma8[t_, s_] := t^6 s^6 + (t^6 + t^2) s^4 +
  (t^6 + t^5 + t^4 + t^3 + t^2 + 1) s^2 + (t + 1)^3 s + t^6 + t^5 + t^2 + t
initsigma8[t_] := t + t^2 + t^5 + t^6 + t^12 + 0[t]^13
automatonsigma8 = AutomaticSequenceAutomaton[AutomaticSequenceReduce[
  AlgebraicSequence[SeriesRoot[{Function[s, fsigma8[t, s]], initsigma8[t]],
    Modulus → 2]] [n], n, Method → "Diagonal"]

```

Out[ ]:= Automaton[{{1 → 2, 0}, {1 → 3, 1}, {4 → 5, 0}, {4 → 3, 1}, {6 → 7, 0}, {6 → 8, 1},  
 {9 → 10, 0}, {9 → 11, 1}, {12 → 13, 0}, {12 → 8, 1}, {14 → 15, 0}, {14 → 11, 1},  
 {16 → 17, 0}, {16 → 18, 1}, {19 → 20, 0}, {19 → 18, 1}, {21 → 22, 0}, {21 → 23, 1},  
 {24 → 25, 0}, {24 → 23, 1}, {26 → 9, 0}, {26 → 27, 1}, {28 → 24, 0}, {28 → 27, 1},  
 {29 → 30, 0}, {29 → 31, 1}, {32 → 32, 0}, {32 → 31, 1}, {33 → 32, 0}, {33 → 34, 1},  
 {35 → 33, 0}, {35 → 36, 1}, {37 → 33, 0}, {37 → 38, 1}, {39 → 40, 0}, {39 → 41, 1},  
 {42 → 43, 0}, {42 → 3, 1}, {30 → 44, 0}, {30 → 41, 1}, {45 → 46, 0}, {45 → 3, 1},  
 {47 → 35, 0}, {47 → 48, 1}, {49 → 37, 0}, {49 → 50, 1}, {51 → 35, 0}, {51 → 8, 1},  
 {52 → 37, 0}, {52 → 53, 1}, {54 → 55, 0}, {54 → 18, 1}, {56 → 57, 0}, {56 → 27, 1},  
 {2 → 58, 0}, {2 → 59, 1}, {22 → 60, 0}, {22 → 61, 1}, {62 → 63, 0}, {62 → 64, 1},  
 {5 → 65, 0}, {5 → 66, 1}, {67 → 65, 0}, {67 → 68, 1}, {69 → 70, 0}, {69 → 71, 1},  
 {25 → 70, 0}, {25 → 72, 1}, {73 → 74, 0}, {73 → 75, 1}, {17 → 76, 0}, {17 → 77, 1},  
 {20 → 78, 0}, {20 → 79, 1}, {80 → 81, 0}, {80 → 82, 1}, {83 → 81, 0}, {83 → 84, 1},

$\{85 \rightarrow 86, 0\}, \{85 \rightarrow 87, 1\}, \{88 \rightarrow 86, 0\}, \{88 \rightarrow 89, 1\}, \{90 \rightarrow 91, 0\}, \{90 \rightarrow 92, 1\},$   
 $\{93 \rightarrow 94, 0\}, \{93 \rightarrow 89, 1\}, \{95 \rightarrow 96, 0\}, \{95 \rightarrow 97, 1\}, \{98 \rightarrow 99, 0\}, \{98 \rightarrow 79, 1\},$   
 $\{55 \rightarrow 99, 0\}, \{55 \rightarrow 100, 1\}, \{44 \rightarrow 96, 0\}, \{44 \rightarrow 101, 1\}, \{102 \rightarrow 103, 0\},$   
 $\{102 \rightarrow 101, 1\}, \{104 \rightarrow 105, 0\}, \{104 \rightarrow 89, 1\}, \{106 \rightarrow 4, 0\}, \{106 \rightarrow 107, 1\},$   
 $\{108 \rightarrow 54, 0\}, \{108 \rightarrow 109, 1\}, \{40 \rightarrow 51, 0\}, \{40 \rightarrow 109, 1\}, \{110 \rightarrow 56, 0\},$   
 $\{110 \rightarrow 107, 1\}, \{94 \rightarrow 111, 0\}, \{94 \rightarrow 107, 1\}, \{112 \rightarrow 113, 0\}, \{112 \rightarrow 114, 1\},$   
 $\{43 \rightarrow 115, 0\}, \{43 \rightarrow 116, 1\}, \{117 \rightarrow 118, 0\}, \{117 \rightarrow 116, 1\}, \{119 \rightarrow 120, 0\},$   
 $\{119 \rightarrow 114, 1\}, \{121 \rightarrow 62, 0\}, \{121 \rightarrow 68, 1\}, \{122 \rightarrow 73, 0\}, \{122 \rightarrow 123, 1\},$   
 $\{46 \rightarrow 80, 0\}, \{46 \rightarrow 68, 1\}, \{124 \rightarrow 90, 0\}, \{124 \rightarrow 123, 1\}, \{96 \rightarrow 125, 0\},$   
 $\{96 \rightarrow 123, 1\}, \{125 \rightarrow 126, 0\}, \{125 \rightarrow 127, 1\}, \{126 \rightarrow 126, 0\}, \{126 \rightarrow 75, 1\},$   
 $\{99 \rightarrow 125, 0\}, \{99 \rightarrow 128, 1\}, \{103 \rightarrow 52, 0\}, \{103 \rightarrow 114, 1\}, \{105 \rightarrow 85, 0\},$   
 $\{105 \rightarrow 89, 1\}, \{111 \rightarrow 129, 0\}, \{111 \rightarrow 130, 1\}, \{115 \rightarrow 131, 0\}, \{115 \rightarrow 132, 1\},$   
 $\{133 \rightarrow 131, 0\}, \{133 \rightarrow 134, 1\}, \{135 \rightarrow 129, 0\}, \{135 \rightarrow 27, 1\}, \{7 \rightarrow 136, 0\},$   
 $\{7 \rightarrow 137, 1\}, \{113 \rightarrow 138, 0\}, \{113 \rightarrow 139, 1\}, \{10 \rightarrow 140, 0\}, \{10 \rightarrow 141, 1\},$   
 $\{57 \rightarrow 142, 0\}, \{57 \rightarrow 143, 1\}, \{144 \rightarrow 140, 0\}, \{144 \rightarrow 145, 1\}, \{146 \rightarrow 142, 0\},$   
 $\{146 \rightarrow 11, 1\}, \{13 \rightarrow 147, 0\}, \{13 \rightarrow 38, 1\}, \{118 \rightarrow 148, 0\}, \{118 \rightarrow 149, 1\},$   
 $\{120 \rightarrow 150, 0\}, \{120 \rightarrow 50, 1\}, \{15 \rightarrow 151, 0\}, \{15 \rightarrow 152, 1\}, \{58 \rightarrow 60, 0\},$   
 $\{58 \rightarrow 93, 1\}, \{60 \rightarrow 60, 0\}, \{60 \rightarrow 106, 1\}, \{63 \rightarrow 58, 0\}, \{63 \rightarrow 112, 1\},$   
 $\{153 \rightarrow 58, 0\}, \{153 \rightarrow 124, 1\}, \{154 \rightarrow 155, 0\}, \{154 \rightarrow 121, 1\}, \{156 \rightarrow 157, 0\},$   
 $\{156 \rightarrow 121, 1\}, \{158 \rightarrow 159, 0\}, \{158 \rightarrow 46, 1\}, \{160 \rightarrow 161, 0\}, \{160 \rightarrow 46, 1\},$   
 $\{162 \rightarrow 163, 0\}, \{162 \rightarrow 122, 1\}, \{164 \rightarrow 165, 0\}, \{164 \rightarrow 122, 1\}, \{166 \rightarrow 167, 0\},$   
 $\{166 \rightarrow 124, 1\}, \{168 \rightarrow 169, 0\}, \{168 \rightarrow 124, 1\}, \{170 \rightarrow 171, 0\}, \{170 \rightarrow 26, 1\},$   
 $\{129 \rightarrow 153, 0\}, \{129 \rightarrow 28, 1\}, \{172 \rightarrow 173, 0\}, \{172 \rightarrow 28, 1\}, \{131 \rightarrow 153, 0\},$   
 $\{131 \rightarrow 42, 1\}, \{142 \rightarrow 63, 0\}, \{142 \rightarrow 6, 1\}, \{140 \rightarrow 63, 0\}, \{140 \rightarrow 16, 1\},$   
 $\{174 \rightarrow 175, 0\}, \{174 \rightarrow 26, 1\}, \{171 \rightarrow 176, 0\}, \{171 \rightarrow 29, 1\}, \{177 \rightarrow 178, 0\},$   
 $\{177 \rightarrow 32, 1\}, \{179 \rightarrow 86, 0\}, \{179 \rightarrow 32, 1\}, \{180 \rightarrow 181, 0\}, \{180 \rightarrow 29, 1\},$   
 $\{182 \rightarrow 183, 0\}, \{182 \rightarrow 29, 1\}, \{173 \rightarrow 65, 0\}, \{173 \rightarrow 46, 1\}, \{175 \rightarrow 184, 0\},$   
 $\{175 \rightarrow 26, 1\}, \{185 \rightarrow 154, 0\}, \{185 \rightarrow 186, 1\}, \{187 \rightarrow 129, 0\}, \{187 \rightarrow 188, 1\},$   
 $\{189 \rightarrow 179, 0\}, \{189 \rightarrow 188, 1\}, \{190 \rightarrow 162, 0\}, \{190 \rightarrow 186, 1\}, \{186 \rightarrow 191, 0\},$   
 $\{186 \rightarrow 192, 1\}, \{192 \rightarrow 187, 0\}, \{192 \rightarrow 193, 1\}, \{193 \rightarrow 193, 0\}, \{193 \rightarrow 193, 1\},$   
 $\{188 \rightarrow 194, 0\}, \{188 \rightarrow 192, 1\}, \{151 \rightarrow 148, 0\}, \{151 \rightarrow 194, 1\}, \{148 \rightarrow 193, 0\},$   
 $\{148 \rightarrow 187, 1\}, \{195 \rightarrow 148, 0\}, \{195 \rightarrow 191, 1\}, \{196 \rightarrow 197, 0\}, \{196 \rightarrow 162, 1\},$   
 $\{191 \rightarrow 198, 0\}, \{191 \rightarrow 164, 1\}, \{199 \rightarrow 200, 0\}, \{199 \rightarrow 164, 1\}, \{201 \rightarrow 202, 0\},$   
 $\{201 \rightarrow 162, 1\}, \{203 \rightarrow 204, 0\}, \{203 \rightarrow 166, 1\}, \{194 \rightarrow 205, 0\}, \{194 \rightarrow 166, 1\},$   
 $\{206 \rightarrow 207, 0\}, \{206 \rightarrow 168, 1\}, \{208 \rightarrow 209, 0\}, \{208 \rightarrow 168, 1\}, \{65 \rightarrow 151, 0\},$   
 $\{65 \rightarrow 129, 1\}, \{86 \rightarrow 195, 0\}, \{86 \rightarrow 162, 1\}, \{70 \rightarrow 151, 0\}, \{70 \rightarrow 179, 1\},$   
 $\{81 \rightarrow 195, 0\}, \{81 \rightarrow 154, 1\}, \{178 \rightarrow 142, 0\}, \{178 \rightarrow 168, 1\}, \{181 \rightarrow 210, 0\},$   
 $\{181 \rightarrow 192, 1\}, \{183 \rightarrow 211, 0\}, \{183 \rightarrow 186, 1\}, \{155 \rightarrow 95, 0\}, \{155 \rightarrow 203, 1\},$   
 $\{74 \rightarrow 95, 0\}, \{74 \rightarrow 199, 1\}, \{176 \rightarrow 44, 0\}, \{176 \rightarrow 189, 1\}, \{78 \rightarrow 44, 0\},$   
 $\{78 \rightarrow 192, 1\}, \{197 \rightarrow 67, 0\}, \{197 \rightarrow 194, 1\}, \{198 \rightarrow 98, 0\}, \{198 \rightarrow 177, 1\},$   
 $\{136 \rightarrow 55, 0\}, \{136 \rightarrow 164, 1\}, \{138 \rightarrow 98, 0\}, \{138 \rightarrow 172, 1\}, \{210 \rightarrow 55, 0\},$   
 $\{210 \rightarrow 156, 1\}, \{157 \rightarrow 33, 0\}, \{157 \rightarrow 206, 1\}, \{159 \rightarrow 69, 0\}, \{159 \rightarrow 179, 1\},$   
 $\{200 \rightarrow 37, 0\}, \{200 \rightarrow 180, 1\}, \{161 \rightarrow 144, 0\}, \{161 \rightarrow 182, 1\}, \{202 \rightarrow 146, 0\},$   
 $\{202 \rightarrow 208, 1\}, \{163 \rightarrow 47, 0\}, \{163 \rightarrow 19, 1\}, \{76 \rightarrow 51, 0\}, \{76 \rightarrow 26, 1\},$   
 $\{91 \rightarrow 47, 0\}, \{91 \rightarrow 12, 1\}, \{184 \rightarrow 51, 0\}, \{184 \rightarrow 45, 1\}, \{204 \rightarrow 126, 0\},$   
 $\{204 \rightarrow 108, 1\}, \{165 \rightarrow 99, 0\}, \{165 \rightarrow 21, 1\}, \{205 \rightarrow 49, 0\}, \{205 \rightarrow 110, 1\},$   
 $\{147 \rightarrow 52, 0\}, \{147 \rightarrow 122, 1\}, \{150 \rightarrow 49, 0\}, \{150 \rightarrow 104, 1\}, \{211 \rightarrow 52, 0\},$

$\{211 \rightarrow 119, 1\}$ ,  $\{167 \rightarrow 133, 0\}$ ,  $\{167 \rightarrow 106, 1\}$ ,  $\{207 \rightarrow 135, 0\}$ ,  $\{207 \rightarrow 16, 1\}$ ,  
 $\{169 \rightarrow 83, 0\}$ ,  $\{169 \rightarrow 40, 1\}$ ,  $\{209 \rightarrow 88, 0\}$ ,  $\{209 \rightarrow 24, 1\}$ ,  $\{3 \rightarrow 82, 0\}$ ,  
 $\{3 \rightarrow 185, 1\}$ ,  $\{27 \rightarrow 89, 0\}$ ,  $\{27 \rightarrow 190, 1\}$ ,  $\{41 \rightarrow 84, 0\}$ ,  $\{41 \rightarrow 185, 1\}$ ,  
 $\{31 \rightarrow 87, 0\}$ ,  $\{31 \rightarrow 190, 1\}$ ,  $\{149 \rightarrow 212, 0\}$ ,  $\{149 \rightarrow 156, 1\}$ ,  $\{137 \rightarrow 213, 0\}$ ,  
 $\{137 \rightarrow 156, 1\}$ ,  $\{38 \rightarrow 214, 0\}$ ,  $\{38 \rightarrow 154, 1\}$ ,  $\{132 \rightarrow 215, 0\}$ ,  $\{132 \rightarrow 154, 1\}$ ,  
 $\{216 \rightarrow 212, 0\}$ ,  $\{216 \rightarrow 164, 1\}$ ,  $\{217 \rightarrow 218, 0\}$ ,  $\{217 \rightarrow 172, 1\}$ ,  $\{219 \rightarrow 218, 0\}$ ,  
 $\{219 \rightarrow 177, 1\}$ ,  $\{220 \rightarrow 68, 0\}$ ,  $\{220 \rightarrow 187, 1\}$ ,  $\{221 \rightarrow 66, 0\}$ ,  $\{221 \rightarrow 187, 1\}$ ,  
 $\{130 \rightarrow 71, 0\}$ ,  $\{130 \rightarrow 189, 1\}$ ,  $\{34 \rightarrow 72, 0\}$ ,  $\{34 \rightarrow 189, 1\}$ ,  $\{222 \rightarrow 223, 0\}$ ,  
 $\{222 \rightarrow 158, 1\}$ ,  $\{36 \rightarrow 224, 0\}$ ,  $\{36 \rightarrow 160, 1\}$ ,  $\{134 \rightarrow 225, 0\}$ ,  $\{134 \rightarrow 160, 1\}$ ,  
 $\{226 \rightarrow 227, 0\}$ ,  $\{226 \rightarrow 203, 1\}$ ,  $\{228 \rightarrow 227, 0\}$ ,  $\{228 \rightarrow 199, 1\}$ ,  $\{229 \rightarrow 230, 0\}$ ,  
 $\{229 \rightarrow 192, 1\}$ ,  $\{231 \rightarrow 230, 0\}$ ,  $\{231 \rightarrow 189, 1\}$ ,  $\{232 \rightarrow 233, 0\}$ ,  $\{232 \rightarrow 190, 1\}$ ,  
 $\{234 \rightarrow 235, 0\}$ ,  $\{234 \rightarrow 154, 1\}$ ,  $\{236 \rightarrow 237, 0\}$ ,  $\{236 \rightarrow 160, 1\}$ ,  $\{238 \rightarrow 239, 0\}$ ,  
 $\{238 \rightarrow 196, 1\}$ ,  $\{240 \rightarrow 241, 0\}$ ,  $\{240 \rightarrow 170, 1\}$ ,  $\{242 \rightarrow 243, 0\}$ ,  $\{242 \rightarrow 129, 1\}$ ,  
 $\{244 \rightarrow 243, 0\}$ ,  $\{244 \rightarrow 179, 1\}$ ,  $\{245 \rightarrow 246, 0\}$ ,  $\{245 \rightarrow 162, 1\}$ ,  $\{247 \rightarrow 246, 0\}$ ,  
 $\{247 \rightarrow 154, 1\}$ ,  $\{243 \rightarrow 248, 0\}$ ,  $\{243 \rightarrow 194, 1\}$ ,  $\{248 \rightarrow 249, 0\}$ ,  $\{248 \rightarrow 187, 1\}$ ,  
 $\{249 \rightarrow 249, 0\}$ ,  $\{249 \rightarrow 193, 1\}$ ,  $\{246 \rightarrow 248, 0\}$ ,  $\{246 \rightarrow 191, 1\}$ ,  $\{250 \rightarrow 216, 0\}$ ,  
 $\{250 \rightarrow 199, 1\}$ ,  $\{251 \rightarrow 252, 0\}$ ,  $\{251 \rightarrow 201, 1\}$ ,  $\{253 \rightarrow 217, 0\}$ ,  $\{253 \rightarrow 172, 1\}$ ,  
 $\{254 \rightarrow 255, 0\}$ ,  $\{254 \rightarrow 174, 1\}$ ,  $\{256 \rightarrow 257, 0\}$ ,  $\{256 \rightarrow 6, 1\}$ ,  $\{241 \rightarrow 257, 0\}$ ,  
 $\{241 \rightarrow 16, 1\}$ ,  $\{252 \rightarrow 258, 0\}$ ,  $\{252 \rightarrow 42, 1\}$ ,  $\{259 \rightarrow 258, 0\}$ ,  $\{259 \rightarrow 28, 1\}$ ,  
 $\{257 \rightarrow 260, 0\}$ ,  $\{257 \rightarrow 112, 1\}$ ,  $\{260 \rightarrow 261, 0\}$ ,  $\{260 \rightarrow 93, 1\}$ ,  $\{261 \rightarrow 261, 0\}$ ,  
 $\{261 \rightarrow 106, 1\}$ ,  $\{258 \rightarrow 260, 0\}$ ,  $\{258 \rightarrow 124, 1\}$ ,  $\{262 \rightarrow 263, 0\}$ ,  $\{262 \rightarrow 12, 1\}$ ,  
 $\{264 \rightarrow 244, 0\}$ ,  $\{264 \rightarrow 44, 1\}$ ,  $\{265 \rightarrow 228, 0\}$ ,  $\{265 \rightarrow 102, 1\}$ ,  $\{266 \rightarrow 229, 0\}$ ,  
 $\{266 \rightarrow 14, 1\}$ ,  $\{267 \rightarrow 247, 0\}$ ,  $\{267 \rightarrow 9, 1\}$ ,  $\{268 \rightarrow 269, 0\}$ ,  $\{268 \rightarrow 104, 1\}$ ,  
 $\{143 \rightarrow 270, 0\}$ ,  $\{143 \rightarrow 112, 1\}$ ,  $\{239 \rightarrow 271, 0\}$ ,  $\{239 \rightarrow 122, 1\}$ ,  $\{48 \rightarrow 272, 0\}$ ,  
 $\{48 \rightarrow 112, 1\}$ ,  $\{273 \rightarrow 271, 0\}$ ,  $\{273 \rightarrow 119, 1\}$ ,  $\{274 \rightarrow 275, 0\}$ ,  $\{274 \rightarrow 119, 1\}$ ,  
 $\{276 \rightarrow 277, 0\}$ ,  $\{276 \rightarrow 110, 1\}$ ,  $\{255 \rightarrow 277, 0\}$ ,  $\{255 \rightarrow 104, 1\}$ ,  $\{8 \rightarrow 278, 0\}$ ,  
 $\{8 \rightarrow 43, 1\}$ ,  $\{18 \rightarrow 279, 0\}$ ,  $\{18 \rightarrow 117, 1\}$ ,  $\{23 \rightarrow 280, 0\}$ ,  $\{23 \rightarrow 117, 1\}$ ,  
 $\{11 \rightarrow 281, 0\}$ ,  $\{11 \rightarrow 43, 1\}$ ,  $\{53 \rightarrow 282, 0\}$ ,  $\{53 \rightarrow 39, 1\}$ ,  $\{145 \rightarrow 283, 0\}$ ,  
 $\{145 \rightarrow 39, 1\}$ ,  $\{284 \rightarrow 285, 0\}$ ,  $\{284 \rightarrow 30, 1\}$ ,  $\{286 \rightarrow 287, 0\}$ ,  $\{286 \rightarrow 30, 1\}$ ,  
 $\{139 \rightarrow 288, 0\}$ ,  $\{139 \rightarrow 42, 1\}$ ,  $\{152 \rightarrow 289, 0\}$ ,  $\{152 \rightarrow 42, 1\}$ ,  $\{50 \rightarrow 290, 0\}$ ,  
 $\{50 \rightarrow 45, 1\}$ ,  $\{141 \rightarrow 291, 0\}$ ,  $\{141 \rightarrow 45, 1\}$ ,  $\{263 \rightarrow 292, 0\}$ ,  $\{263 \rightarrow 26, 1\}$ ,  
 $\{293 \rightarrow 292, 0\}$ ,  $\{293 \rightarrow 45, 1\}$ ,  $\{269 \rightarrow 294, 0\}$ ,  $\{269 \rightarrow 12, 1\}$ ,  $\{295 \rightarrow 294, 0\}$ ,  
 $\{295 \rightarrow 19, 1\}$ ,  $\{296 \rightarrow 297, 0\}$ ,  $\{296 \rightarrow 39, 1\}$ ,  $\{298 \rightarrow 299, 0\}$ ,  $\{298 \rightarrow 112, 1\}$ ,  
 $\{300 \rightarrow 301, 0\}$ ,  $\{300 \rightarrow 43, 1\}$ ,  $\{59 \rightarrow 238, 0\}$ ,  $\{59 \rightarrow 128, 1\}$ ,  $\{128 \rightarrow 240, 0\}$ ,  
 $\{128 \rightarrow 66, 1\}$ ,  $\{66 \rightarrow 242, 0\}$ ,  $\{66 \rightarrow 66, 1\}$ ,  $\{302 \rightarrow 242, 0\}$ ,  $\{302 \rightarrow 68, 1\}$ ,  
 $\{303 \rightarrow 250, 0\}$ ,  $\{303 \rightarrow 128, 1\}$ ,  $\{304 \rightarrow 244, 0\}$ ,  $\{304 \rightarrow 71, 1\}$ ,  $\{235 \rightarrow 244, 0\}$ ,  
 $\{235 \rightarrow 72, 1\}$ ,  $\{114 \rightarrow 262, 0\}$ ,  $\{114 \rightarrow 303, 1\}$ ,  $\{68 \rightarrow 260, 0\}$ ,  $\{68 \rightarrow 59, 1\}$ ,  
 $\{123 \rightarrow 264, 0\}$ ,  $\{123 \rightarrow 59, 1\}$ ,  $\{116 \rightarrow 266, 0\}$ ,  $\{116 \rightarrow 303, 1\}$ ,  $\{71 \rightarrow 293, 0\}$ ,  
 $\{71 \rightarrow 305, 1\}$ ,  $\{127 \rightarrow 296, 0\}$ ,  $\{127 \rightarrow 305, 1\}$ ,  $\{306 \rightarrow 298, 0\}$ ,  $\{306 \rightarrow 307, 1\}$ ,  
 $\{308 \rightarrow 300, 0\}$ ,  $\{308 \rightarrow 307, 1\}$ ,  $\{282 \rightarrow 226, 0\}$ ,  $\{282 \rightarrow 128, 1\}$ ,  $\{75 \rightarrow 232, 0\}$ ,  
 $\{75 \rightarrow 97, 1\}$ ,  $\{72 \rightarrow 231, 0\}$ ,  $\{72 \rightarrow 97, 1\}$ ,  $\{92 \rightarrow 234, 0\}$ ,  $\{92 \rightarrow 87, 1\}$ ,  
 $\{61 \rightarrow 236, 0\}$ ,  $\{61 \rightarrow 87, 1\}$ ,  $\{309 \rightarrow 245, 0\}$ ,  $\{309 \rightarrow 89, 1\}$ ,  $\{310 \rightarrow 247, 0\}$ ,  
 $\{310 \rightarrow 84, 1\}$ ,  $\{285 \rightarrow 245, 0\}$ ,  $\{285 \rightarrow 87, 1\}$ ,  $\{301 \rightarrow 247, 0\}$ ,  $\{301 \rightarrow 82, 1\}$ ,  
 $\{283 \rightarrow 295, 0\}$ ,  $\{283 \rightarrow 303, 1\}$ ,  $\{287 \rightarrow 258, 0\}$ ,  $\{287 \rightarrow 307, 1\}$ ,  $\{82 \rightarrow 256, 0\}$ ,  
 $\{82 \rightarrow 143, 1\}$ ,  $\{64 \rightarrow 265, 0\}$ ,  $\{64 \rightarrow 48, 1\}$ ,  $\{79 \rightarrow 267, 0\}$ ,  $\{79 \rightarrow 143, 1\}$ ,  
 $\{77 \rightarrow 268, 0\}$ ,  $\{77 \rightarrow 48, 1\}$ ,  $\{311 \rightarrow 241, 0\}$ ,  $\{311 \rightarrow 145, 1\}$ ,  $\{312 \rightarrow 256, 0\}$ ,  
 $\{312 \rightarrow 11, 1\}$ ,  $\{237 \rightarrow 241, 0\}$ ,  $\{237 \rightarrow 141, 1\}$ ,  $\{89 \rightarrow 149, 0\}$ ,  $\{89 \rightarrow 220, 1\}$ ,

$\{107 \rightarrow 3, 0\}, \{107 \rightarrow 221, 1\}, \{109 \rightarrow 221, 0\}, \{109 \rightarrow 221, 1\}, \{101 \rightarrow 222, 0\},$   
 $\{101 \rightarrow 220, 1\}, \{97 \rightarrow 23, 0\}, \{97 \rightarrow 34, 1\}, \{305 \rightarrow 152, 0\}, \{305 \rightarrow 130, 1\},$   
 $\{87 \rightarrow 273, 0\}, \{87 \rightarrow 34, 1\}, \{307 \rightarrow 284, 0\}, \{307 \rightarrow 130, 1\}, \{100 \rightarrow 251, 0\},$   
 $\{100 \rightarrow 273, 1\}, \{84 \rightarrow 246, 0\}, \{84 \rightarrow 273, 1\}, \{313 \rightarrow 253, 0\}, \{313 \rightarrow 274, 1\},$   
 $\{314 \rightarrow 254, 0\}, \{314 \rightarrow 274, 1\}, \{288 \rightarrow 249, 0\}, \{288 \rightarrow 221, 1\}, \{289 \rightarrow 259, 0\},$   
 $\{289 \rightarrow 130, 1\}, \{315 \rightarrow 259, 0\}, \{315 \rightarrow 27, 1\}, \{316 \rightarrow 252, 0\}, \{316 \rightarrow 134, 1\},$   
 $\{299 \rightarrow 252, 0\}, \{299 \rightarrow 132, 1\}, \{290 \rightarrow 276, 0\}, \{290 \rightarrow 48, 1\}, \{291 \rightarrow 219, 0\},$   
 $\{291 \rightarrow 274, 1\}, \{270 \rightarrow 302, 0\}, \{270 \rightarrow 222, 1\}, \{271 \rightarrow 317, 0\}, \{271 \rightarrow 53, 1\},$   
 $\{294 \rightarrow 223, 0\}, \{294 \rightarrow 48, 1\}, \{292 \rightarrow 223, 0\}, \{292 \rightarrow 8, 1\}, \{277 \rightarrow 317, 0\},$   
 $\{277 \rightarrow 50, 1\}, \{317 \rightarrow 318, 0\}, \{317 \rightarrow 38, 1\}, \{223 \rightarrow 318, 0\}, \{223 \rightarrow 36, 1\},$   
 $\{318 \rightarrow 233, 0\}, \{318 \rightarrow 34, 1\}, \{233 \rightarrow 233, 0\}, \{233 \rightarrow 31, 1\}, \{224 \rightarrow 311, 0\},$   
 $\{224 \rightarrow 145, 1\}, \{272 \rightarrow 312, 0\}, \{272 \rightarrow 134, 1\}, \{275 \rightarrow 218, 0\}, \{275 \rightarrow 286, 1\},$   
 $\{225 \rightarrow 304, 0\}, \{225 \rightarrow 284, 1\}, \{212 \rightarrow 319, 0\}, \{212 \rightarrow 100, 1\}, \{227 \rightarrow 297, 0\},$   
 $\{227 \rightarrow 97, 1\}, \{230 \rightarrow 297, 0\}, \{230 \rightarrow 101, 1\}, \{218 \rightarrow 319, 0\}, \{218 \rightarrow 79, 1\},$   
 $\{278 \rightarrow 309, 0\}, \{278 \rightarrow 84, 1\}, \{319 \rightarrow 280, 0\}, \{319 \rightarrow 128, 1\}, \{280 \rightarrow 320, 0\},$   
 $\{280 \rightarrow 127, 1\}, \{320 \rightarrow 320, 0\}, \{320 \rightarrow 75, 1\}, \{297 \rightarrow 280, 0\}, \{297 \rightarrow 123, 1\},$   
 $\{213 \rightarrow 294, 0\}, \{213 \rightarrow 313, 1\}, \{214 \rightarrow 310, 0\}, \{214 \rightarrow 71, 1\}, \{279 \rightarrow 277, 0\},$   
 $\{279 \rightarrow 306, 1\}, \{281 \rightarrow 315, 0\}, \{281 \rightarrow 314, 1\}, \{215 \rightarrow 316, 0\}, \{215 \rightarrow 308, 1\}\},$   
1,  $\{1 \rightarrow 0, 2 \rightarrow 0, 3 \rightarrow 1, 4 \rightarrow 0, 5 \rightarrow 0, 6 \rightarrow 0, 7 \rightarrow 0, 8 \rightarrow 1, 9 \rightarrow 0, 10 \rightarrow 0, 11 \rightarrow 1,$   
 $12 \rightarrow 0, 13 \rightarrow 0, 14 \rightarrow 0, 15 \rightarrow 0, 16 \rightarrow 0, 17 \rightarrow 0, 18 \rightarrow 1, 19 \rightarrow 0, 20 \rightarrow 0, 21 \rightarrow 0,$   
 $22 \rightarrow 0, 23 \rightarrow 1, 24 \rightarrow 0, 25 \rightarrow 0, 26 \rightarrow 0, 27 \rightarrow 1, 28 \rightarrow 0, 29 \rightarrow 0, 30 \rightarrow 0, 31 \rightarrow 1,$   
 $32 \rightarrow 0, 33 \rightarrow 0, 34 \rightarrow 1, 35 \rightarrow 0, 36 \rightarrow 1, 37 \rightarrow 0, 38 \rightarrow 1, 39 \rightarrow 0, 40 \rightarrow 0, 41 \rightarrow 1,$   
 $42 \rightarrow 0, 43 \rightarrow 0, 44 \rightarrow 0, 45 \rightarrow 0, 46 \rightarrow 0, 47 \rightarrow 0, 48 \rightarrow 1, 49 \rightarrow 0, 50 \rightarrow 1, 51 \rightarrow 0,$   
 $52 \rightarrow 0, 53 \rightarrow 1, 54 \rightarrow 0, 55 \rightarrow 0, 56 \rightarrow 0, 57 \rightarrow 0, 58 \rightarrow 0, 59 \rightarrow 1, 60 \rightarrow 0, 61 \rightarrow 1,$   
 $62 \rightarrow 0, 63 \rightarrow 0, 64 \rightarrow 1, 65 \rightarrow 0, 66 \rightarrow 1, 67 \rightarrow 0, 68 \rightarrow 1, 69 \rightarrow 0, 70 \rightarrow 0, 71 \rightarrow 1,$   
 $72 \rightarrow 1, 73 \rightarrow 0, 74 \rightarrow 0, 75 \rightarrow 1, 76 \rightarrow 0, 77 \rightarrow 1, 78 \rightarrow 0, 79 \rightarrow 1, 80 \rightarrow 0, 81 \rightarrow 0,$   
 $82 \rightarrow 1, 83 \rightarrow 0, 84 \rightarrow 1, 85 \rightarrow 0, 86 \rightarrow 0, 87 \rightarrow 1, 88 \rightarrow 0, 89 \rightarrow 1, 90 \rightarrow 0, 91 \rightarrow 0,$   
 $92 \rightarrow 1, 93 \rightarrow 0, 94 \rightarrow 0, 95 \rightarrow 0, 96 \rightarrow 0, 97 \rightarrow 1, 98 \rightarrow 0, 99 \rightarrow 0, 100 \rightarrow 1, 101 \rightarrow 1,$   
 $102 \rightarrow 0, 103 \rightarrow 0, 104 \rightarrow 0, 105 \rightarrow 0, 106 \rightarrow 0, 107 \rightarrow 1, 108 \rightarrow 0, 109 \rightarrow 1, 110 \rightarrow 0,$   
 $111 \rightarrow 0, 112 \rightarrow 0, 113 \rightarrow 0, 114 \rightarrow 1, 115 \rightarrow 0, 116 \rightarrow 1, 117 \rightarrow 0, 118 \rightarrow 0, 119 \rightarrow 0,$   
 $120 \rightarrow 0, 121 \rightarrow 0, 122 \rightarrow 0, 123 \rightarrow 1, 124 \rightarrow 0, 125 \rightarrow 0, 126 \rightarrow 0, 127 \rightarrow 1, 128 \rightarrow 1,$   
 $129 \rightarrow 0, 130 \rightarrow 1, 131 \rightarrow 0, 132 \rightarrow 1, 133 \rightarrow 0, 134 \rightarrow 1, 135 \rightarrow 0, 136 \rightarrow 0, 137 \rightarrow 1,$   
 $138 \rightarrow 0, 139 \rightarrow 1, 140 \rightarrow 0, 141 \rightarrow 1, 142 \rightarrow 0, 143 \rightarrow 1, 144 \rightarrow 0, 145 \rightarrow 1, 146 \rightarrow 0,$   
 $147 \rightarrow 0, 148 \rightarrow 0, 149 \rightarrow 1, 150 \rightarrow 0, 151 \rightarrow 0, 152 \rightarrow 1, 153 \rightarrow 0, 154 \rightarrow 0, 155 \rightarrow 0,$   
 $156 \rightarrow 0, 157 \rightarrow 0, 158 \rightarrow 0, 159 \rightarrow 0, 160 \rightarrow 0, 161 \rightarrow 0, 162 \rightarrow 0, 163 \rightarrow 0, 164 \rightarrow 0,$   
 $165 \rightarrow 0, 166 \rightarrow 0, 167 \rightarrow 0, 168 \rightarrow 0, 169 \rightarrow 0, 170 \rightarrow 0, 171 \rightarrow 0, 172 \rightarrow 0, 173 \rightarrow 0,$   
 $174 \rightarrow 0, 175 \rightarrow 0, 176 \rightarrow 0, 177 \rightarrow 0, 178 \rightarrow 0, 179 \rightarrow 0, 180 \rightarrow 0, 181 \rightarrow 0, 182 \rightarrow 0,$   
 $183 \rightarrow 0, 184 \rightarrow 0, 185 \rightarrow 0, 186 \rightarrow 0, 187 \rightarrow 0, 188 \rightarrow 0, 189 \rightarrow 0, 190 \rightarrow 0, 191 \rightarrow 0,$   
 $192 \rightarrow 0, 193 \rightarrow 0, 194 \rightarrow 0, 195 \rightarrow 0, 196 \rightarrow 0, 197 \rightarrow 0, 198 \rightarrow 0, 199 \rightarrow 0, 200 \rightarrow 0,$   
 $201 \rightarrow 0, 202 \rightarrow 0, 203 \rightarrow 0, 204 \rightarrow 0, 205 \rightarrow 0, 206 \rightarrow 0, 207 \rightarrow 0, 208 \rightarrow 0, 209 \rightarrow 0,$   
 $210 \rightarrow 0, 211 \rightarrow 0, 212 \rightarrow 1, 213 \rightarrow 1, 214 \rightarrow 1, 215 \rightarrow 1, 216 \rightarrow 1, 217 \rightarrow 1, 218 \rightarrow 1,$   
 $219 \rightarrow 1, 220 \rightarrow 1, 221 \rightarrow 1, 222 \rightarrow 1, 223 \rightarrow 1, 224 \rightarrow 1, 225 \rightarrow 1, 226 \rightarrow 1, 227 \rightarrow 1,$   
 $228 \rightarrow 1, 229 \rightarrow 1, 230 \rightarrow 1, 231 \rightarrow 1, 232 \rightarrow 1, 233 \rightarrow 1, 234 \rightarrow 1, 235 \rightarrow 1, 236 \rightarrow 1,$   
 $237 \rightarrow 1, 238 \rightarrow 1, 239 \rightarrow 1, 240 \rightarrow 1, 241 \rightarrow 1, 242 \rightarrow 1, 243 \rightarrow 1, 244 \rightarrow 1, 245 \rightarrow 1,$   
 $246 \rightarrow 1, 247 \rightarrow 1, 248 \rightarrow 1, 249 \rightarrow 1, 250 \rightarrow 1, 251 \rightarrow 1, 252 \rightarrow 1, 253 \rightarrow 1, 254 \rightarrow 1,$   
 $255 \rightarrow 1, 256 \rightarrow 1, 257 \rightarrow 1, 258 \rightarrow 1, 259 \rightarrow 1, 260 \rightarrow 1, 261 \rightarrow 1, 262 \rightarrow 1, 263 \rightarrow 1,$   
 $264 \rightarrow 1, 265 \rightarrow 1, 266 \rightarrow 1, 267 \rightarrow 1, 268 \rightarrow 1, 269 \rightarrow 1, 270 \rightarrow 1, 271 \rightarrow 1, 272 \rightarrow 1,$

```

273 → 1, 274 → 1, 275 → 1, 276 → 1, 277 → 1, 278 → 1, 279 → 1, 280 → 1, 281 → 1,
282 → 1, 283 → 1, 284 → 1, 285 → 1, 286 → 1, 287 → 1, 288 → 1, 289 → 1, 290 → 1,
291 → 1, 292 → 1, 293 → 1, 294 → 1, 295 → 1, 296 → 1, 297 → 1, 298 → 1,
299 → 1, 300 → 1, 301 → 1, 302 → 1, 303 → 1, 304 → 1, 305 → 1, 306 → 1,
307 → 1, 308 → 1, 309 → 1, 310 → 1, 311 → 1, 312 → 1, 313 → 1, 314 → 1,
315 → 1, 316 → 1, 317 → 1, 318 → 1, 319 → 1, 320 → 1}, InputAlphabet → {0, 1}]

```

```

In[ ]:= edge[x_, ___] := {Arrowheads[0.020], Arrow[x, 0.1]}
AutomatonGraph[automatonsigma8, VertexSize → 0.3, EdgeShapeFunction → edge]

```

Out[ ]:=

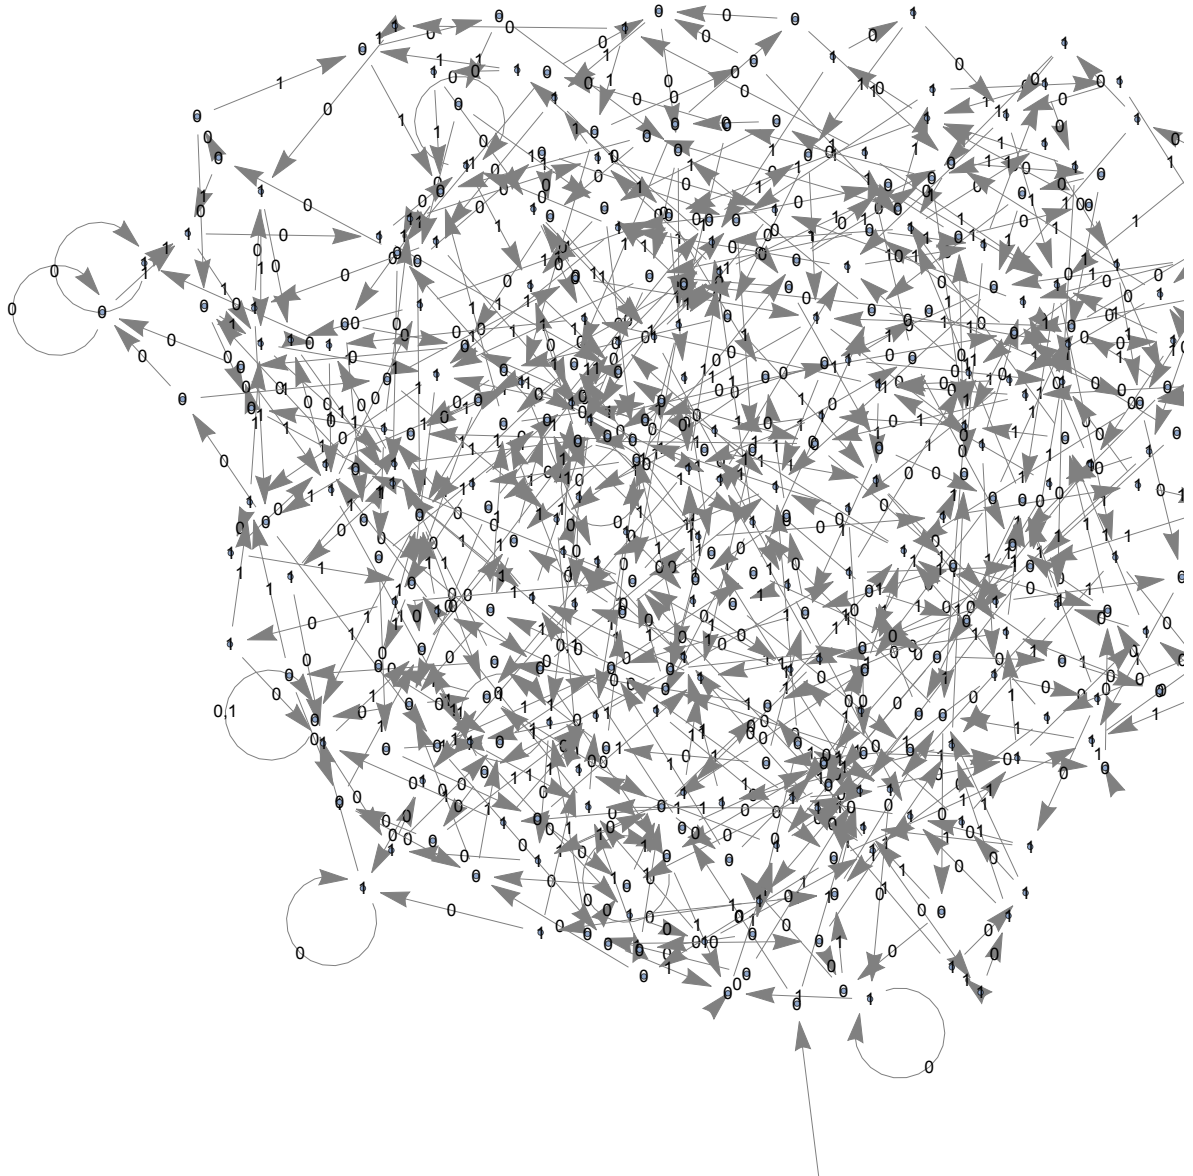

$\sigma_8^{03}$ 

```

In[ ]:= fsigma83[t_, s_] := s^5 + s^3 t + s^4 t + s^2 t^2 + s^4 t^2 + s^6 t^2 + s t^3 + s^3 t^3 + t^4 + s^4 t^4 + t^6 + s^4 t^6
initsigma83[t_] := t + t^2 + t^4 + t^5 + t^8 + t^10 + 0[t]^13
automatonsigma83 = AutomaticSequenceAutomaton[
  AutomaticSequenceReduce[AlgebraicSequence[SeriesRoot[
    {Function[s, fsigma83[t, s]], initsigma83[t]], Modulus -> 2]][n], n]]
Out[ ]:= Automaton[{ {1 -> 2, 0}, {1 -> 3, 1}, {4 -> 5, 0}, {4 -> 6, 1}, {7 -> 8, 0}, {7 -> 9, 1},
  {10 -> 7, 0}, {10 -> 11, 1}, {8 -> 8, 0}, {8 -> 12, 1}, {13 -> 7, 0}, {13 -> 14, 1},
  {15 -> 16, 0}, {15 -> 6, 1}, {17 -> 18, 0}, {17 -> 12, 1}, {2 -> 19, 0}, {2 -> 20, 1},
  {21 -> 10, 0}, {21 -> 22, 1}, {23 -> 13, 0}, {23 -> 24, 1}, {25 -> 13, 0}, {25 -> 26, 1},
  {27 -> 10, 0}, {27 -> 28, 1}, {19 -> 29, 0}, {19 -> 30, 1}, {5 -> 31, 0}, {5 -> 32, 1},
  {33 -> 34, 0}, {33 -> 35, 1}, {36 -> 37, 0}, {36 -> 35, 1}, {38 -> 39, 0}, {38 -> 32, 1},
  {40 -> 41, 0}, {40 -> 6, 1}, {42 -> 43, 0}, {42 -> 26, 1}, {44 -> 45, 0}, {44 -> 26, 1},
  {46 -> 47, 0}, {46 -> 48, 1}, {16 -> 49, 0}, {16 -> 48, 1}, {50 -> 29, 0}, {50 -> 51, 1},
  {52 -> 53, 0}, {52 -> 51, 1}, {54 -> 55, 0}, {54 -> 51, 1}, {56 -> 57, 0}, {56 -> 58, 1},
  {18 -> 59, 0}, {18 -> 58, 1}, {60 -> 61, 0}, {60 -> 35, 1}, {29 -> 62, 0}, {29 -> 63, 1},
  {31 -> 64, 0}, {31 -> 65, 1}, {66 -> 62, 0}, {66 -> 67, 1}, {68 -> 64, 0}, {68 -> 69, 1},
  {70 -> 71, 0}, {70 -> 72, 1}, {73 -> 74, 0}, {73 -> 75, 1}, {76 -> 77, 0}, {76 -> 78, 1},
  {79 -> 80, 0}, {79 -> 81, 1}, {34 -> 82, 0}, {34 -> 83, 1}, {84 -> 85, 0}, {84 -> 86, 1},
  {87 -> 85, 0}, {87 -> 88, 1}, {89 -> 90, 0}, {89 -> 91, 1}, {92 -> 90, 0}, {92 -> 93, 1},
  {37 -> 94, 0}, {37 -> 95, 1}, {39 -> 96, 0}, {39 -> 97, 1}, {98 -> 73, 0}, {98 -> 99, 1},
  {100 -> 76, 0}, {100 -> 67, 1}, {101 -> 79, 0}, {101 -> 99, 1}, {53 -> 87, 0},
  {53 -> 67, 1}, {102 -> 103, 0}, {102 -> 91, 1}, {59 -> 104, 0}, {59 -> 105, 1},
  {106 -> 104, 0}, {106 -> 107, 1}, {108 -> 109, 0}, {108 -> 105, 1}, {110 -> 111, 0},
  {110 -> 95, 1}, {112 -> 113, 0}, {112 -> 91, 1}, {61 -> 111, 0}, {61 -> 114, 1},
  {115 -> 40, 0}, {115 -> 116, 1}, {117 -> 50, 0}, {117 -> 116, 1}, {57 -> 25, 0},
  {57 -> 118, 1}, {119 -> 60, 0}, {119 -> 118, 1}, {103 -> 120, 0}, {103 -> 116, 1},
  {121 -> 122, 0}, {121 -> 123, 1}, {124 -> 125, 0}, {124 -> 126, 1}, {127 -> 128, 0},
  {127 -> 126, 1}, {55 -> 129, 0}, {55 -> 123, 1}, {104 -> 130, 0}, {104 -> 99, 1},
  {130 -> 131, 0}, {130 -> 132, 1}, {131 -> 131, 0}, {131 -> 81, 1}, {111 -> 130, 0},
  {111 -> 133, 1}, {109 -> 27, 0}, {109 -> 126, 1}, {113 -> 92, 0}, {113 -> 91, 1},
  {41 -> 134, 0}, {41 -> 135, 1}, {136 -> 134, 0}, {136 -> 48, 1}, {137 -> 138, 0},
  {137 -> 139, 1}, {49 -> 138, 0}, {49 -> 140, 1}, {141 -> 142, 0}, {141 -> 143, 1},
  {120 -> 144, 0}, {120 -> 145, 1}, {146 -> 144, 0}, {146 -> 6, 1}, {129 -> 142, 0},
  {129 -> 147, 1}, {122 -> 148, 0}, {122 -> 149, 1}, {125 -> 150, 0}, {125 -> 22, 1},
  {43 -> 151, 0}, {43 -> 152, 1}, {128 -> 153, 0}, {128 -> 154, 1}, {45 -> 155, 0},
  {45 -> 11, 1}, {47 -> 156, 0}, {47 -> 157, 1}, {158 -> 144, 0}, {158 -> 159, 1},
  {160 -> 161, 0}, {160 -> 162, 1}, {163 -> 164, 0}, {163 -> 162, 1}, {165 -> 166, 0},
  {165 -> 159, 1}, {159 -> 167, 0}, {159 -> 168, 1}, {168 -> 158, 0}, {168 -> 169, 1},
  {156 -> 148, 0}, {156 -> 167, 1}, {169 -> 169, 0}, {169 -> 169, 1}, {148 -> 169, 0},
  {148 -> 158, 1}, {162 -> 170, 0}, {162 -> 168, 1}, {171 -> 148, 0}, {171 -> 170, 1},
  {62 -> 156, 0}, {62 -> 144, 1}, {64 -> 156, 0}, {64 -> 166, 1}, {90 -> 171, 0},
  {90 -> 164, 1}, {85 -> 171, 0}, {85 -> 161, 1}, {167 -> 172, 0}, {167 -> 173, 1},
  {174 -> 175, 0}, {174 -> 176, 1}, {177 -> 178, 0}, {177 -> 173, 1}, {179 -> 180, 0},
  {179 -> 176, 1}, {181 -> 182, 0}, {181 -> 164, 1}, {170 -> 183, 0}, {170 -> 184, 1},

```



$\{185 \rightarrow 186, 0\}, \{185 \rightarrow 164, 1\}, \{187 \rightarrow 188, 0\}, \{187 \rightarrow 184, 1\}, \{189 \rightarrow 134, 0\},$   
 $\{189 \rightarrow 176, 1\}, \{190 \rightarrow 191, 0\}, \{190 \rightarrow 162, 1\}, \{192 \rightarrow 193, 0\}, \{192 \rightarrow 168, 1\},$   
 $\{144 \rightarrow 194, 0\}, \{144 \rightarrow 4, 1\}, \{134 \rightarrow 77, 0\}, \{134 \rightarrow 42, 1\}, \{142 \rightarrow 194, 0\},$   
 $\{142 \rightarrow 54, 1\}, \{195 \rightarrow 196, 0\}, \{195 \rightarrow 15, 1\}, \{197 \rightarrow 198, 0\}, \{197 \rightarrow 4, 1\},$   
 $\{138 \rightarrow 77, 0\}, \{138 \rightarrow 33, 1\}, \{199 \rightarrow 200, 0\}, \{199 \rightarrow 15, 1\}, \{194 \rightarrow 201, 0\},$   
 $\{194 \rightarrow 98, 1\}, \{201 \rightarrow 96, 0\}, \{201 \rightarrow 102, 1\}, \{96 \rightarrow 96, 0\}, \{96 \rightarrow 117, 1\},$   
 $\{77 \rightarrow 201, 0\}, \{77 \rightarrow 127, 1\}, \{202 \rightarrow 203, 0\}, \{202 \rightarrow 100, 1\}, \{161 \rightarrow 204, 0\},$   
 $\{161 \rightarrow 100, 1\}, \{205 \rightarrow 206, 0\}, \{205 \rightarrow 53, 1\}, \{207 \rightarrow 208, 0\}, \{207 \rightarrow 53, 1\},$   
 $\{173 \rightarrow 209, 0\}, \{173 \rightarrow 98, 1\}, \{164 \rightarrow 210, 0\}, \{164 \rightarrow 101, 1\}, \{176 \rightarrow 211, 0\},$   
 $\{176 \rightarrow 98, 1\}, \{184 \rightarrow 212, 0\}, \{184 \rightarrow 101, 1\}, \{166 \rightarrow 90, 0\}, \{166 \rightarrow 8, 1\},$   
 $\{213 \rightarrow 189, 0\}, \{213 \rightarrow 8, 1\}, \{214 \rightarrow 190, 0\}, \{214 \rightarrow 17, 1\}, \{215 \rightarrow 192, 0\},$   
 $\{215 \rightarrow 17, 1\}, \{196 \rightarrow 216, 0\}, \{196 \rightarrow 17, 1\}, \{198 \rightarrow 62, 0\}, \{198 \rightarrow 53, 1\},$   
 $\{200 \rightarrow 217, 0\}, \{200 \rightarrow 15, 1\}, \{71 \rightarrow 29, 0\}, \{71 \rightarrow 218, 1\}, \{218 \rightarrow 41, 0\},$   
 $\{218 \rightarrow 160, 1\}, \{182 \rightarrow 136, 0\}, \{182 \rightarrow 179, 1\}, \{203 \rightarrow 7, 0\}, \{203 \rightarrow 174, 1\},$   
 $\{204 \rightarrow 106, 0\}, \{204 \rightarrow 177, 1\}, \{80 \rightarrow 106, 0\}, \{80 \rightarrow 187, 1\}, \{216 \rightarrow 59, 0\},$   
 $\{216 \rightarrow 165, 1\}, \{94 \rightarrow 59, 0\}, \{94 \rightarrow 168, 1\}, \{183 \rightarrow 110, 0\}, \{183 \rightarrow 213, 1\},$   
 $\{151 \rightarrow 61, 0\}, \{151 \rightarrow 184, 1\}, \{153 \rightarrow 110, 0\}, \{153 \rightarrow 197, 1\}, \{193 \rightarrow 61, 0\},$   
 $\{193 \rightarrow 202, 1\}, \{186 \rightarrow 66, 0\}, \{186 \rightarrow 167, 1\}, \{206 \rightarrow 137, 0\}, \{206 \rightarrow 214, 1\},$   
 $\{208 \rightarrow 68, 0\}, \{208 \rightarrow 166, 1\}, \{188 \rightarrow 10, 0\}, \{188 \rightarrow 215, 1\}, \{172 \rightarrow 21, 0\},$   
 $\{172 \rightarrow 115, 1\}, \{150 \rightarrow 21, 0\}, \{150 \rightarrow 112, 1\}, \{155 \rightarrow 27, 0\}, \{155 \rightarrow 101, 1\},$   
 $\{191 \rightarrow 27, 0\}, \{191 \rightarrow 124, 1\}, \{209 \rightarrow 141, 0\}, \{209 \rightarrow 117, 1\}, \{74 \rightarrow 23, 0\},$   
 $\{74 \rightarrow 44, 1\}, \{210 \rightarrow 23, 0\}, \{210 \rightarrow 36, 1\}, \{82 \rightarrow 25, 0\}, \{82 \rightarrow 15, 1\},$   
 $\{217 \rightarrow 25, 0\}, \{217 \rightarrow 52, 1\}, \{175 \rightarrow 146, 0\}, \{175 \rightarrow 33, 1\}, \{211 \rightarrow 84, 0\},$   
 $\{211 \rightarrow 57, 1\}, \{178 \rightarrow 131, 0\}, \{178 \rightarrow 119, 1\}, \{212 \rightarrow 111, 0\}, \{212 \rightarrow 38, 1\},$   
 $\{180 \rightarrow 89, 0\}, \{180 \rightarrow 5, 1\}, \{3 \rightarrow 63, 0\}, \{3 \rightarrow 158, 1\}, \{219 \rightarrow 67, 0\},$   
 $\{219 \rightarrow 158, 1\}, \{9 \rightarrow 65, 0\}, \{9 \rightarrow 165, 1\}, \{145 \rightarrow 69, 0\}, \{145 \rightarrow 165, 1\},$   
 $\{149 \rightarrow 220, 0\}, \{149 \rightarrow 202, 1\}, \{11 \rightarrow 221, 0\}, \{11 \rightarrow 161, 1\}, \{147 \rightarrow 222, 0\},$   
 $\{147 \rightarrow 161, 1\}, \{152 \rightarrow 223, 0\}, \{152 \rightarrow 202, 1\}, \{224 \rightarrow 220, 0\}, \{224 \rightarrow 184, 1\},$   
 $\{225 \rightarrow 226, 0\}, \{225 \rightarrow 197, 1\}, \{227 \rightarrow 226, 0\}, \{227 \rightarrow 213, 1\}, \{6 \rightarrow 91, 0\},$   
 $\{6 \rightarrow 163, 1\}, \{12 \rightarrow 93, 0\}, \{12 \rightarrow 163, 1\}, \{51 \rightarrow 88, 0\}, \{51 \rightarrow 160, 1\}, \{58 \rightarrow 86, 0\},$   
 $\{58 \rightarrow 160, 1\}, \{228 \rightarrow 229, 0\}, \{228 \rightarrow 161, 1\}, \{230 \rightarrow 231, 0\}, \{230 \rightarrow 165, 1\},$   
 $\{232 \rightarrow 233, 0\}, \{232 \rightarrow 187, 1\}, \{234 \rightarrow 231, 0\}, \{234 \rightarrow 168, 1\}, \{235 \rightarrow 233, 0\},$   
 $\{235 \rightarrow 177, 1\}, \{143 \rightarrow 236, 0\}, \{143 \rightarrow 205, 1\}, \{237 \rightarrow 238, 0\}, \{237 \rightarrow 207, 1\},$   
 $\{14 \rightarrow 239, 0\}, \{14 \rightarrow 205, 1\}, \{240 \rightarrow 241, 0\}, \{240 \rightarrow 163, 1\}, \{242 \rightarrow 243, 0\},$   
 $\{242 \rightarrow 205, 1\}, \{20 \rightarrow 244, 0\}, \{20 \rightarrow 70, 1\}, \{32 \rightarrow 245, 0\}, \{32 \rightarrow 121, 1\},$   
 $\{26 \rightarrow 246, 0\}, \{26 \rightarrow 55, 1\}, \{35 \rightarrow 247, 0\}, \{35 \rightarrow 121, 1\}, \{48 \rightarrow 248, 0\},$   
 $\{48 \rightarrow 55, 1\}, \{249 \rightarrow 250, 0\}, \{249 \rightarrow 124, 1\}, \{135 \rightarrow 251, 0\}, \{135 \rightarrow 127, 1\},$   
 $\{24 \rightarrow 252, 0\}, \{24 \rightarrow 127, 1\}, \{253 \rightarrow 250, 0\}, \{253 \rightarrow 101, 1\}, \{254 \rightarrow 255, 0\},$   
 $\{254 \rightarrow 115, 1\}, \{256 \rightarrow 257, 0\}, \{256 \rightarrow 124, 1\}, \{258 \rightarrow 255, 0\}, \{258 \rightarrow 112, 1\},$   
 $\{22 \rightarrow 259, 0\}, \{22 \rightarrow 52, 1\}, \{157 \rightarrow 260, 0\}, \{157 \rightarrow 54, 1\}, \{154 \rightarrow 261, 0\},$   
 $\{154 \rightarrow 54, 1\}, \{140 \rightarrow 262, 0\}, \{140 \rightarrow 52, 1\}, \{263 \rightarrow 264, 0\}, \{263 \rightarrow 36, 1\},$   
 $\{265 \rightarrow 266, 0\}, \{265 \rightarrow 15, 1\}, \{267 \rightarrow 266, 0\}, \{267 \rightarrow 52, 1\}, \{268 \rightarrow 264, 0\},$   
 $\{268 \rightarrow 44, 1\}, \{269 \rightarrow 270, 0\}, \{269 \rightarrow 56, 1\}, \{28 \rightarrow 271, 0\}, \{28 \rightarrow 56, 1\},$   
 $\{272 \rightarrow 273, 0\}, \{272 \rightarrow 18, 1\}, \{139 \rightarrow 274, 0\}, \{139 \rightarrow 56, 1\}, \{275 \rightarrow 276, 0\},$   
 $\{275 \rightarrow 18, 1\}, \{277 \rightarrow 278, 0\}, \{277 \rightarrow 55, 1\}, \{279 \rightarrow 280, 0\}, \{279 \rightarrow 127, 1\},$   
 $\{30 \rightarrow 281, 0\}, \{30 \rightarrow 159, 1\}, \{282 \rightarrow 283, 0\}, \{282 \rightarrow 162, 1\}, \{284 \rightarrow 285, 0\},$   
 $\{284 \rightarrow 181, 1\}, \{286 \rightarrow 287, 0\}, \{286 \rightarrow 144, 1\}, \{288 \rightarrow 289, 0\}, \{288 \rightarrow 161, 1\},$

$\{290 \rightarrow 287, 0\}$ ,  $\{290 \rightarrow 166, 1\}$ ,  $\{291 \rightarrow 289, 0\}$ ,  $\{291 \rightarrow 164, 1\}$ ,  $\{292 \rightarrow 30, 0\}$ ,  
 $\{292 \rightarrow 169, 1\}$ ,  $\{287 \rightarrow 293, 0\}$ ,  $\{287 \rightarrow 167, 1\}$ ,  $\{293 \rightarrow 294, 0\}$ ,  $\{293 \rightarrow 158, 1\}$ ,  
 $\{294 \rightarrow 294, 0\}$ ,  $\{294 \rightarrow 169, 1\}$ ,  $\{289 \rightarrow 293, 0\}$ ,  $\{289 \rightarrow 170, 1\}$ ,  $\{295 \rightarrow 296, 0\}$ ,  
 $\{295 \rightarrow 195, 1\}$ ,  $\{297 \rightarrow 253, 0\}$ ,  $\{297 \rightarrow 185, 1\}$ ,  $\{298 \rightarrow 224, 0\}$ ,  $\{298 \rightarrow 187, 1\}$ ,  
 $\{299 \rightarrow 225, 0\}$ ,  $\{299 \rightarrow 197, 1\}$ ,  $\{300 \rightarrow 258, 0\}$ ,  $\{300 \rightarrow 199, 1\}$ ,  $\{281 \rightarrow 301, 0\}$ ,  
 $\{281 \rightarrow 4, 1\}$ ,  $\{285 \rightarrow 301, 0\}$ ,  $\{285 \rightarrow 54, 1\}$ ,  $\{296 \rightarrow 302, 0\}$ ,  $\{296 \rightarrow 33, 1\}$ ,  
 $\{303 \rightarrow 302, 0\}$ ,  $\{303 \rightarrow 42, 1\}$ ,  $\{301 \rightarrow 304, 0\}$ ,  $\{301 \rightarrow 98, 1\}$ ,  $\{304 \rightarrow 305, 0\}$ ,  
 $\{304 \rightarrow 102, 1\}$ ,  $\{305 \rightarrow 305, 0\}$ ,  $\{305 \rightarrow 117, 1\}$ ,  $\{302 \rightarrow 304, 0\}$ ,  $\{302 \rightarrow 127, 1\}$ ,  
 $\{283 \rightarrow 263, 0\}$ ,  $\{283 \rightarrow 101, 1\}$ ,  $\{306 \rightarrow 268, 0\}$ ,  $\{306 \rightarrow 112, 1\}$ ,  $\{307 \rightarrow 290, 0\}$ ,  
 $\{307 \rightarrow 59, 1\}$ ,  $\{308 \rightarrow 232, 0\}$ ,  $\{308 \rightarrow 108, 1\}$ ,  $\{309 \rightarrow 234, 0\}$ ,  $\{309 \rightarrow 46, 1\}$ ,  
 $\{310 \rightarrow 265, 0\}$ ,  $\{310 \rightarrow 44, 1\}$ ,  $\{311 \rightarrow 288, 0\}$ ,  $\{311 \rightarrow 16, 1\}$ ,  $\{63 \rightarrow 286, 0\}$ ,  
 $\{63 \rightarrow 63, 1\}$ ,  $\{133 \rightarrow 295, 0\}$ ,  $\{133 \rightarrow 63, 1\}$ ,  $\{312 \rightarrow 297, 0\}$ ,  $\{312 \rightarrow 133, 1\}$ ,  
 $\{313 \rightarrow 286, 0\}$ ,  $\{313 \rightarrow 67, 1\}$ ,  $\{314 \rightarrow 298, 0\}$ ,  $\{314 \rightarrow 133, 1\}$ ,  $\{229 \rightarrow 290, 0\}$ ,  
 $\{229 \rightarrow 65, 1\}$ ,  $\{315 \rightarrow 290, 0\}$ ,  $\{315 \rightarrow 69, 1\}$ ,  $\{99 \rightarrow 307, 0\}$ ,  $\{99 \rightarrow 312, 1\}$ ,  
 $\{67 \rightarrow 304, 0\}$ ,  $\{67 \rightarrow 312, 1\}$ ,  $\{123 \rightarrow 309, 0\}$ ,  $\{123 \rightarrow 314, 1\}$ ,  $\{126 \rightarrow 310, 0\}$ ,  
 $\{126 \rightarrow 314, 1\}$ ,  $\{278 \rightarrow 288, 0\}$ ,  $\{278 \rightarrow 88, 1\}$ ,  $\{316 \rightarrow 288, 0\}$ ,  $\{316 \rightarrow 86, 1\}$ ,  
 $\{317 \rightarrow 291, 0\}$ ,  $\{317 \rightarrow 91, 1\}$ ,  $\{273 \rightarrow 291, 0\}$ ,  $\{273 \rightarrow 93, 1\}$ ,  $\{75 \rightarrow 228, 0\}$ ,  
 $\{75 \rightarrow 93, 1\}$ ,  $\{65 \rightarrow 230, 0\}$ ,  $\{65 \rightarrow 107, 1\}$ ,  $\{81 \rightarrow 240, 0\}$ ,  $\{81 \rightarrow 107, 1\}$ ,  
 $\{97 \rightarrow 242, 0\}$ ,  $\{97 \rightarrow 93, 1\}$ ,  $\{132 \rightarrow 269, 0\}$ ,  $\{132 \rightarrow 318, 1\}$ ,  $\{69 \rightarrow 267, 0\}$ ,  
 $\{69 \rightarrow 318, 1\}$ ,  $\{319 \rightarrow 277, 0\}$ ,  $\{319 \rightarrow 320, 1\}$ ,  $\{321 \rightarrow 279, 0\}$ ,  $\{321 \rightarrow 320, 1\}$ ,  
 $\{271 \rightarrow 235, 0\}$ ,  $\{271 \rightarrow 133, 1\}$ ,  $\{274 \rightarrow 263, 0\}$ ,  $\{274 \rightarrow 314, 1\}$ ,  $\{276 \rightarrow 301, 0\}$ ,  
 $\{276 \rightarrow 320, 1\}$ ,  $\{244 \rightarrow 149, 0\}$ ,  $\{244 \rightarrow 292, 1\}$ ,  $\{114 \rightarrow 284, 0\}$ ,  $\{114 \rightarrow 249, 1\}$ ,  
 $\{86 \rightarrow 289, 0\}$ ,  $\{86 \rightarrow 249, 1\}$ ,  $\{322 \rightarrow 299, 0\}$ ,  $\{322 \rightarrow 256, 1\}$ ,  $\{323 \rightarrow 300, 0\}$ ,  
 $\{323 \rightarrow 256, 1\}$ ,  $\{91 \rightarrow 149, 0\}$ ,  $\{91 \rightarrow 219, 1\}$ ,  $\{116 \rightarrow 51, 0\}$ ,  $\{116 \rightarrow 3, 1\}$ ,  
 $\{105 \rightarrow 237, 0\}$ ,  $\{105 \rightarrow 219, 1\}$ ,  $\{118 \rightarrow 3, 0\}$ ,  $\{118 \rightarrow 3, 1\}$ ,  $\{78 \rightarrow 308, 0\}$ ,  
 $\{78 \rightarrow 24, 1\}$ ,  $\{88 \rightarrow 303, 0\}$ ,  $\{88 \rightarrow 135, 1\}$ ,  $\{83 \rightarrow 306, 0\}$ ,  $\{83 \rightarrow 24, 1\}$ ,  
 $\{324 \rightarrow 303, 0\}$ ,  $\{324 \rightarrow 48, 1\}$ ,  $\{95 \rightarrow 311, 0\}$ ,  $\{95 \rightarrow 135, 1\}$ ,  $\{325 \rightarrow 296, 0\}$ ,  
 $\{325 \rightarrow 139, 1\}$ ,  $\{243 \rightarrow 296, 0\}$ ,  $\{243 \rightarrow 140, 1\}$ ,  $\{93 \rightarrow 249, 0\}$ ,  $\{93 \rightarrow 9, 1\}$ ,  
 $\{107 \rightarrow 32, 0\}$ ,  $\{107 \rightarrow 9, 1\}$ ,  $\{318 \rightarrow 157, 0\}$ ,  $\{318 \rightarrow 145, 1\}$ ,  $\{320 \rightarrow 272, 0\}$ ,  
 $\{320 \rightarrow 145, 1\}$ ,  $\{280 \rightarrow 285, 0\}$ ,  $\{280 \rightarrow 147, 1\}$ ,  $\{260 \rightarrow 281, 0\}$ ,  $\{260 \rightarrow 145, 1\}$ ,  
 $\{326 \rightarrow 285, 0\}$ ,  $\{326 \rightarrow 143, 1\}$ ,  $\{327 \rightarrow 281, 0\}$ ,  $\{327 \rightarrow 6, 1\}$ ,  $\{259 \rightarrow 254, 0\}$ ,  
 $\{259 \rightarrow 24, 1\}$ ,  $\{261 \rightarrow 294, 0\}$ ,  $\{261 \rightarrow 3, 1\}$ ,  $\{262 \rightarrow 227, 0\}$ ,  $\{262 \rightarrow 256, 1\}$ ,  
 $\{72 \rightarrow 328, 0\}$ ,  $\{72 \rightarrow 329, 1\}$ ,  $\{220 \rightarrow 330, 0\}$ ,  $\{220 \rightarrow 114, 1\}$ ,  $\{231 \rightarrow 270, 0\}$ ,  
 $\{231 \rightarrow 105, 1\}$ ,  $\{233 \rightarrow 270, 0\}$ ,  $\{233 \rightarrow 107, 1\}$ ,  $\{226 \rightarrow 330, 0\}$ ,  $\{226 \rightarrow 95, 1\}$ ,  
 $\{329 \rightarrow 331, 0\}$ ,  $\{329 \rightarrow 332, 1\}$ ,  $\{332 \rightarrow 333, 0\}$ ,  $\{332 \rightarrow 334, 1\}$ ,  $\{334 \rightarrow 335, 0\}$ ,  
 $\{334 \rightarrow 334, 1\}$ ,  $\{330 \rightarrow 245, 0\}$ ,  $\{330 \rightarrow 133, 1\}$ ,  $\{245 \rightarrow 336, 0\}$ ,  $\{245 \rightarrow 132, 1\}$ ,  
 $\{336 \rightarrow 336, 0\}$ ,  $\{336 \rightarrow 81, 1\}$ ,  $\{270 \rightarrow 245, 0\}$ ,  $\{270 \rightarrow 99, 1\}$ ,  $\{331 \rightarrow 278, 0\}$ ,  
 $\{331 \rightarrow 337, 1\}$ ,  $\{337 \rightarrow 280, 0\}$ ,  $\{337 \rightarrow 123, 1\}$ ,  $\{222 \rightarrow 326, 0\}$ ,  $\{222 \rightarrow 319, 1\}$ ,  
 $\{333 \rightarrow 270, 0\}$ ,  $\{333 \rightarrow 338, 1\}$ ,  $\{335 \rightarrow 266, 0\}$ ,  $\{335 \rightarrow 339, 1\}$ ,  $\{340 \rightarrow 266, 0\}$ ,  
 $\{340 \rightarrow 118, 1\}$ ,  $\{223 \rightarrow 264, 0\}$ ,  $\{223 \rightarrow 322, 1\}$ ,  $\{221 \rightarrow 316, 0\}$ ,  $\{221 \rightarrow 69, 1\}$ ,  
 $\{341 \rightarrow 278, 0\}$ ,  $\{341 \rightarrow 67, 1\}$ ,  $\{246 \rightarrow 317, 0\}$ ,  $\{246 \rightarrow 86, 1\}$ ,  $\{247 \rightarrow 255, 0\}$ ,  
 $\{247 \rightarrow 321, 1\}$ ,  $\{248 \rightarrow 327, 0\}$ ,  $\{248 \rightarrow 323, 1\}$ ,  $\{328 \rightarrow 241, 0\}$ ,  $\{328 \rightarrow 282, 1\}$ ,  
 $\{241 \rightarrow 241, 0\}$ ,  $\{241 \rightarrow 12, 1\}$ ,  $\{342 \rightarrow 343, 0\}$ ,  $\{342 \rightarrow 11, 1\}$ ,  $\{343 \rightarrow 241, 0\}$ ,  
 $\{343 \rightarrow 9, 1\}$ ,  $\{238 \rightarrow 343, 0\}$ ,  $\{238 \rightarrow 14, 1\}$ ,  $\{250 \rightarrow 342, 0\}$ ,  $\{250 \rightarrow 28, 1\}$ ,  
 $\{264 \rightarrow 238, 0\}$ ,  $\{264 \rightarrow 24, 1\}$ ,  $\{266 \rightarrow 238, 0\}$ ,  $\{266 \rightarrow 26, 1\}$ ,  $\{255 \rightarrow 342, 0\}$ ,  
 $\{255 \rightarrow 22, 1\}$ ,  $\{251 \rightarrow 313, 0\}$ ,  $\{251 \rightarrow 237, 1\}$ ,  $\{338 \rightarrow 340, 0\}$ ,  $\{338 \rightarrow 58, 1\}$ ,  
 $\{339 \rightarrow 341, 0\}$ ,  $\{339 \rightarrow 51, 1\}$ ,  $\{236 \rightarrow 315, 0\}$ ,  $\{236 \rightarrow 272, 1\}$ ,  $\{252 \rightarrow 324, 0\}$ ,

```

{252 → 143, 1}, {239 → 325, 0}, {239 → 139, 1}, {257 → 226, 0}, {257 → 275, 1}},
1, {1 → 0, 2 → 0, 3 → 1, 4 → 0, 5 → 0, 6 → 1, 7 → 0, 8 → 0, 9 → 1, 10 → 0, 11 → 1,
12 → 1, 13 → 0, 14 → 1, 15 → 0, 16 → 0, 17 → 0, 18 → 0, 19 → 0, 20 → 1, 21 → 0, 22 → 1,
23 → 0, 24 → 1, 25 → 0, 26 → 1, 27 → 0, 28 → 1, 29 → 0, 30 → 1, 31 → 0, 32 → 1, 33 → 0,
34 → 0, 35 → 1, 36 → 0, 37 → 0, 38 → 0, 39 → 0, 40 → 0, 41 → 0, 42 → 0, 43 → 0,
44 → 0, 45 → 0, 46 → 0, 47 → 0, 48 → 1, 49 → 0, 50 → 0, 51 → 1, 52 → 0, 53 → 0,
54 → 0, 55 → 0, 56 → 0, 57 → 0, 58 → 1, 59 → 0, 60 → 0, 61 → 0, 62 → 0, 63 → 1,
64 → 0, 65 → 1, 66 → 0, 67 → 1, 68 → 0, 69 → 1, 70 → 0, 71 → 0, 72 → 1, 73 → 0,
74 → 0, 75 → 1, 76 → 0, 77 → 0, 78 → 1, 79 → 0, 80 → 0, 81 → 1, 82 → 0, 83 → 1,
84 → 0, 85 → 0, 86 → 1, 87 → 0, 88 → 1, 89 → 0, 90 → 0, 91 → 1, 92 → 0, 93 → 1,
94 → 0, 95 → 1, 96 → 0, 97 → 1, 98 → 0, 99 → 1, 100 → 0, 101 → 0, 102 → 0, 103 → 0,
104 → 0, 105 → 1, 106 → 0, 107 → 1, 108 → 0, 109 → 0, 110 → 0, 111 → 0, 112 → 0,
113 → 0, 114 → 1, 115 → 0, 116 → 1, 117 → 0, 118 → 1, 119 → 0, 120 → 0, 121 → 0,
122 → 0, 123 → 1, 124 → 0, 125 → 0, 126 → 1, 127 → 0, 128 → 0, 129 → 0, 130 → 0,
131 → 0, 132 → 1, 133 → 1, 134 → 0, 135 → 1, 136 → 0, 137 → 0, 138 → 0, 139 → 1,
140 → 1, 141 → 0, 142 → 0, 143 → 1, 144 → 0, 145 → 1, 146 → 0, 147 → 1, 148 → 0,
149 → 1, 150 → 0, 151 → 0, 152 → 1, 153 → 0, 154 → 1, 155 → 0, 156 → 0, 157 → 1,
158 → 0, 159 → 0, 160 → 0, 161 → 0, 162 → 0, 163 → 0, 164 → 0, 165 → 0, 166 → 0,
167 → 0, 168 → 0, 169 → 0, 170 → 0, 171 → 0, 172 → 0, 173 → 0, 174 → 0, 175 → 0,
176 → 0, 177 → 0, 178 → 0, 179 → 0, 180 → 0, 181 → 0, 182 → 0, 183 → 0, 184 → 0,
185 → 0, 186 → 0, 187 → 0, 188 → 0, 189 → 0, 190 → 0, 191 → 0, 192 → 0, 193 → 0,
194 → 0, 195 → 0, 196 → 0, 197 → 0, 198 → 0, 199 → 0, 200 → 0, 201 → 0, 202 → 0,
203 → 0, 204 → 0, 205 → 0, 206 → 0, 207 → 0, 208 → 0, 209 → 0, 210 → 0, 211 → 0,
212 → 0, 213 → 0, 214 → 0, 215 → 0, 216 → 0, 217 → 0, 218 → 0, 219 → 1, 220 → 1,
221 → 1, 222 → 1, 223 → 1, 224 → 1, 225 → 1, 226 → 1, 227 → 1, 228 → 1, 229 → 1,
230 → 1, 231 → 1, 232 → 1, 233 → 1, 234 → 1, 235 → 1, 236 → 1, 237 → 1, 238 → 1,
239 → 1, 240 → 1, 241 → 1, 242 → 1, 243 → 1, 244 → 1, 245 → 1, 246 → 1, 247 → 1,
248 → 1, 249 → 1, 250 → 1, 251 → 1, 252 → 1, 253 → 1, 254 → 1, 255 → 1, 256 → 1,
257 → 1, 258 → 1, 259 → 1, 260 → 1, 261 → 1, 262 → 1, 263 → 1, 264 → 1, 265 → 1,
266 → 1, 267 → 1, 268 → 1, 269 → 1, 270 → 1, 271 → 1, 272 → 1, 273 → 1, 274 → 1,
275 → 1, 276 → 1, 277 → 1, 278 → 1, 279 → 1, 280 → 1, 281 → 1, 282 → 1, 283 → 1,
284 → 1, 285 → 1, 286 → 1, 287 → 1, 288 → 1, 289 → 1, 290 → 1, 291 → 1, 292 → 1,
293 → 1, 294 → 1, 295 → 1, 296 → 1, 297 → 1, 298 → 1, 299 → 1, 300 → 1, 301 → 1,
302 → 1, 303 → 1, 304 → 1, 305 → 1, 306 → 1, 307 → 1, 308 → 1, 309 → 1, 310 → 1,
311 → 1, 312 → 1, 313 → 1, 314 → 1, 315 → 1, 316 → 1, 317 → 1, 318 → 1, 319 → 1,
320 → 1, 321 → 1, 322 → 1, 323 → 1, 324 → 1, 325 → 1, 326 → 1, 327 → 1, 328 → 1,
329 → 1, 330 → 1, 331 → 1, 332 → 1, 333 → 1, 334 → 1, 335 → 1, 336 → 1, 337 → 1,
338 → 1, 339 → 1, 340 → 1, 341 → 1, 342 → 1, 343 → 1}, InputAlphabet → {0, 1}]

```

```

In[ ]:= edge[x_, ___] := {Arrowheads[0.015], Arrow[x, 0.1]}

```

```

AutomatonGraph[automatonsigma83, VertexSize → 0.3, EdgeShapeFunction → edge]

```

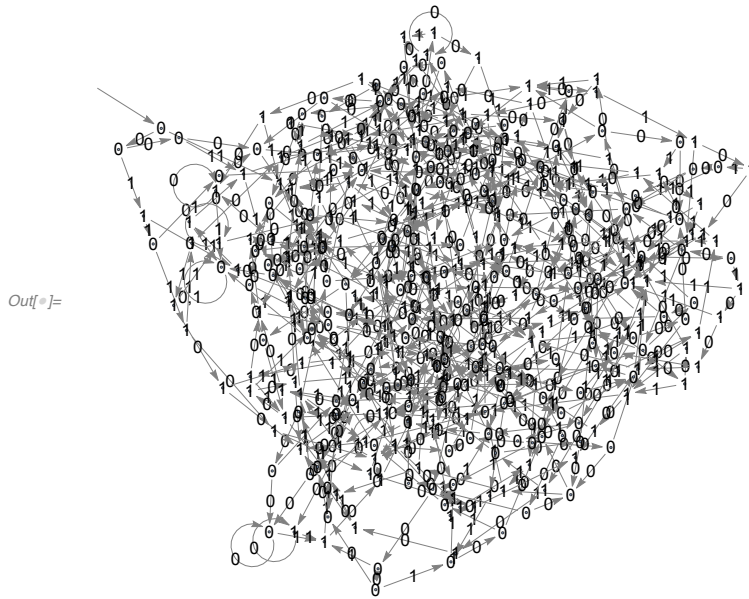

$\sigma_{8,2}$

`fsigma82[t_, s_] :=`

```

s^6*t+s^5*t+s^5+s^4*t^5+s^4*t^3+s^3*t^5+s^3*t+s^3+s^2*t^6+
s^2*t^5+s^2*t^4+s^2*t^3+s^2*t+s*t^4+s*t^2+t^4+t^3;

```

`initsigma82[t_] := t+t^2+t^5+t^9+t^11+0[t]^12`

`automatonsigma82 = AutomaticSequenceAutomaton[`

`AutomaticSequenceReduce[AlgebraicSequence[SeriesRoot[`

`{Function[s, fsigma82[t, s]], initsigma82[t]], Modulus -> 2}][n], n]]`

Out[\*]= Automaton[{ {1 -> 2, 0}, {1 -> 3, 1}, {4 -> 5, 0}, {4 -> 6, 1}, {7 -> 8, 0}, {7 -> 9, 1}, {10 -> 11, 0}, {10 -> 9, 1}, {12 -> 13, 0}, {12 -> 14, 1}, {15 -> 13, 0}, {15 -> 16, 1}, {17 -> 18, 0}, {17 -> 19, 1}, {20 -> 21, 0}, {20 -> 14, 1}, {22 -> 23, 0}, {22 -> 19, 1}, {24 -> 25, 0}, {24 -> 6, 1}, {26 -> 5, 0}, {26 -> 27, 1}, {28 -> 29, 0}, {28 -> 30, 1}, {31 -> 32, 0}, {31 -> 33, 1}, {34 -> 32, 0}, {34 -> 35, 1}, {36 -> 29, 0}, {36 -> 37, 1}, {38 -> 39, 0}, {38 -> 40, 1}, {41 -> 42, 0}, {41 -> 43, 1}, {44 -> 45, 0}, {44 -> 46, 1}, {47 -> 48, 0}, {47 -> 49, 1}, {50 -> 45, 0}, {50 -> 49, 1}, {51 -> 52, 0}, {51 -> 53, 1}, {54 -> 55, 0}, {54 -> 43, 1}, {56 -> 52, 0}, {56 -> 57, 1}, {58 -> 59, 0}, {58 -> 53, 1}, {60 -> 61, 0}, {60 -> 40, 1}, {29 -> 62, 0}, {29 -> 63, 1}, {62 -> 64, 0}, {62 -> 9, 1}, {65 -> 4, 0}, {65 -> 6, 1}, {66 -> 67, 0}, {66 -> 19, 1}, {32 -> 62, 0}, {32 -> 19, 1}, {64 -> 64, 0}, {64 -> 68, 1}, {69 -> 44, 0}, {69 -> 14, 1}, {70 -> 50, 0}, {70 -> 6, 1}, {71 -> 72, 0}, {71 -> 9, 1}, {73 -> 26, 0}, {73 -> 14, 1}, {74 -> 75, 0}, {74 -> 49, 1}, {67 -> 76, 0}, {67 -> 40, 1}, {77 -> 78, 0}, {77 -> 79, 1}, {80 -> 81, 0}, {80 -> 53, 1}, {82 -> 83, 0}, {82 -> 43, 1}, {84 -> 85, 0}, {84 -> 40, 1}, {86 -> 78, 0}, {86 -> 43, 1}, {72 -> 76, 0}, {72 -> 87, 1}, {88 -> 89, 0}, {88 -> 49, 1}, {90 -> 91, 0}, {90 -> 53, 1}, {92 -> 93, 0}, {92 -> 94, 1}, {95 -> 93, 0}, {95 -> 96, 1}, {97 -> 98, 0}, {97 -> 99, 1}, {100 -> 98, 0}, {100 -> 101, 1}, {102 -> 103, 0}, {102 -> 104, 1}, {105 -> 106, 0}, {105 -> 107, 1}, {108 -> 103, 0}, {108 -> 109, 1}, {110 -> 106, 0}, {110 -> 111, 1}, {112 -> 113, 0}, {112 -> 114, 1}, {115 -> 116, 0}, {115 -> 117, 1}, {118 -> 113, 0}, {118 -> 119, 1}, {120 -> 116, 0}, {120 -> 121, 1}, {2 -> 122, 0}, {2 -> 123, 1}, {124 -> 125, 0},

$\{124 \rightarrow 126, 1\}, \{127 \rightarrow 128, 0\}, \{127 \rightarrow 129, 1\}, \{130 \rightarrow 131, 0\}, \{130 \rightarrow 132, 1\},$   
 $\{133 \rightarrow 131, 0\}, \{133 \rightarrow 134, 1\}, \{135 \rightarrow 136, 0\}, \{135 \rightarrow 132, 1\}, \{21 \rightarrow 137, 0\},$   
 $\{21 \rightarrow 138, 1\}, \{25 \rightarrow 137, 0\}, \{25 \rightarrow 139, 1\}, \{140 \rightarrow 141, 0\}, \{140 \rightarrow 139, 1\},$   
 $\{142 \rightarrow 143, 0\}, \{142 \rightarrow 129, 1\}, \{144 \rightarrow 145, 0\}, \{144 \rightarrow 126, 1\}, \{146 \rightarrow 147, 0\},$   
 $\{146 \rightarrow 148, 1\}, \{149 \rightarrow 147, 0\}, \{149 \rightarrow 150, 1\}, \{151 \rightarrow 152, 0\}, \{151 \rightarrow 153, 1\},$   
 $\{154 \rightarrow 152, 0\}, \{154 \rightarrow 155, 1\}, \{13 \rightarrow 156, 0\}, \{13 \rightarrow 157, 1\}, \{113 \rightarrow 158, 0\},$   
 $\{113 \rightarrow 159, 1\}, \{5 \rightarrow 156, 0\}, \{5 \rightarrow 160, 1\}, \{161 \rightarrow 162, 0\}, \{161 \rightarrow 163, 1\},$   
 $\{116 \rightarrow 158, 0\}, \{116 \rightarrow 164, 1\}, \{165 \rightarrow 166, 0\}, \{165 \rightarrow 163, 1\}, \{167 \rightarrow 168, 0\},$   
 $\{167 \rightarrow 169, 1\}, \{170 \rightarrow 171, 0\}, \{170 \rightarrow 160, 1\}, \{172 \rightarrow 173, 0\}, \{172 \rightarrow 169, 1\},$   
 $\{174 \rightarrow 175, 0\}, \{174 \rightarrow 164, 1\}, \{176 \rightarrow 177, 0\}, \{176 \rightarrow 132, 1\}, \{11 \rightarrow 178, 0\},$   
 $\{11 \rightarrow 179, 1\}, \{180 \rightarrow 181, 0\}, \{180 \rightarrow 129, 1\}, \{182 \rightarrow 183, 0\}, \{182 \rightarrow 139, 1\},$   
 $\{184 \rightarrow 181, 0\}, \{184 \rightarrow 185, 1\}, \{18 \rightarrow 178, 0\}, \{18 \rightarrow 126, 1\}, \{186 \rightarrow 187, 0\},$   
 $\{186 \rightarrow 139, 1\}, \{188 \rightarrow 189, 0\}, \{188 \rightarrow 129, 1\}, \{190 \rightarrow 191, 0\}, \{190 \rightarrow 132, 1\},$   
 $\{192 \rightarrow 193, 0\}, \{192 \rightarrow 126, 1\}, \{194 \rightarrow 195, 0\}, \{194 \rightarrow 164, 1\}, \{8 \rightarrow 196, 0\},$   
 $\{8 \rightarrow 197, 1\}, \{198 \rightarrow 199, 0\}, \{198 \rightarrow 164, 1\}, \{200 \rightarrow 201, 0\}, \{200 \rightarrow 160, 1\},$   
 $\{202 \rightarrow 203, 0\}, \{202 \rightarrow 163, 1\}, \{204 \rightarrow 205, 0\}, \{204 \rightarrow 169, 1\}, \{206 \rightarrow 207, 0\},$   
 $\{206 \rightarrow 160, 1\}, \{208 \rightarrow 209, 0\}, \{208 \rightarrow 163, 1\}, \{23 \rightarrow 196, 0\}, \{23 \rightarrow 169, 1\},$   
 $\{210 \rightarrow 203, 0\}, \{210 \rightarrow 211, 1\}, \{212 \rightarrow 213, 0\}, \{212 \rightarrow 214, 1\}, \{215 \rightarrow 216, 0\},$   
 $\{215 \rightarrow 217, 1\}, \{218 \rightarrow 213, 0\}, \{218 \rightarrow 219, 1\}, \{220 \rightarrow 216, 0\}, \{220 \rightarrow 221, 1\},$   
 $\{222 \rightarrow 223, 0\}, \{222 \rightarrow 224, 1\}, \{225 \rightarrow 226, 0\}, \{225 \rightarrow 227, 1\}, \{228 \rightarrow 223, 0\},$   
 $\{228 \rightarrow 229, 1\}, \{230 \rightarrow 226, 0\}, \{230 \rightarrow 231, 1\}, \{232 \rightarrow 233, 0\}, \{232 \rightarrow 234, 1\},$   
 $\{235 \rightarrow 236, 0\}, \{235 \rightarrow 237, 1\}, \{238 \rightarrow 236, 0\}, \{238 \rightarrow 239, 1\}, \{240 \rightarrow 233, 0\},$   
 $\{240 \rightarrow 241, 1\}, \{242 \rightarrow 146, 0\}, \{242 \rightarrow 243, 1\}, \{78 \rightarrow 244, 0\}, \{78 \rightarrow 245, 1\},$   
 $\{106 \rightarrow 246, 0\}, \{106 \rightarrow 247, 1\}, \{248 \rightarrow 249, 0\}, \{248 \rightarrow 250, 1\}, \{251 \rightarrow 252, 0\},$   
 $\{251 \rightarrow 253, 1\}, \{76 \rightarrow 244, 0\}, \{76 \rightarrow 254, 1\}, \{255 \rightarrow 256, 0\}, \{255 \rightarrow 257, 1\},$   
 $\{103 \rightarrow 246, 0\}, \{103 \rightarrow 257, 1\}, \{258 \rightarrow 259, 0\}, \{258 \rightarrow 250, 1\}, \{260 \rightarrow 261, 0\},$   
 $\{260 \rightarrow 254, 1\}, \{262 \rightarrow 263, 0\}, \{262 \rightarrow 253, 1\}, \{264 \rightarrow 265, 0\}, \{264 \rightarrow 254, 1\},$   
 $\{266 \rightarrow 267, 0\}, \{266 \rightarrow 254, 1\}, \{268 \rightarrow 269, 0\}, \{268 \rightarrow 253, 1\}, \{81 \rightarrow 270, 0\},$   
 $\{81 \rightarrow 250, 1\}, \{271 \rightarrow 272, 0\}, \{271 \rightarrow 250, 1\}, \{273 \rightarrow 269, 0\}, \{273 \rightarrow 274, 1\},$   
 $\{275 \rightarrow 276, 0\}, \{275 \rightarrow 257, 1\}, \{277 \rightarrow 278, 0\}, \{277 \rightarrow 253, 1\}, \{279 \rightarrow 280, 0\},$   
 $\{279 \rightarrow 257, 1\}, \{89 \rightarrow 270, 0\}, \{89 \rightarrow 281, 1\}, \{282 \rightarrow 92, 0\}, \{282 \rightarrow 283, 1\},$   
 $\{284 \rightarrow 95, 0\}, \{284 \rightarrow 285, 1\}, \{286 \rightarrow 31, 0\}, \{286 \rightarrow 287, 1\}, \{85 \rightarrow 34, 0\},$   
 $\{85 \rightarrow 288, 1\}, \{289 \rightarrow 105, 0\}, \{289 \rightarrow 288, 1\}, \{290 \rightarrow 112, 0\}, \{290 \rightarrow 283, 1\},$   
 $\{291 \rightarrow 31, 0\}, \{291 \rightarrow 292, 1\}, \{83 \rightarrow 34, 0\}, \{83 \rightarrow 293, 1\}, \{294 \rightarrow 118, 0\},$   
 $\{294 \rightarrow 285, 1\}, \{295 \rightarrow 110, 0\}, \{295 \rightarrow 287, 1\}, \{244 \rightarrow 296, 0\}, \{244 \rightarrow 297, 1\},$   
 $\{246 \rightarrow 296, 0\}, \{246 \rightarrow 298, 1\}, \{296 \rightarrow 299, 0\}, \{296 \rightarrow 300, 1\}, \{299 \rightarrow 299, 0\},$   
 $\{299 \rightarrow 301, 1\}, \{75 \rightarrow 146, 0\}, \{75 \rightarrow 302, 1\}, \{303 \rightarrow 215, 0\}, \{303 \rightarrow 287, 1\},$   
 $\{91 \rightarrow 146, 0\}, \{91 \rightarrow 285, 1\}, \{304 \rightarrow 149, 0\}, \{304 \rightarrow 283, 1\}, \{305 \rightarrow 232, 0\},$   
 $\{305 \rightarrow 287, 1\}, \{306 \rightarrow 220, 0\}, \{306 \rightarrow 288, 1\}, \{307 \rightarrow 149, 0\}, \{307 \rightarrow 308, 1\},$   
 $\{309 \rightarrow 225, 0\}, \{309 \rightarrow 285, 1\}, \{310 \rightarrow 230, 0\}, \{310 \rightarrow 283, 1\}, \{311 \rightarrow 240, 0\},$   
 $\{311 \rightarrow 288, 1\}, \{249 \rightarrow 151, 0\}, \{249 \rightarrow 312, 1\}, \{252 \rightarrow 151, 0\}, \{252 \rightarrow 313, 1\},$   
 $\{314 \rightarrow 154, 0\}, \{314 \rightarrow 315, 1\}, \{316 \rightarrow 154, 0\}, \{316 \rightarrow 317, 1\}, \{256 \rightarrow 28, 0\},$   
 $\{256 \rightarrow 318, 1\}, \{261 \rightarrow 28, 0\}, \{261 \rightarrow 319, 1\}, \{320 \rightarrow 36, 0\}, \{320 \rightarrow 321, 1\},$   
 $\{322 \rightarrow 36, 0\}, \{322 \rightarrow 323, 1\}, \{324 \rightarrow 325, 0\}, \{324 \rightarrow 326, 1\}, \{259 \rightarrow 327, 0\},$   
 $\{259 \rightarrow 328, 1\}, \{329 \rightarrow 325, 0\}, \{329 \rightarrow 330, 1\}, \{263 \rightarrow 327, 0\}, \{263 \rightarrow 331, 1\},$   
 $\{332 \rightarrow 333, 0\}, \{332 \rightarrow 334, 1\}, \{335 \rightarrow 336, 0\}, \{335 \rightarrow 337, 1\}, \{338 \rightarrow 339, 0\},$   
 $\{338 \rightarrow 337, 1\}, \{340 \rightarrow 341, 0\}, \{340 \rightarrow 342, 1\}, \{48 \rightarrow 343, 0\}, \{48 \rightarrow 344, 1\},$

$\{345 \rightarrow 346, 0\}, \{345 \rightarrow 347, 1\}, \{348 \rightarrow 349, 0\}, \{348 \rightarrow 350, 1\}, \{351 \rightarrow 352, 0\},$   
 $\{351 \rightarrow 347, 1\}, \{353 \rightarrow 349, 0\}, \{353 \rightarrow 354, 1\}, \{59 \rightarrow 343, 0\}, \{59 \rightarrow 342, 1\},$   
 $\{355 \rightarrow 356, 0\}, \{355 \rightarrow 350, 1\}, \{357 \rightarrow 358, 0\}, \{357 \rightarrow 359, 1\}, \{360 \rightarrow 361, 0\},$   
 $\{360 \rightarrow 359, 1\}, \{362 \rightarrow 363, 0\}, \{362 \rightarrow 364, 1\}, \{365 \rightarrow 363, 0\}, \{365 \rightarrow 366, 1\},$   
 $\{367 \rightarrow 368, 0\}, \{367 \rightarrow 369, 1\}, \{42 \rightarrow 370, 0\}, \{42 \rightarrow 371, 1\}, \{372 \rightarrow 373, 0\},$   
 $\{372 \rightarrow 374, 1\}, \{61 \rightarrow 370, 0\}, \{61 \rightarrow 369, 1\}, \{375 \rightarrow 376, 0\}, \{375 \rightarrow 364, 1\},$   
 $\{377 \rightarrow 378, 0\}, \{377 \rightarrow 374, 1\}, \{39 \rightarrow 379, 0\}, \{39 \rightarrow 347, 1\}, \{380 \rightarrow 381, 0\},$   
 $\{380 \rightarrow 350, 1\}, \{382 \rightarrow 383, 0\}, \{382 \rightarrow 337, 1\}, \{384 \rightarrow 385, 0\}, \{384 \rightarrow 342, 1\},$   
 $\{55 \rightarrow 379, 0\}, \{55 \rightarrow 386, 1\}, \{387 \rightarrow 388, 0\}, \{387 \rightarrow 347, 1\}, \{389 \rightarrow 390, 0\},$   
 $\{389 \rightarrow 337, 1\}, \{391 \rightarrow 392, 0\}, \{391 \rightarrow 342, 1\}, \{393 \rightarrow 394, 0\}, \{393 \rightarrow 350, 1\},$   
 $\{395 \rightarrow 383, 0\}, \{395 \rightarrow 396, 1\}, \{52 \rightarrow 397, 0\}, \{52 \rightarrow 359, 1\}, \{398 \rightarrow 399, 0\},$   
 $\{398 \rightarrow 364, 1\}, \{400 \rightarrow 401, 0\}, \{400 \rightarrow 374, 1\}, \{93 \rightarrow 402, 0\}, \{93 \rightarrow 374, 1\},$   
 $\{98 \rightarrow 402, 0\}, \{98 \rightarrow 403, 1\}, \{45 \rightarrow 397, 0\}, \{45 \rightarrow 404, 1\}, \{405 \rightarrow 406, 0\},$   
 $\{405 \rightarrow 369, 1\}, \{407 \rightarrow 408, 0\}, \{407 \rightarrow 364, 1\}, \{409 \rightarrow 410, 0\}, \{409 \rightarrow 369, 1\},$   
 $\{411 \rightarrow 412, 0\}, \{411 \rightarrow 359, 1\}, \{265 \rightarrow 413, 0\}, \{265 \rightarrow 414, 1\}, \{280 \rightarrow 413, 0\},$   
 $\{280 \rightarrow 415, 1\}, \{416 \rightarrow 417, 0\}, \{416 \rightarrow 418, 1\}, \{419 \rightarrow 417, 0\}, \{419 \rightarrow 420, 1\},$   
 $\{267 \rightarrow 421, 0\}, \{267 \rightarrow 422, 1\}, \{423 \rightarrow 424, 0\}, \{423 \rightarrow 425, 1\}, \{276 \rightarrow 421, 0\},$   
 $\{276 \rightarrow 426, 1\}, \{427 \rightarrow 424, 0\}, \{427 \rightarrow 428, 1\}, \{429 \rightarrow 430, 0\}, \{429 \rightarrow 431, 1\},$   
 $\{272 \rightarrow 432, 0\}, \{272 \rightarrow 433, 1\}, \{278 \rightarrow 432, 0\}, \{278 \rightarrow 434, 1\}, \{435 \rightarrow 430, 0\},$   
 $\{435 \rightarrow 436, 1\}, \{327 \rightarrow 437, 0\}, \{327 \rightarrow 438, 1\}, \{269 \rightarrow 439, 0\}, \{269 \rightarrow 440, 1\},$   
 $\{325 \rightarrow 437, 0\}, \{325 \rightarrow 441, 1\}, \{270 \rightarrow 439, 0\}, \{270 \rightarrow 442, 1\}, \{122 \rightarrow 443, 0\},$   
 $\{122 \rightarrow 444, 1\}, \{397 \rightarrow 131, 0\}, \{397 \rightarrow 445, 1\}, \{439 \rightarrow 137, 0\}, \{439 \rightarrow 152, 1\},$   
 $\{402 \rightarrow 131, 0\}, \{402 \rightarrow 446, 1\}, \{437 \rightarrow 137, 0\}, \{437 \rightarrow 447, 1\}, \{443 \rightarrow 448, 0\},$   
 $\{443 \rightarrow 449, 1\}, \{448 \rightarrow 450, 0\}, \{448 \rightarrow 451, 1\}, \{450 \rightarrow 450, 0\}, \{450 \rightarrow 452, 1\},$   
 $\{453 \rightarrow 216, 0\}, \{453 \rightarrow 454, 1\}, \{454 \rightarrow 455, 0\}, \{454 \rightarrow 454, 1\}, \{456 \rightarrow 457, 0\},$   
 $\{456 \rightarrow 453, 1\}, \{458 \rightarrow 459, 0\}, \{458 \rightarrow 453, 1\}, \{128 \rightarrow 213, 0\}, \{128 \rightarrow 460, 1\},$   
 $\{461 \rightarrow 462, 0\}, \{461 \rightarrow 226, 1\}, \{463 \rightarrow 464, 0\}, \{463 \rightarrow 465, 1\}, \{145 \rightarrow 213, 0\},$   
 $\{145 \rightarrow 465, 1\}, \{466 \rightarrow 216, 0\}, \{466 \rightarrow 467, 1\}, \{468 \rightarrow 469, 0\}, \{468 \rightarrow 226, 1\},$   
 $\{125 \rightarrow 236, 0\}, \{125 \rightarrow 456, 1\}, \{470 \rightarrow 471, 0\}, \{470 \rightarrow 456, 1\}, \{472 \rightarrow 473, 0\},$   
 $\{472 \rightarrow 458, 1\}, \{474 \rightarrow 233, 0\}, \{474 \rightarrow 475, 1\}, \{476 \rightarrow 477, 0\}, \{476 \rightarrow 458, 1\},$   
 $\{478 \rightarrow 479, 0\}, \{478 \rightarrow 480, 1\}, \{467 \rightarrow 481, 0\}, \{467 \rightarrow 475, 1\}, \{143 \rightarrow 236, 0\},$   
 $\{143 \rightarrow 482, 1\}, \{482 \rightarrow 483, 0\}, \{482 \rightarrow 480, 1\}, \{484 \rightarrow 233, 0\}, \{484 \rightarrow 485, 1\},$   
 $\{486 \rightarrow 147, 0\}, \{486 \rightarrow 458, 1\}, \{487 \rightarrow 447, 0\}, \{487 \rightarrow 480, 1\}, \{136 \rightarrow 152, 0\},$   
 $\{136 \rightarrow 480, 1\}, \{488 \rightarrow 446, 0\}, \{488 \rightarrow 475, 1\}, \{460 \rightarrow 489, 0\}, \{460 \rightarrow 458, 1\},$   
 $\{490 \rightarrow 445, 0\}, \{490 \rightarrow 475, 1\}, \{491 \rightarrow 147, 0\}, \{491 \rightarrow 478, 1\}, \{141 \rightarrow 152, 0\},$   
 $\{141 \rightarrow 492, 1\}, \{492 \rightarrow 493, 0\}, \{492 \rightarrow 456, 1\}, \{485 \rightarrow 494, 0\}, \{485 \rightarrow 456, 1\},$   
 $\{226 \rightarrow 226, 0\}, \{226 \rightarrow 226, 1\}, \{480 \rightarrow 474, 0\}, \{480 \rightarrow 465, 1\}, \{131 \rightarrow 223, 0\},$   
 $\{131 \rightarrow 453, 1\}, \{465 \rightarrow 486, 0\}, \{465 \rightarrow 226, 1\}, \{223 \rightarrow 226, 0\}, \{223 \rightarrow 486, 1\},$   
 $\{495 \rightarrow 491, 0\}, \{495 \rightarrow 453, 1\}, \{137 \rightarrow 223, 0\}, \{137 \rightarrow 474, 1\}, \{475 \rightarrow 453, 0\},$   
 $\{475 \rightarrow 465, 1\}, \{496 \rightarrow 466, 0\}, \{496 \rightarrow 454, 1\}, \{497 \rightarrow 484, 0\}, \{497 \rightarrow 454, 1\},$   
 $\{399 \rightarrow 181, 0\}, \{399 \rightarrow 498, 1\}, \{499 \rightarrow 178, 0\}, \{499 \rightarrow 500, 1\}, \{406 \rightarrow 181, 0\},$   
 $\{406 \rightarrow 501, 1\}, \{502 \rightarrow 178, 0\}, \{502 \rightarrow 503, 1\}, \{401 \rightarrow 158, 0\}, \{401 \rightarrow 504, 1\},$   
 $\{505 \rightarrow 156, 0\}, \{505 \rightarrow 506, 1\}, \{507 \rightarrow 156, 0\}, \{507 \rightarrow 508, 1\}, \{412 \rightarrow 158, 0\},$   
 $\{412 \rightarrow 509, 1\}, \{408 \rightarrow 203, 0\}, \{408 \rightarrow 510, 1\}, \{410 \rightarrow 203, 0\}, \{410 \rightarrow 511, 1\},$   
 $\{512 \rightarrow 196, 0\}, \{512 \rightarrow 513, 1\}, \{514 \rightarrow 196, 0\}, \{514 \rightarrow 515, 1\}, \{516 \rightarrow 242, 0\},$   
 $\{516 \rightarrow 332, 1\}, \{471 \rightarrow 296, 0\}, \{471 \rightarrow 367, 1\}, \{517 \rightarrow 314, 0\}, \{517 \rightarrow 39, 1\},$   
 $\{518 \rightarrow 324, 0\}, \{518 \rightarrow 39, 1\}, \{481 \rightarrow 296, 0\}, \{481 \rightarrow 387, 1\}, \{519 \rightarrow 329, 0\},$

$\{519 \rightarrow 59, 1\}, \{520 \rightarrow 320, 0\}, \{520 \rightarrow 340, 1\}, \{209 \rightarrow 299, 0\}, \{209 \rightarrow 340, 1\},$   
 $\{205 \rightarrow 299, 0\}, \{205 \rightarrow 411, 1\}, \{521 \rightarrow 322, 0\}, \{521 \rightarrow 387, 1\}, \{522 \rightarrow 316, 0\},$   
 $\{522 \rightarrow 59, 1\}, \{233 \rightarrow 28, 0\}, \{233 \rightarrow 335, 1\}, \{236 \rightarrow 28, 0\}, \{236 \rightarrow 398, 1\},$   
 $\{203 \rightarrow 36, 0\}, \{203 \rightarrow 380, 1\}, \{523 \rightarrow 102, 0\}, \{523 \rightarrow 380, 1\}, \{524 \rightarrow 97, 0\},$   
 $\{524 \rightarrow 338, 1\}, \{196 \rightarrow 36, 0\}, \{196 \rightarrow 372, 1\}, \{525 \rightarrow 115, 0\}, \{525 \rightarrow 393, 1\},$   
 $\{526 \rightarrow 100, 0\}, \{526 \rightarrow 393, 1\}, \{527 \rightarrow 120, 0\}, \{527 \rightarrow 338, 1\}, \{528 \rightarrow 108, 0\},$   
 $\{528 \rightarrow 335, 1\}, \{383 \rightarrow 31, 0\}, \{383 \rightarrow 176, 1\}, \{421 \rightarrow 34, 0\}, \{421 \rightarrow 127, 1\},$   
 $\{379 \rightarrow 31, 0\}, \{379 \rightarrow 194, 1\}, \{424 \rightarrow 34, 0\}, \{424 \rightarrow 165, 1\}, \{529 \rightarrow 212, 0\},$   
 $\{529 \rightarrow 335, 1\}, \{530 \rightarrow 222, 0\}, \{530 \rightarrow 338, 1\}, \{195 \rightarrow 154, 0\}, \{195 \rightarrow 407, 1\},$   
 $\{531 \rightarrow 218, 0\}, \{531 \rightarrow 380, 1\}, \{201 \rightarrow 154, 0\}, \{201 \rightarrow 338, 1\}, \{532 \rightarrow 235, 0\},$   
 $\{532 \rightarrow 380, 1\}, \{477 \rightarrow 151, 0\}, \{477 \rightarrow 377, 1\}, \{483 \rightarrow 151, 0\}, \{483 \rightarrow 393, 1\},$   
 $\{533 \rightarrow 228, 0\}, \{533 \rightarrow 393, 1\}, \{534 \rightarrow 238, 0\}, \{534 \rightarrow 335, 1\}, \{535 \rightarrow 146, 0\},$   
 $\{535 \rightarrow 198, 1\}, \{381 \rightarrow 149, 0\}, \{381 \rightarrow 161, 1\}, \{536 \rightarrow 146, 0\}, \{536 \rightarrow 190, 1\},$   
 $\{392 \rightarrow 149, 0\}, \{392 \rightarrow 142, 1\}, \{537 \rightarrow 429, 0\}, \{537 \rightarrow 39, 1\}, \{473 \rightarrow 327, 0\},$   
 $\{473 \rightarrow 52, 1\}, \{538 \rightarrow 423, 0\}, \{538 \rightarrow 340, 1\}, \{199 \rightarrow 325, 0\}, \{199 \rightarrow 61, 1\},$   
 $\{539 \rightarrow 435, 0\}, \{539 \rightarrow 59, 1\}, \{207 \rightarrow 325, 0\}, \{207 \rightarrow 39, 1\}, \{479 \rightarrow 327, 0\},$   
 $\{479 \rightarrow 59, 1\}, \{540 \rightarrow 427, 0\}, \{540 \rightarrow 387, 1\}, \{541 \rightarrow 416, 0\}, \{541 \rightarrow 387, 1\},$   
 $\{542 \rightarrow 419, 0\}, \{542 \rightarrow 340, 1\}, \{543 \rightarrow 244, 0\}, \{543 \rightarrow 204, 1\}, \{388 \rightarrow 246, 0\},$   
 $\{388 \rightarrow 170, 1\}, \{390 \rightarrow 246, 0\}, \{390 \rightarrow 140, 1\}, \{544 \rightarrow 244, 0\}, \{544 \rightarrow 192, 1\},$   
 $\{385 \rightarrow 269, 0\}, \{385 \rightarrow 18, 1\}, \{545 \rightarrow 270, 0\}, \{545 \rightarrow 25, 1\}, \{394 \rightarrow 269, 0\},$   
 $\{394 \rightarrow 23, 1\}, \{546 \rightarrow 270, 0\}, \{546 \rightarrow 5, 1\}, \{444 \rightarrow 349, 0\}, \{444 \rightarrow 124, 1\},$   
 $\{349 \rightarrow 349, 0\}, \{349 \rightarrow 38, 1\}, \{432 \rightarrow 343, 0\}, \{432 \rightarrow 74, 1\}, \{343 \rightarrow 349, 0\},$   
 $\{343 \rightarrow 10, 1\}, \{430 \rightarrow 343, 0\}, \{430 \rightarrow 70, 1\}, \{333 \rightarrow 432, 0\}, \{333 \rightarrow 360, 1\},$   
 $\{547 \rightarrow 548, 0\}, \{547 \rightarrow 264, 1\}, \{549 \rightarrow 550, 0\}, \{549 \rightarrow 264, 1\}, \{147 \rightarrow 432, 0\},$   
 $\{147 \rightarrow 284, 1\}, \{551 \rightarrow 552, 0\}, \{551 \rightarrow 266, 1\}, \{156 \rightarrow 430, 0\}, \{156 \rightarrow 266, 1\},$   
 $\{158 \rightarrow 430, 0\}, \{158 \rightarrow 306, 1\}, \{152 \rightarrow 432, 0\}, \{152 \rightarrow 248, 1\}, \{504 \rightarrow 553, 0\},$   
 $\{504 \rightarrow 258, 1\}, \{501 \rightarrow 554, 0\}, \{501 \rightarrow 248, 1\}, \{515 \rightarrow 555, 0\}, \{515 \rightarrow 258, 1\},$   
 $\{336 \rightarrow 383, 0\}, \{336 \rightarrow 65, 1\}, \{550 \rightarrow 379, 0\}, \{550 \rightarrow 7, 1\}, \{346 \rightarrow 383, 0\},$   
 $\{346 \rightarrow 88, 1\}, \{555 \rightarrow 379, 0\}, \{555 \rightarrow 60, 1\}, \{446 \rightarrow 421, 0\}, \{446 \rightarrow 264, 1\},$   
 $\{556 \rightarrow 535, 0\}, \{556 \rightarrow 248, 1\}, \{557 \rightarrow 543, 0\}, \{557 \rightarrow 258, 1\}, \{166 \rightarrow 424, 0\},$   
 $\{166 \rightarrow 258, 1\}, \{506 \rightarrow 545, 0\}, \{506 \rightarrow 266, 1\}, \{511 \rightarrow 536, 0\}, \{511 \rightarrow 266, 1\},$   
 $\{168 \rightarrow 424, 0\}, \{168 \rightarrow 294, 1\}, \{503 \rightarrow 544, 0\}, \{503 \rightarrow 264, 1\}, \{558 \rightarrow 546, 0\},$   
 $\{558 \rightarrow 248, 1\}, \{494 \rightarrow 421, 0\}, \{494 \rightarrow 311, 1\}, \{548 \rightarrow 370, 0\}, \{548 \rightarrow 66, 1\},$   
 $\{553 \rightarrow 370, 0\}, \{553 \rightarrow 82, 1\}, \{339 \rightarrow 363, 0\}, \{339 \rightarrow 20, 1\}, \{352 \rightarrow 363, 0\},$   
 $\{352 \rightarrow 58, 1\}, \{552 \rightarrow 397, 0\}, \{552 \rightarrow 12, 1\}, \{341 \rightarrow 402, 0\}, \{341 \rightarrow 32, 1\},$   
 $\{554 \rightarrow 397, 0\}, \{554 \rightarrow 51, 1\}, \{356 \rightarrow 402, 0\}, \{356 \rightarrow 86, 1\}, \{447 \rightarrow 439, 0\},$   
 $\{447 \rightarrow 268, 1\}, \{498 \rightarrow 505, 0\}, \{498 \rightarrow 268, 1\}, \{559 \rightarrow 499, 0\}, \{559 \rightarrow 255, 1\},$   
 $\{560 \rightarrow 507, 0\}, \{560 \rightarrow 103, 1\}, \{489 \rightarrow 439, 0\}, \{489 \rightarrow 304, 1\}, \{561 \rightarrow 512, 0\},$   
 $\{561 \rightarrow 255, 1\}, \{171 \rightarrow 437, 0\}, \{171 \rightarrow 103, 1\}, \{513 \rightarrow 502, 0\}, \{513 \rightarrow 277, 1\},$   
 $\{509 \rightarrow 514, 0\}, \{509 \rightarrow 277, 1\}, \{175 \rightarrow 437, 0\}, \{175 \rightarrow 286, 1\}, \{445 \rightarrow 413, 0\},$   
 $\{445 \rightarrow 255, 1\}, \{162 \rightarrow 417, 0\}, \{162 \rightarrow 277, 1\}, \{562 \rightarrow 563, 0\}, \{562 \rightarrow 268, 1\},$   
 $\{500 \rightarrow 564, 0\}, \{500 \rightarrow 255, 1\}, \{508 \rightarrow 565, 0\}, \{508 \rightarrow 103, 1\}, \{510 \rightarrow 566, 0\},$   
 $\{510 \rightarrow 103, 1\}, \{567 \rightarrow 568, 0\}, \{567 \rightarrow 277, 1\}, \{569 \rightarrow 570, 0\}, \{569 \rightarrow 268, 1\},$   
 $\{173 \rightarrow 417, 0\}, \{173 \rightarrow 310, 1\}, \{493 \rightarrow 413, 0\}, \{493 \rightarrow 295, 1\}, \{449 \rightarrow 13, 0\},$   
 $\{449 \rightarrow 547, 1\}, \{451 \rightarrow 78, 0\}, \{451 \rightarrow 551, 1\}, \{216 \rightarrow 106, 0\}, \{216 \rightarrow 571, 1\},$   
 $\{571 \rightarrow 286, 0\}, \{571 \rightarrow 572, 1\}, \{213 \rightarrow 106, 0\}, \{213 \rightarrow 573, 1\}, \{574 \rightarrow 304, 0\},$   
 $\{574 \rightarrow 191, 1\}, \{181 \rightarrow 103, 0\}, \{181 \rightarrow 575, 1\}, \{576 \rightarrow 291, 0\}, \{576 \rightarrow 573, 1\},$

$\{577 \rightarrow 307, 0\}, \{577 \rightarrow 193, 1\}, \{578 \rightarrow 273, 0\}, \{578 \rightarrow 193, 1\}, \{178 \rightarrow 103, 0\},$   
 $\{178 \rightarrow 572, 1\}, \{579 \rightarrow 268, 0\}, \{579 \rightarrow 191, 1\}, \{358 \rightarrow 52, 0\}, \{358 \rightarrow 203, 1\},$   
 $\{563 \rightarrow 45, 0\}, \{563 \rightarrow 207, 1\}, \{373 \rightarrow 52, 0\}, \{373 \rightarrow 209, 1\}, \{566 \rightarrow 45, 0\},$   
 $\{566 \rightarrow 201, 1\}, \{452 \rightarrow 62, 0\}, \{452 \rightarrow 556, 1\}, \{580 \rightarrow 362, 0\}, \{580 \rightarrow 572, 1\},$   
 $\{457 \rightarrow 93, 0\}, \{457 \rightarrow 177, 1\}, \{581 \rightarrow 365, 0\}, \{581 \rightarrow 573, 1\}, \{177 \rightarrow 98, 0\},$   
 $\{177 \rightarrow 193, 1\}, \{582 \rightarrow 382, 0\}, \{582 \rightarrow 572, 1\}, \{462 \rightarrow 93, 0\}, \{462 \rightarrow 191, 1\},$   
 $\{575 \rightarrow 353, 0\}, \{575 \rightarrow 193, 1\}, \{583 \rightarrow 348, 0\}, \{583 \rightarrow 191, 1\}, \{183 \rightarrow 98, 0\},$   
 $\{183 \rightarrow 178, 1\}, \{584 \rightarrow 395, 0\}, \{584 \rightarrow 573, 1\}, \{455 \rightarrow 32, 0\}, \{455 \rightarrow 581, 1\},$   
 $\{573 \rightarrow 77, 0\}, \{573 \rightarrow 585, 1\}, \{586 \rightarrow 51, 0\}, \{586 \rightarrow 587, 1\}, \{585 \rightarrow 15, 0\},$   
 $\{585 \rightarrow 588, 1\}, \{193 \rightarrow 29, 0\}, \{193 \rightarrow 585, 1\}, \{588 \rightarrow 56, 0\}, \{588 \rightarrow 588, 1\},$   
 $\{589 \rightarrow 86, 0\}, \{589 \rightarrow 590, 1\}, \{591 \rightarrow 12, 0\}, \{591 \rightarrow 587, 1\}, \{464 \rightarrow 32, 0\},$   
 $\{464 \rightarrow 590, 1\}, \{189 \rightarrow 29, 0\}, \{189 \rightarrow 579, 1\}, \{361 \rightarrow 13, 0\}, \{361 \rightarrow 529, 1\},$   
 $\{565 \rightarrow 5, 0\}, \{565 \rightarrow 526, 1\}, \{378 \rightarrow 13, 0\}, \{378 \rightarrow 540, 1\}, \{570 \rightarrow 5, 0\},$   
 $\{570 \rightarrow 522, 1\}, \{370 \rightarrow 78, 0\}, \{370 \rightarrow 537, 1\}, \{363 \rightarrow 78, 0\}, \{363 \rightarrow 530, 1\},$   
 $\{413 \rightarrow 76, 0\}, \{413 \rightarrow 523, 1\}, \{417 \rightarrow 76, 0\}, \{417 \rightarrow 520, 1\}, \{572 \rightarrow 130, 0\},$   
 $\{572 \rightarrow 587, 1\}, \{459 \rightarrow 113, 0\}, \{459 \rightarrow 574, 1\}, \{587 \rightarrow 180, 0\}, \{587 \rightarrow 590, 1\},$   
 $\{590 \rightarrow 202, 0\}, \{590 \rightarrow 590, 1\}, \{191 \rightarrow 116, 0\}, \{191 \rightarrow 587, 1\}, \{592 \rightarrow 184, 0\},$   
 $\{592 \rightarrow 585, 1\}, \{593 \rightarrow 133, 0\}, \{593 \rightarrow 588, 1\}, \{469 \rightarrow 113, 0\}, \{469 \rightarrow 588, 1\},$   
 $\{594 \rightarrow 210, 0\}, \{594 \rightarrow 585, 1\}, \{187 \rightarrow 116, 0\}, \{187 \rightarrow 584, 1\}, \{368 \rightarrow 62, 0\},$   
 $\{368 \rightarrow 519, 1\}, \{376 \rightarrow 62, 0\}, \{376 \rightarrow 525, 1\}, \{564 \rightarrow 64, 0\}, \{564 \rightarrow 534, 1\},$   
 $\{568 \rightarrow 64, 0\}, \{568 \rightarrow 541, 1\}, \{3 \rightarrow 595, 0\}, \{3 \rightarrow 516, 1\}, \{596 \rightarrow 597, 0\},$   
 $\{596 \rightarrow 549, 1\}, \{598 \rightarrow 597, 0\}, \{598 \rightarrow 559, 1\}, \{599 \rightarrow 600, 0\}, \{599 \rightarrow 562, 1\},$   
 $\{601 \rightarrow 600, 0\}, \{601 \rightarrow 556, 1\}, \{40 \rightarrow 441, 0\}, \{40 \rightarrow 487, 1\}, \{602 \rightarrow 603, 0\},$   
 $\{602 \rightarrow 470, 1\}, \{6 \rightarrow 442, 0\}, \{6 \rightarrow 136, 1\}, \{19 \rightarrow 440, 0\}, \{19 \rightarrow 136, 1\},$   
 $\{604 \rightarrow 438, 0\}, \{604 \rightarrow 495, 1\}, \{605 \rightarrow 603, 0\}, \{605 \rightarrow 463, 1\}, \{606 \rightarrow 607, 0\},$   
 $\{606 \rightarrow 470, 1\}, \{608 \rightarrow 609, 0\}, \{608 \rightarrow 125, 1\}, \{53 \rightarrow 438, 0\}, \{53 \rightarrow 487, 1\},$   
 $\{610 \rightarrow 611, 0\}, \{610 \rightarrow 125, 1\}, \{63 \rightarrow 612, 0\}, \{63 \rightarrow 472, 1\}, \{613 \rightarrow 404, 0\},$   
 $\{613 \rightarrow 490, 1\}, \{614 \rightarrow 374, 0\}, \{614 \rightarrow 488, 1\}, \{615 \rightarrow 403, 0\}, \{615 \rightarrow 488, 1\},$   
 $\{616 \rightarrow 617, 0\}, \{616 \rightarrow 461, 1\}, \{57 \rightarrow 617, 0\}, \{57 \rightarrow 476, 1\}, \{618 \rightarrow 374, 0\},$   
 $\{618 \rightarrow 496, 1\}, \{619 \rightarrow 359, 0\}, \{619 \rightarrow 490, 1\}, \{87 \rightarrow 620, 0\}, \{87 \rightarrow 476, 1\},$   
 $\{27 \rightarrow 621, 0\}, \{27 \rightarrow 472, 1\}, \{9 \rightarrow 622, 0\}, \{9 \rightarrow 470, 1\}, \{49 \rightarrow 623, 0\},$   
 $\{49 \rightarrow 125, 1\}, \{14 \rightarrow 624, 0\}, \{14 \rightarrow 470, 1\}, \{43 \rightarrow 625, 0\}, \{43 \rightarrow 125, 1\},$   
 $\{626 \rightarrow 627, 0\}, \{626 \rightarrow 136, 1\}, \{628 \rightarrow 629, 0\}, \{628 \rightarrow 487, 1\}, \{630 \rightarrow 631, 0\},$   
 $\{630 \rightarrow 136, 1\}, \{632 \rightarrow 633, 0\}, \{632 \rightarrow 487, 1\}, \{634 \rightarrow 623, 0\}, \{634 \rightarrow 145, 1\},$   
 $\{635 \rightarrow 631, 0\}, \{635 \rightarrow 131, 1\}, \{636 \rightarrow 637, 0\}, \{636 \rightarrow 156, 1\}, \{638 \rightarrow 328, 0\},$   
 $\{638 \rightarrow 162, 1\}, \{639 \rightarrow 328, 0\}, \{639 \rightarrow 166, 1\}, \{640 \rightarrow 637, 0\}, \{640 \rightarrow 171, 1\},$   
 $\{641 \rightarrow 642, 0\}, \{641 \rightarrow 551, 1\}, \{643 \rightarrow 644, 0\}, \{643 \rightarrow 557, 1\}, \{645 \rightarrow 642, 0\},$   
 $\{645 \rightarrow 560, 1\}, \{646 \rightarrow 644, 0\}, \{646 \rightarrow 567, 1\}, \{68 \rightarrow 647, 0\}, \{68 \rightarrow 488, 1\},$   
 $\{648 \rightarrow 649, 0\}, \{648 \rightarrow 476, 1\}, \{650 \rightarrow 651, 0\}, \{650 \rightarrow 472, 1\}, \{46 \rightarrow 652, 0\},$   
 $\{46 \rightarrow 490, 1\}, \{79 \rightarrow 653, 0\}, \{79 \rightarrow 490, 1\}, \{654 \rightarrow 655, 0\}, \{654 \rightarrow 476, 1\},$   
 $\{16 \rightarrow 656, 0\}, \{16 \rightarrow 488, 1\}, \{657 \rightarrow 658, 0\}, \{657 \rightarrow 472, 1\}, \{659 \rightarrow 651, 0\},$   
 $\{659 \rightarrow 468, 1\}, \{660 \rightarrow 652, 0\}, \{660 \rightarrow 497, 1\}, \{661 \rightarrow 662, 0\}, \{661 \rightarrow 561, 1\},$   
 $\{663 \rightarrow 662, 0\}, \{663 \rightarrow 547, 1\}, \{664 \rightarrow 281, 0\}, \{664 \rightarrow 569, 1\}, \{665 \rightarrow 281, 0\},$   
 $\{665 \rightarrow 558, 1\}, \{123 \rightarrow 666, 0\}, \{123 \rightarrow 233, 1\}, \{667 \rightarrow 668, 0\}, \{667 \rightarrow 517, 1\},$   
 $\{669 \rightarrow 670, 0\}, \{669 \rightarrow 538, 1\}, \{671 \rightarrow 668, 0\}, \{671 \rightarrow 524, 1\}, \{672 \rightarrow 670, 0\},$   
 $\{672 \rightarrow 531, 1\}, \{666 \rightarrow 673, 0\}, \{666 \rightarrow 453, 1\}, \{673 \rightarrow 674, 0\}, \{673 \rightarrow 486, 1\},$   
 $\{674 \rightarrow 674, 0\}, \{674 \rightarrow 226, 1\}, \{675 \rightarrow 666, 0\}, \{675 \rightarrow 446, 1\}, \{126 \rightarrow 602, 0\},$



$\{126 \rightarrow 580, 1\}$ ,  $\{132 \rightarrow 614, 0\}$ ,  $\{132 \rightarrow 580, 1\}$ ,  $\{676 \rightarrow 605, 0\}$ ,  $\{676 \rightarrow 578, 1\}$ ,  
 $\{160 \rightarrow 630, 0\}$ ,  $\{160 \rightarrow 582, 1\}$ ,  $\{677 \rightarrow 618, 0\}$ ,  $\{677 \rightarrow 591, 1\}$ ,  $\{163 \rightarrow 650, 0\}$ ,  
 $\{163 \rightarrow 582, 1\}$ ,  $\{678 \rightarrow 659, 0\}$ ,  $\{678 \rightarrow 577, 1\}$ ,  $\{679 \rightarrow 618, 0\}$ ,  $\{679 \rightarrow 578, 1\}$ ,  
 $\{680 \rightarrow 614, 0\}$ ,  $\{680 \rightarrow 594, 1\}$ ,  $\{681 \rightarrow 635, 0\}$ ,  $\{681 \rightarrow 577, 1\}$ ,  $\{157 \rightarrow 682, 0\}$ ,  
 $\{157 \rightarrow 213, 1\}$ ,  $\{683 \rightarrow 684, 0\}$ ,  $\{683 \rightarrow 462, 1\}$ ,  $\{685 \rightarrow 686, 0\}$ ,  $\{685 \rightarrow 593, 1\}$ ,  
 $\{687 \rightarrow 688, 0\}$ ,  $\{687 \rightarrow 583, 1\}$ ,  $\{179 \rightarrow 689, 0\}$ ,  $\{179 \rightarrow 576, 1\}$ ,  $\{690 \rightarrow 686, 0\}$ ,  
 $\{690 \rightarrow 583, 1\}$ ,  $\{691 \rightarrow 692, 0\}$ ,  $\{691 \rightarrow 589, 1\}$ ,  $\{134 \rightarrow 692, 0\}$ ,  $\{134 \rightarrow 576, 1\}$ ,  
 $\{693 \rightarrow 694, 0\}$ ,  $\{693 \rightarrow 462, 1\}$ ,  $\{211 \rightarrow 695, 0\}$ ,  $\{211 \rightarrow 213, 1\}$ ,  $\{696 \rightarrow 138, 0\}$ ,  
 $\{696 \rightarrow 582, 1\}$ ,  $\{697 \rightarrow 697, 0\}$ ,  $\{697 \rightarrow 586, 1\}$ ,  $\{129 \rightarrow 698, 0\}$ ,  $\{129 \rightarrow 577, 1\}$ ,  
 $\{668 \rightarrow 139, 0\}$ ,  $\{668 \rightarrow 582, 1\}$ ,  $\{670 \rightarrow 139, 0\}$ ,  $\{670 \rightarrow 592, 1\}$ ,  $\{164 \rightarrow 691, 0\}$ ,  
 $\{164 \rightarrow 578, 1\}$ ,  $\{139 \rightarrow 697, 0\}$ ,  $\{139 \rightarrow 577, 1\}$ ,  $\{699 \rightarrow 132, 0\}$ ,  $\{699 \rightarrow 580, 1\}$ ,  
 $\{169 \rightarrow 680, 0\}$ ,  $\{169 \rightarrow 578, 1\}$ ,  $\{700 \rightarrow 134, 0\}$ ,  $\{700 \rightarrow 580, 1\}$ ,  $\{701 \rightarrow 702, 0\}$ ,  
 $\{701 \rightarrow 233, 1\}$ ,  $\{703 \rightarrow 702, 0\}$ ,  $\{703 \rightarrow 481, 1\}$ ,  $\{704 \rightarrow 705, 0\}$ ,  $\{704 \rightarrow 483, 1\}$ ,  
 $\{706 \rightarrow 705, 0\}$ ,  $\{706 \rightarrow 479, 1\}$ ,  $\{707 \rightarrow 708, 0\}$ ,  $\{707 \rightarrow 213, 1\}$ ,  $\{709 \rightarrow 710, 0\}$ ,  
 $\{709 \rightarrow 576, 1\}$ ,  $\{138 \rightarrow 227, 0\}$ ,  $\{138 \rightarrow 462, 1\}$ ,  $\{159 \rightarrow 229, 0\}$ ,  $\{159 \rightarrow 583, 1\}$ ,  
 $\{698 \rightarrow 227, 0\}$ ,  $\{698 \rightarrow 469, 1\}$ ,  $\{197 \rightarrow 224, 0\}$ ,  $\{197 \rightarrow 583, 1\}$ ,  $\{711 \rightarrow 712, 0\}$ ,  
 $\{711 \rightarrow 576, 1\}$ ,  $\{713 \rightarrow 714, 0\}$ ,  $\{713 \rightarrow 213, 1\}$ ,  $\{185 \rightarrow 231, 0\}$ ,  $\{185 \rightarrow 462, 1\}$ ,  
 $\{715 \rightarrow 714, 0\}$ ,  $\{715 \rightarrow 464, 1\}$ ,  $\{716 \rightarrow 57, 0\}$ ,  $\{716 \rightarrow 518, 1\}$ ,  $\{717 \rightarrow 616, 0\}$ ,  
 $\{717 \rightarrow 532, 1\}$ ,  $\{718 \rightarrow 57, 0\}$ ,  $\{718 \rightarrow 527, 1\}$ ,  $\{719 \rightarrow 616, 0\}$ ,  $\{719 \rightarrow 542, 1\}$ ,  
 $\{720 \rightarrow 721, 0\}$ ,  $\{720 \rightarrow 539, 1\}$ ,  $\{722 \rightarrow 101, 0\}$ ,  $\{722 \rightarrow 521, 1\}$ ,  $\{723 \rightarrow 721, 0\}$ ,  
 $\{723 \rightarrow 533, 1\}$ ,  $\{724 \rightarrow 101, 0\}$ ,  $\{724 \rightarrow 528, 1\}$ ,  $\{725 \rightarrow 596, 0\}$ ,  $\{725 \rightarrow 357, 1\}$ ,  
 $\{726 \rightarrow 636, 0\}$ ,  $\{726 \rightarrow 360, 1\}$ ,  $\{727 \rightarrow 643, 0\}$ ,  $\{727 \rightarrow 357, 1\}$ ,  $\{710 \rightarrow 598, 0\}$ ,  
 $\{710 \rightarrow 345, 1\}$ ,  $\{229 \rightarrow 598, 0\}$ ,  $\{229 \rightarrow 405, 1\}$ ,  $\{150 \rightarrow 640, 0\}$ ,  $\{150 \rightarrow 409, 1\}$ ,  
 $\{728 \rightarrow 596, 0\}$ ,  $\{728 \rightarrow 391, 1\}$ ,  $\{221 \rightarrow 646, 0\}$ ,  $\{221 \rightarrow 405, 1\}$ ,  $\{237 \rightarrow 664, 0\}$ ,  
 $\{237 \rightarrow 409, 1\}$ ,  $\{729 \rightarrow 665, 0\}$ ,  $\{729 \rightarrow 360, 1\}$ ,  $\{148 \rightarrow 730, 0\}$ ,  $\{148 \rightarrow 362, 1\}$ ,  
 $\{731 \rightarrow 732, 0\}$ ,  $\{731 \rightarrow 400, 1\}$ ,  $\{733 \rightarrow 734, 0\}$ ,  $\{733 \rightarrow 400, 1\}$ ,  $\{217 \rightarrow 735, 0\}$ ,  
 $\{217 \rightarrow 375, 1\}$ ,  $\{224 \rightarrow 736, 0\}$ ,  $\{224 \rightarrow 375, 1\}$ ,  $\{712 \rightarrow 736, 0\}$ ,  $\{712 \rightarrow 389, 1\}$ ,  
 $\{737 \rightarrow 734, 0\}$ ,  $\{737 \rightarrow 355, 1\}$ ,  $\{738 \rightarrow 739, 0\}$ ,  $\{738 \rightarrow 93, 1\}$ ,  $\{239 \rightarrow 740, 0\}$ ,  
 $\{239 \rightarrow 362, 1\}$ ,  $\{741 \rightarrow 742, 0\}$ ,  $\{741 \rightarrow 93, 1\}$ ,  $\{227 \rightarrow 743, 0\}$ ,  $\{227 \rightarrow 93, 1\}$ ,  
 $\{702 \rightarrow 744, 0\}$ ,  $\{702 \rightarrow 362, 1\}$ ,  $\{705 \rightarrow 744, 0\}$ ,  $\{705 \rightarrow 382, 1\}$ ,  $\{214 \rightarrow 745, 0\}$ ,  
 $\{214 \rightarrow 93, 1\}$ ,  $\{714 \rightarrow 743, 0\}$ ,  $\{714 \rightarrow 348, 1\}$ ,  $\{155 \rightarrow 746, 0\}$ ,  $\{155 \rightarrow 400, 1\}$ ,  
 $\{234 \rightarrow 747, 0\}$ ,  $\{234 \rightarrow 400, 1\}$ ,  $\{748 \rightarrow 749, 0\}$ ,  $\{748 \rightarrow 362, 1\}$ ,  $\{750 \rightarrow 751, 0\}$ ,  
 $\{750 \rightarrow 375, 1\}$ ,  $\{752 \rightarrow 753, 0\}$ ,  $\{752 \rightarrow 375, 1\}$ ,  $\{754 \rightarrow 599, 0\}$ ,  $\{754 \rightarrow 182, 1\}$ ,  
 $\{755 \rightarrow 599, 0\}$ ,  $\{755 \rightarrow 200, 1\}$ ,  $\{746 \rightarrow 601, 0\}$ ,  $\{746 \rightarrow 167, 1\}$ ,  $\{753 \rightarrow 601, 0\}$ ,  
 $\{753 \rightarrow 144, 1\}$ ,  $\{756 \rightarrow 717, 0\}$ ,  $\{756 \rightarrow 405, 1\}$ ,  $\{708 \rightarrow 667, 0\}$ ,  $\{708 \rightarrow 384, 1\}$ ,  
 $\{757 \rightarrow 671, 0\}$ ,  $\{757 \rightarrow 409, 1\}$ ,  $\{758 \rightarrow 671, 0\}$ ,  $\{758 \rightarrow 351, 1\}$ ,  $\{153 \rightarrow 722, 0\}$ ,  
 $\{153 \rightarrow 357, 1\}$ ,  $\{759 \rightarrow 704, 0\}$ ,  $\{759 \rightarrow 409, 1\}$ ,  $\{219 \rightarrow 706, 0\}$ ,  $\{219 \rightarrow 360, 1\}$ ,  
 $\{231 \rightarrow 667, 0\}$ ,  $\{231 \rightarrow 360, 1\}$ ,  $\{760 \rightarrow 724, 0\}$ ,  $\{760 \rightarrow 405, 1\}$ ,  $\{241 \rightarrow 719, 0\}$ ,  
 $\{241 \rightarrow 357, 1\}$ ,  $\{743 \rightarrow 761, 0\}$ ,  $\{743 \rightarrow 116, 1\}$ ,  $\{761 \rightarrow 762, 0\}$ ,  $\{761 \rightarrow 180, 1\}$ ,  
 $\{744 \rightarrow 761, 0\}$ ,  $\{744 \rightarrow 130, 1\}$ ,  $\{762 \rightarrow 762, 0\}$ ,  $\{762 \rightarrow 202, 1\}$ ,  $\{745 \rightarrow 672, 0\}$ ,  
 $\{745 \rightarrow 206, 1\}$ ,  $\{763 \rightarrow 669, 0\}$ ,  $\{763 \rightarrow 124, 1\}$ ,  $\{749 \rightarrow 672, 0\}$ ,  $\{749 \rightarrow 186, 1\}$ ,  
 $\{764 \rightarrow 669, 0\}$ ,  $\{764 \rightarrow 172, 1\}$ ,  $\{765 \rightarrow 766, 0\}$ ,  $\{765 \rightarrow 135, 1\}$ ,  $\{747 \rightarrow 767, 0\}$ ,  
 $\{747 \rightarrow 208, 1\}$ ,  $\{751 \rightarrow 767, 0\}$ ,  $\{751 \rightarrow 188, 1\}$ ,  $\{768 \rightarrow 766, 0\}$ ,  $\{768 \rightarrow 174, 1\}$ ,  
 $\{30 \rightarrow 769, 0\}$ ,  $\{30 \rightarrow 282, 1\}$ ,  $\{770 \rightarrow 771, 0\}$ ,  $\{770 \rightarrow 303, 1\}$ ,  $\{99 \rightarrow 772, 0\}$ ,  
 $\{99 \rightarrow 290, 1\}$ ,  $\{773 \rightarrow 774, 0\}$ ,  $\{773 \rightarrow 305, 1\}$ ,  $\{688 \rightarrow 775, 0\}$ ,  $\{688 \rightarrow 305, 1\}$ ,  
 $\{689 \rightarrow 775, 0\}$ ,  $\{689 \rightarrow 279, 1\}$ ,  $\{776 \rightarrow 772, 0\}$ ,  $\{776 \rightarrow 262, 1\}$ ,  $\{119 \rightarrow 777, 0\}$ ,  
 $\{119 \rightarrow 282, 1\}$ ,  $\{778 \rightarrow 779, 0\}$ ,  $\{778 \rightarrow 303, 1\}$ ,  $\{111 \rightarrow 780, 0\}$ ,  $\{111 \rightarrow 290, 1\}$ ,

$\{730 \rightarrow 781, 0\}$ ,  $\{730 \rightarrow 69, 1\}$ ,  $\{782 \rightarrow 783, 0\}$ ,  $\{782 \rightarrow 54, 1\}$ ,  $\{784 \rightarrow 783, 0\}$ ,  
 $\{784 \rightarrow 17, 1\}$ ,  $\{739 \rightarrow 781, 0\}$ ,  $\{739 \rightarrow 90, 1\}$ ,  $\{682 \rightarrow 785, 0\}$ ,  $\{682 \rightarrow 251, 1\}$ ,  
 $\{33 \rightarrow 786, 0\}$ ,  $\{33 \rightarrow 305, 1\}$ ,  $\{694 \rightarrow 785, 0\}$ ,  $\{694 \rightarrow 282, 1\}$ ,  $\{787 \rightarrow 788, 0\}$ ,  
 $\{787 \rightarrow 290, 1\}$ ,  $\{96 \rightarrow 789, 0\}$ ,  $\{96 \rightarrow 303, 1\}$ ,  $\{790 \rightarrow 789, 0\}$ ,  $\{790 \rightarrow 275, 1\}$ ,  
 $\{791 \rightarrow 792, 0\}$ ,  $\{791 \rightarrow 282, 1\}$ ,  $\{793 \rightarrow 794, 0\}$ ,  $\{793 \rightarrow 290, 1\}$ ,  $\{121 \rightarrow 795, 0\}$ ,  
 $\{121 \rightarrow 305, 1\}$ ,  $\{109 \rightarrow 796, 0\}$ ,  $\{109 \rightarrow 303, 1\}$ ,  $\{732 \rightarrow 797, 0\}$ ,  $\{732 \rightarrow 41, 1\}$ ,  
 $\{798 \rightarrow 799, 0\}$ ,  $\{798 \rightarrow 80, 1\}$ ,  $\{735 \rightarrow 797, 0\}$ ,  $\{735 \rightarrow 22, 1\}$ ,  $\{800 \rightarrow 799, 0\}$ ,  
 $\{800 \rightarrow 73, 1\}$ ,  $\{684 \rightarrow 801, 0\}$ ,  $\{684 \rightarrow 91, 1\}$ ,  $\{94 \rightarrow 802, 0\}$ ,  $\{94 \rightarrow 85, 1\}$ ,  
 $\{35 \rightarrow 803, 0\}$ ,  $\{35 \rightarrow 289, 1\}$ ,  $\{104 \rightarrow 804, 0\}$ ,  $\{104 \rightarrow 85, 1\}$ ,  $\{805 \rightarrow 802, 0\}$ ,  
 $\{805 \rightarrow 76, 1\}$ ,  $\{806 \rightarrow 807, 0\}$ ,  $\{806 \rightarrow 309, 1\}$ ,  $\{117 \rightarrow 808, 0\}$ ,  $\{117 \rightarrow 289, 1\}$ ,  
 $\{809 \rightarrow 810, 0\}$ ,  $\{809 \rightarrow 91, 1\}$ ,  $\{695 \rightarrow 801, 0\}$ ,  $\{695 \rightarrow 81, 1\}$ ,  $\{811 \rightarrow 812, 0\}$ ,  
 $\{811 \rightarrow 309, 1\}$ ,  $\{767 \rightarrow 813, 0\}$ ,  $\{767 \rightarrow 47, 1\}$ ,  $\{736 \rightarrow 814, 0\}$ ,  $\{736 \rightarrow 71, 1\}$ ,  
 $\{734 \rightarrow 814, 0\}$ ,  $\{734 \rightarrow 84, 1\}$ ,  $\{766 \rightarrow 813, 0\}$ ,  $\{766 \rightarrow 24, 1\}$ ,  $\{37 \rightarrow 815, 0\}$ ,  
 $\{37 \rightarrow 91, 1\}$ ,  $\{721 \rightarrow 816, 0\}$ ,  $\{721 \rightarrow 271, 1\}$ ,  $\{101 \rightarrow 816, 0\}$ ,  $\{101 \rightarrow 309, 1\}$ ,  
 $\{686 \rightarrow 817, 0\}$ ,  $\{686 \rightarrow 289, 1\}$ ,  $\{692 \rightarrow 817, 0\}$ ,  $\{692 \rightarrow 260, 1\}$ ,  $\{818 \rightarrow 819, 0\}$ ,  
 $\{818 \rightarrow 85, 1\}$ ,  $\{107 \rightarrow 820, 0\}$ ,  $\{107 \rightarrow 309, 1\}$ ,  $\{114 \rightarrow 821, 0\}$ ,  $\{114 \rightarrow 91, 1\}$ ,  
 $\{822 \rightarrow 823, 0\}$ ,  $\{822 \rightarrow 289, 1\}$ ,  $\{824 \rightarrow 825, 0\}$ ,  $\{824 \rightarrow 85, 1\}$ ,  $\{826 \rightarrow 827, 0\}$ ,  
 $\{826 \rightarrow 67, 1\}$ ,  $\{828 \rightarrow 827, 0\}$ ,  $\{828 \rightarrow 62, 1\}$ ,  $\{740 \rightarrow 829, 0\}$ ,  $\{740 \rightarrow 4, 1\}$ ,  
 $\{742 \rightarrow 829, 0\}$ ,  $\{742 \rightarrow 50, 1\}$ ,  $\{595 \rightarrow 830, 0\}$ ,  $\{595 \rightarrow 725, 1\}$ ,  $\{831 \rightarrow 651, 0\}$ ,  
 $\{831 \rightarrow 726, 1\}$ ,  $\{832 \rightarrow 651, 0\}$ ,  $\{832 \rightarrow 738, 1\}$ ,  $\{819 \rightarrow 652, 0\}$ ,  $\{819 \rightarrow 752, 1\}$ ,  
 $\{821 \rightarrow 652, 0\}$ ,  $\{821 \rightarrow 760, 1\}$ ,  $\{813 \rightarrow 603, 0\}$ ,  $\{813 \rightarrow 731, 1\}$ ,  $\{814 \rightarrow 603, 0\}$ ,  
 $\{814 \rightarrow 727, 1\}$ ,  $\{816 \rightarrow 438, 0\}$ ,  $\{816 \rightarrow 759, 1\}$ ,  $\{817 \rightarrow 438, 0\}$ ,  $\{817 \rightarrow 748, 1\}$ ,  
 $\{603 \rightarrow 642, 0\}$ ,  $\{603 \rightarrow 696, 1\}$ ,  $\{642 \rightarrow 644, 0\}$ ,  $\{642 \rightarrow 676, 1\}$ ,  $\{414 \rightarrow 833, 0\}$ ,  
 $\{414 \rightarrow 707, 1\}$ ,  $\{644 \rightarrow 644, 0\}$ ,  $\{644 \rightarrow 687, 1\}$ ,  $\{834 \rightarrow 835, 0\}$ ,  $\{834 \rightarrow 690, 1\}$ ,  
 $\{438 \rightarrow 642, 0\}$ ,  $\{438 \rightarrow 707, 1\}$ ,  $\{425 \rightarrow 836, 0\}$ ,  $\{425 \rightarrow 713, 1\}$ ,  $\{434 \rightarrow 837, 0\}$ ,  
 $\{434 \rightarrow 713, 1\}$ ,  $\{838 \rightarrow 839, 0\}$ ,  $\{838 \rightarrow 690, 1\}$ ,  $\{840 \rightarrow 841, 0\}$ ,  $\{840 \rightarrow 687, 1\}$ ,  
 $\{842 \rightarrow 662, 0\}$ ,  $\{842 \rightarrow 14, 1\}$ ,  $\{441 \rightarrow 600, 0\}$ ,  $\{441 \rightarrow 683, 1\}$ ,  $\{843 \rightarrow 844, 0\}$ ,  
 $\{843 \rightarrow 709, 1\}$ ,  $\{845 \rightarrow 846, 0\}$ ,  $\{845 \rightarrow 709, 1\}$ ,  $\{833 \rightarrow 597, 0\}$ ,  $\{833 \rightarrow 699, 1\}$ ,  
 $\{841 \rightarrow 597, 0\}$ ,  $\{841 \rightarrow 711, 1\}$ ,  $\{607 \rightarrow 600, 0\}$ ,  $\{607 \rightarrow 678, 1\}$ ,  $\{847 \rightarrow 848, 0\}$ ,  
 $\{847 \rightarrow 711, 1\}$ ,  $\{433 \rightarrow 849, 0\}$ ,  $\{433 \rightarrow 693, 1\}$ ,  $\{415 \rightarrow 850, 0\}$ ,  $\{415 \rightarrow 683, 1\}$ ,  
 $\{428 \rightarrow 851, 0\}$ ,  $\{428 \rightarrow 693, 1\}$ ,  $\{852 \rightarrow 853, 0\}$ ,  $\{852 \rightarrow 707, 1\}$ ,  $\{854 \rightarrow 855, 0\}$ ,  
 $\{854 \rightarrow 707, 1\}$ ,  $\{422 \rightarrow 326, 0\}$ ,  $\{422 \rightarrow 687, 1\}$ ,  $\{440 \rightarrow 328, 0\}$ ,  $\{440 \rightarrow 690, 1\}$ ,  
 $\{835 \rightarrow 637, 0\}$ ,  $\{835 \rightarrow 713, 1\}$ ,  $\{609 \rightarrow 328, 0\}$ ,  $\{609 \rightarrow 679, 1\}$ ,  $\{836 \rightarrow 637, 0\}$ ,  
 $\{836 \rightarrow 668, 1\}$ ,  $\{436 \rightarrow 330, 0\}$ ,  $\{436 \rightarrow 687, 1\}$ ,  $\{856 \rightarrow 857, 0\}$ ,  $\{856 \rightarrow 713, 1\}$ ,  
 $\{420 \rightarrow 331, 0\}$ ,  $\{420 \rightarrow 690, 1\}$ ,  $\{858 \rightarrow 374, 0\}$ ,  $\{858 \rightarrow 756, 1\}$ ,  $\{859 \rightarrow 374, 0\}$ ,  
 $\{859 \rightarrow 750, 1\}$ ,  $\{820 \rightarrow 617, 0\}$ ,  $\{820 \rightarrow 729, 1\}$ ,  $\{823 \rightarrow 617, 0\}$ ,  $\{823 \rightarrow 741, 1\}$ ,  
 $\{860 \rightarrow 642, 0\}$ ,  $\{860 \rightarrow 43, 1\}$ ,  $\{442 \rightarrow 662, 0\}$ ,  $\{442 \rightarrow 709, 1\}$ ,  $\{431 \rightarrow 861, 0\}$ ,  
 $\{431 \rightarrow 711, 1\}$ ,  $\{862 \rightarrow 274, 0\}$ ,  $\{862 \rightarrow 683, 1\}$ ,  $\{863 \rightarrow 250, 0\}$ ,  $\{863 \rightarrow 693, 1\}$ ,  
 $\{426 \rightarrow 864, 0\}$ ,  $\{426 \rightarrow 711, 1\}$ ,  $\{839 \rightarrow 281, 0\}$ ,  $\{839 \rightarrow 693, 1\}$ ,  $\{837 \rightarrow 281, 0\}$ ,  
 $\{837 \rightarrow 681, 1\}$ ,  $\{418 \rightarrow 865, 0\}$ ,  $\{418 \rightarrow 709, 1\}$ ,  $\{866 \rightarrow 253, 0\}$ ,  $\{866 \rightarrow 683, 1\}$ ,  
 $\{611 \rightarrow 662, 0\}$ ,  $\{611 \rightarrow 700, 1\}$ ,  $\{867 \rightarrow 631, 0\}$ ,  $\{867 \rightarrow 757, 1\}$ ,  $\{815 \rightarrow 623, 0\}$ ,  
 $\{815 \rightarrow 725, 1\}$ ,  $\{868 \rightarrow 631, 0\}$ ,  $\{868 \rightarrow 702, 1\}$ ,  $\{825 \rightarrow 623, 0\}$ ,  $\{825 \rightarrow 733, 1\}$ ,  
 $\{869 \rightarrow 600, 0\}$ ,  $\{869 \rightarrow 19, 1\}$ ,  $\{830 \rightarrow 675, 0\}$ ,  $\{830 \rightarrow 403, 1\}$ ,  $\{783 \rightarrow 667, 0\}$ ,  
 $\{783 \rightarrow 870, 1\}$ ,  $\{789 \rightarrow 671, 0\}$ ,  $\{789 \rightarrow 871, 1\}$ ,  $\{785 \rightarrow 671, 0\}$ ,  $\{785 \rightarrow 872, 1\}$ ,  
 $\{781 \rightarrow 667, 0\}$ ,  $\{781 \rightarrow 873, 1\}$ ,  $\{651 \rightarrow 669, 0\}$ ,  $\{651 \rightarrow 874, 1\}$ ,  $\{247 \rightarrow 701, 0\}$ ,  
 $\{247 \rightarrow 875, 1\}$ ,  $\{662 \rightarrow 672, 0\}$ ,  $\{662 \rightarrow 876, 1\}$ ,  $\{877 \rightarrow 716, 0\}$ ,  $\{877 \rightarrow 877, 1\}$ ,  
 $\{878 \rightarrow 703, 0\}$ ,  $\{878 \rightarrow 879, 1\}$ ,  $\{879 \rightarrow 720, 0\}$ ,  $\{879 \rightarrow 877, 1\}$ ,  $\{652 \rightarrow 669, 0\}$ ,

{652 → 879, 1}, {308 → 723, 0}, {308 → 880, 1}, {293 → 718, 0}, {293 → 880, 1},  
 {281 → 672, 0}, {281 → 875, 1}, {253 → 767, 0}, {253 → 881, 1}, {254 → 798, 0},  
 {254 → 881, 1}, {285 → 782, 0}, {285 → 647, 1}, {287 → 826, 0}, {287 → 647, 1},  
 {876 → 784, 0}, {876 → 652, 1}, {882 → 828, 0}, {882 → 652, 1}, {861 → 767, 0},  
 {861 → 883, 1}, {655 → 766, 0}, {655 → 884, 1}, {656 → 766, 0}, {656 → 878, 1},  
 {883 → 800, 0}, {883 → 878, 1}, {245 → 641, 0}, {245 → 877, 1}, {881 → 645, 0},  
 {881 → 880, 1}, {875 → 638, 0}, {875 → 875, 1}, {647 → 599, 0}, {647 → 880, 1},  
 {302 → 639, 0}, {302 → 879, 1}, {880 → 661, 0}, {880 → 875, 1}, {649 → 599, 0},  
 {649 → 882, 1}, {274 → 601, 0}, {274 → 877, 1}, {292 → 663, 0}, {292 → 879, 1},  
 {864 → 601, 0}, {864 → 885, 1}, {283 → 754, 0}, {283 → 878, 1}, {874 → 755, 0},  
 {874 → 881, 1}, {250 → 761, 0}, {250 → 652, 1}, {288 → 765, 0}, {288 → 878, 1},  
 {257 → 763, 0}, {257 → 652, 1}, {653 → 762, 0}, {653 → 647, 1}, {658 → 762, 0},  
 {658 → 656, 1}, {884 → 764, 0}, {884 → 647, 1}, {885 → 768, 0}, {885 → 881, 1},  
 {865 → 761, 0}, {865 → 653, 1}, {886 → 598, 0}, {886 → 887, 1}, {888 → 598, 0},  
 {888 → 889, 1}, {786 → 596, 0}, {786 → 890, 1}, {788 → 596, 0}, {788 → 891, 1},  
 {892 → 743, 0}, {892 → 627, 1}, {792 → 744, 0}, {792 → 633, 1}, {893 → 743, 0},  
 {893 → 631, 1}, {796 → 744, 0}, {796 → 629, 1}, {894 → 736, 0}, {894 → 895, 1},  
 {896 → 736, 0}, {896 → 897, 1}, {794 → 734, 0}, {794 → 898, 1}, {795 → 734, 0},  
 {795 → 899, 1}, {403 → 813, 0}, {403 → 900, 1}, {243 → 831, 0}, {243 → 850, 1},  
 {850 → 814, 0}, {850 → 901, 1}, {902 → 842, 0}, {902 → 903, 1}, {901 → 858, 0},  
 {901 → 901, 1}, {903 → 860, 0}, {903 → 904, 1}, {905 → 867, 0}, {905 → 850, 1},  
 {904 → 869, 0}, {904 → 904, 1}, {371 → 859, 0}, {371 → 900, 1}, {344 → 832, 0},  
 {344 → 849, 1}, {848 → 814, 0}, {848 → 906, 1}, {620 → 813, 0}, {620 → 907, 1},  
 {396 → 868, 0}, {396 → 849, 1}, {334 → 908, 0}, {334 → 902, 1}, {337 → 909, 0},  
 {337 → 243, 1}, {597 → 797, 0}, {597 → 910, 1}, {600 → 797, 0}, {600 → 911, 1},  
 {374 → 799, 0}, {374 → 905, 1}, {369 → 912, 0}, {369 → 905, 1}, {617 → 799, 0},  
 {617 → 913, 1}, {914 → 915, 0}, {914 → 916, 1}, {342 → 917, 0}, {342 → 243, 1},  
 {913 → 918, 0}, {913 → 916, 1}, {906 → 919, 0}, {906 → 911, 1}, {900 → 920, 0},  
 {900 → 849, 1}, {849 → 829, 0}, {849 → 849, 1}, {916 → 921, 0}, {916 → 900, 1},  
 {911 → 922, 0}, {911 → 900, 1}, {844 → 829, 0}, {844 → 851, 1}, {366 → 923, 0},  
 {366 → 850, 1}, {404 → 827, 0}, {404 → 850, 1}, {386 → 924, 0}, {386 → 901, 1},  
 {354 → 925, 0}, {354 → 901, 1}, {621 → 827, 0}, {621 → 600, 1}, {359 → 783, 0},  
 {359 → 916, 1}, {910 → 886, 0}, {910 → 905, 1}, {347 → 888, 0}, {347 → 911, 1},  
 {612 → 783, 0}, {612 → 926, 1}, {364 → 892, 0}, {364 → 916, 1}, {926 → 894, 0},  
 {926 → 905, 1}, {350 → 896, 0}, {350 → 911, 1}, {851 → 781, 0}, {851 → 243, 1},  
 {846 → 781, 0}, {846 → 914, 1}, {907 → 893, 0}, {907 → 243, 1}, {908 → 827, 0},  
 {908 → 253, 1}, {769 → 789, 0}, {769 → 852, 1}, {909 → 785, 0}, {909 → 843, 1},  
 {918 → 785, 0}, {918 → 838, 1}, {779 → 789, 0}, {779 → 866, 1}, {797 → 775, 0},  
 {797 → 854, 1}, {775 → 772, 0}, {775 → 845, 1}, {772 → 772, 0}, {772 → 834, 1},  
 {799 → 775, 0}, {799 → 862, 1}, {771 → 802, 0}, {771 → 841, 1}, {915 → 801, 0},  
 {915 → 835, 1}, {917 → 801, 0}, {917 → 839, 1}, {777 → 802, 0}, {777 → 644, 1},  
 {774 → 816, 0}, {774 → 863, 1}, {912 → 817, 0}, {912 → 847, 1}, {919 → 817, 0},  
 {919 → 840, 1}, {780 → 816, 0}, {780 → 856, 1}, {920 → 697, 0}, {920 → 770, 1},  
 {923 → 697, 0}, {923 → 818, 1}, {804 → 139, 0}, {804 → 793, 1}, {810 → 139, 0},  
 {810 → 811, 1}, {827 → 227, 0}, {827 → 684, 1}, {829 → 227, 0}, {829 → 694, 1},  
 {801 → 714, 0}, {801 → 686, 1}, {802 → 714, 0}, {802 → 688, 1}, {870 → 49, 0},  
 {870 → 613, 1}, {297 → 604, 0}, {297 → 648, 1}, {853 → 616, 0}, {853 → 628, 1},

$\{624 \rightarrow 57, 0\}, \{624 \rightarrow 608, 1\}, \{313 \rightarrow 634, 0\}, \{313 \rightarrow 654, 1\}, \{897 \rightarrow 53, 0\},$   
 $\{897 \rightarrow 619, 1\}, \{891 \rightarrow 46, 0\}, \{891 \rightarrow 613, 1\}, \{633 \rightarrow 57, 0\}, \{633 \rightarrow 619, 1\},$   
 $\{330 \rightarrow 616, 0\}, \{330 \rightarrow 648, 1\}, \{321 \rightarrow 660, 0\}, \{321 \rightarrow 654, 1\}, \{921 \rightarrow 614, 0\},$   
 $\{921 \rightarrow 787, 1\}, \{925 \rightarrow 614, 0\}, \{925 \rightarrow 806, 1\}, \{808 \rightarrow 618, 0\}, \{808 \rightarrow 778, 1\},$   
 $\{812 \rightarrow 618, 0\}, \{812 \rightarrow 824, 1\}, \{298 \rightarrow 99, 0\}, \{298 \rightarrow 615, 1\}, \{622 \rightarrow 721, 0\},$   
 $\{622 \rightarrow 626, 1\}, \{855 \rightarrow 101, 0\}, \{855 \rightarrow 606, 1\}, \{873 \rightarrow 790, 0\}, \{873 \rightarrow 650, 1\},$   
 $\{312 \rightarrow 96, 0\}, \{312 \rightarrow 614, 1\}, \{326 \rightarrow 101, 0\}, \{326 \rightarrow 615, 1\}, \{895 \rightarrow 776, 0\},$   
 $\{895 \rightarrow 657, 1\}, \{629 \rightarrow 721, 0\}, \{629 \rightarrow 657, 1\}, \{890 \rightarrow 805, 0\}, \{890 \rightarrow 650, 1\},$   
 $\{323 \rightarrow 94, 0\}, \{323 \rightarrow 614, 1\}, \{871 \rightarrow 725, 0\}, \{871 \rightarrow 615, 1\}, \{887 \rightarrow 733, 0\},$   
 $\{887 \rightarrow 615, 1\}, \{637 \rightarrow 705, 0\}, \{637 \rightarrow 630, 1\}, \{623 \rightarrow 702, 0\}, \{623 \rightarrow 602, 1\},$   
 $\{300 \rightarrow 758, 0\}, \{300 \rightarrow 650, 1\}, \{631 \rightarrow 702, 0\}, \{631 \rightarrow 614, 1\}, \{328 \rightarrow 705, 0\},$   
 $\{328 \rightarrow 650, 1\}, \{315 \rightarrow 728, 0\}, \{315 \rightarrow 657, 1\}, \{318 \rightarrow 737, 0\}, \{318 \rightarrow 657, 1\},$   
 $\{899 \rightarrow 757, 0\}, \{899 \rightarrow 614, 1\}, \{872 \rightarrow 685, 0\}, \{872 \rightarrow 648, 1\}, \{889 \rightarrow 677, 0\},$   
 $\{889 \rightarrow 648, 1\}, \{627 \rightarrow 670, 0\}, \{627 \rightarrow 654, 1\}, \{625 \rightarrow 670, 0\}, \{625 \rightarrow 632, 1\},$   
 $\{301 \rightarrow 713, 0\}, \{301 \rightarrow 613, 1\}, \{319 \rightarrow 679, 0\}, \{319 \rightarrow 619, 1\}, \{331 \rightarrow 668, 0\},$   
 $\{331 \rightarrow 613, 1\}, \{898 \rightarrow 715, 0\}, \{898 \rightarrow 654, 1\}, \{317 \rightarrow 690, 0\}, \{317 \rightarrow 619, 1\},$   
 $\{857 \rightarrow 668, 0\}, \{857 \rightarrow 610, 1\}, \{922 \rightarrow 692, 0\}, \{922 \rightarrow 773, 1\}, \{803 \rightarrow 686, 0\},$   
 $\{803 \rightarrow 791, 1\}, \{924 \rightarrow 692, 0\}, \{924 \rightarrow 822, 1\}, \{807 \rightarrow 686, 0\}, \{807 \rightarrow 809, 1\}\},$   
1,  $\{1 \rightarrow 0, 2 \rightarrow 0, 3 \rightarrow 1, 4 \rightarrow 0, 5 \rightarrow 0, 6 \rightarrow 1, 7 \rightarrow 0, 8 \rightarrow 0, 9 \rightarrow 1, 10 \rightarrow 0, 11 \rightarrow 0,$   
 $12 \rightarrow 0, 13 \rightarrow 0, 14 \rightarrow 1, 15 \rightarrow 0, 16 \rightarrow 1, 17 \rightarrow 0, 18 \rightarrow 0, 19 \rightarrow 1, 20 \rightarrow 0, 21 \rightarrow 0,$   
 $22 \rightarrow 0, 23 \rightarrow 0, 24 \rightarrow 0, 25 \rightarrow 0, 26 \rightarrow 0, 27 \rightarrow 1, 28 \rightarrow 0, 29 \rightarrow 0, 30 \rightarrow 1, 31 \rightarrow 0,$   
 $32 \rightarrow 0, 33 \rightarrow 1, 34 \rightarrow 0, 35 \rightarrow 1, 36 \rightarrow 0, 37 \rightarrow 1, 38 \rightarrow 0, 39 \rightarrow 0, 40 \rightarrow 1, 41 \rightarrow 0,$   
 $42 \rightarrow 0, 43 \rightarrow 1, 44 \rightarrow 0, 45 \rightarrow 0, 46 \rightarrow 1, 47 \rightarrow 0, 48 \rightarrow 0, 49 \rightarrow 1, 50 \rightarrow 0, 51 \rightarrow 0,$   
 $52 \rightarrow 0, 53 \rightarrow 1, 54 \rightarrow 0, 55 \rightarrow 0, 56 \rightarrow 0, 57 \rightarrow 1, 58 \rightarrow 0, 59 \rightarrow 0, 60 \rightarrow 0, 61 \rightarrow 0,$   
 $62 \rightarrow 0, 63 \rightarrow 1, 64 \rightarrow 0, 65 \rightarrow 0, 66 \rightarrow 0, 67 \rightarrow 0, 68 \rightarrow 1, 69 \rightarrow 0, 70 \rightarrow 0, 71 \rightarrow 0,$   
 $72 \rightarrow 0, 73 \rightarrow 0, 74 \rightarrow 0, 75 \rightarrow 0, 76 \rightarrow 0, 77 \rightarrow 0, 78 \rightarrow 0, 79 \rightarrow 1, 80 \rightarrow 0, 81 \rightarrow 0,$   
 $82 \rightarrow 0, 83 \rightarrow 0, 84 \rightarrow 0, 85 \rightarrow 0, 86 \rightarrow 0, 87 \rightarrow 1, 88 \rightarrow 0, 89 \rightarrow 0, 90 \rightarrow 0, 91 \rightarrow 0,$   
 $92 \rightarrow 0, 93 \rightarrow 0, 94 \rightarrow 1, 95 \rightarrow 0, 96 \rightarrow 1, 97 \rightarrow 0, 98 \rightarrow 0, 99 \rightarrow 1, 100 \rightarrow 0, 101 \rightarrow 1,$   
 $102 \rightarrow 0, 103 \rightarrow 0, 104 \rightarrow 1, 105 \rightarrow 0, 106 \rightarrow 0, 107 \rightarrow 1, 108 \rightarrow 0, 109 \rightarrow 1, 110 \rightarrow 0,$   
 $111 \rightarrow 1, 112 \rightarrow 0, 113 \rightarrow 0, 114 \rightarrow 1, 115 \rightarrow 0, 116 \rightarrow 0, 117 \rightarrow 1, 118 \rightarrow 0, 119 \rightarrow 1,$   
 $120 \rightarrow 0, 121 \rightarrow 1, 122 \rightarrow 0, 123 \rightarrow 1, 124 \rightarrow 0, 125 \rightarrow 0, 126 \rightarrow 1, 127 \rightarrow 0, 128 \rightarrow 0,$   
 $129 \rightarrow 1, 130 \rightarrow 0, 131 \rightarrow 0, 132 \rightarrow 1, 133 \rightarrow 0, 134 \rightarrow 1, 135 \rightarrow 0, 136 \rightarrow 0, 137 \rightarrow 0,$   
 $138 \rightarrow 1, 139 \rightarrow 1, 140 \rightarrow 0, 141 \rightarrow 0, 142 \rightarrow 0, 143 \rightarrow 0, 144 \rightarrow 0, 145 \rightarrow 0, 146 \rightarrow 0,$   
 $147 \rightarrow 0, 148 \rightarrow 1, 149 \rightarrow 0, 150 \rightarrow 1, 151 \rightarrow 0, 152 \rightarrow 0, 153 \rightarrow 1, 154 \rightarrow 0, 155 \rightarrow 1,$   
 $156 \rightarrow 0, 157 \rightarrow 1, 158 \rightarrow 0, 159 \rightarrow 1, 160 \rightarrow 1, 161 \rightarrow 0, 162 \rightarrow 0, 163 \rightarrow 1, 164 \rightarrow 1,$   
 $165 \rightarrow 0, 166 \rightarrow 0, 167 \rightarrow 0, 168 \rightarrow 0, 169 \rightarrow 1, 170 \rightarrow 0, 171 \rightarrow 0, 172 \rightarrow 0, 173 \rightarrow 0,$   
 $174 \rightarrow 0, 175 \rightarrow 0, 176 \rightarrow 0, 177 \rightarrow 0, 178 \rightarrow 0, 179 \rightarrow 1, 180 \rightarrow 0, 181 \rightarrow 0, 182 \rightarrow 0,$   
 $183 \rightarrow 0, 184 \rightarrow 0, 185 \rightarrow 1, 186 \rightarrow 0, 187 \rightarrow 0, 188 \rightarrow 0, 189 \rightarrow 0, 190 \rightarrow 0, 191 \rightarrow 0,$   
 $192 \rightarrow 0, 193 \rightarrow 0, 194 \rightarrow 0, 195 \rightarrow 0, 196 \rightarrow 0, 197 \rightarrow 1, 198 \rightarrow 0, 199 \rightarrow 0, 200 \rightarrow 0,$   
 $201 \rightarrow 0, 202 \rightarrow 0, 203 \rightarrow 0, 204 \rightarrow 0, 205 \rightarrow 0, 206 \rightarrow 0, 207 \rightarrow 0, 208 \rightarrow 0, 209 \rightarrow 0,$   
 $210 \rightarrow 0, 211 \rightarrow 1, 212 \rightarrow 0, 213 \rightarrow 0, 214 \rightarrow 1, 215 \rightarrow 0, 216 \rightarrow 0, 217 \rightarrow 1, 218 \rightarrow 0,$   
 $219 \rightarrow 1, 220 \rightarrow 0, 221 \rightarrow 1, 222 \rightarrow 0, 223 \rightarrow 0, 224 \rightarrow 1, 225 \rightarrow 0, 226 \rightarrow 0, 227 \rightarrow 1,$   
 $228 \rightarrow 0, 229 \rightarrow 1, 230 \rightarrow 0, 231 \rightarrow 1, 232 \rightarrow 0, 233 \rightarrow 0, 234 \rightarrow 1, 235 \rightarrow 0, 236 \rightarrow 0,$   
 $237 \rightarrow 1, 238 \rightarrow 0, 239 \rightarrow 1, 240 \rightarrow 0, 241 \rightarrow 1, 242 \rightarrow 0, 243 \rightarrow 1, 244 \rightarrow 0, 245 \rightarrow 1,$   
 $246 \rightarrow 0, 247 \rightarrow 1, 248 \rightarrow 0, 249 \rightarrow 0, 250 \rightarrow 1, 251 \rightarrow 0, 252 \rightarrow 0, 253 \rightarrow 1, 254 \rightarrow 1,$   
 $255 \rightarrow 0, 256 \rightarrow 0, 257 \rightarrow 1, 258 \rightarrow 0, 259 \rightarrow 0, 260 \rightarrow 0, 261 \rightarrow 0, 262 \rightarrow 0, 263 \rightarrow 0,$   
 $264 \rightarrow 0, 265 \rightarrow 0, 266 \rightarrow 0, 267 \rightarrow 0, 268 \rightarrow 0, 269 \rightarrow 0, 270 \rightarrow 0, 271 \rightarrow 0, 272 \rightarrow 0,$

273 → 0, 274 → 1, 275 → 0, 276 → 0, 277 → 0, 278 → 0, 279 → 0, 280 → 0, 281 → 1, 282 → 0, 283 → 1, 284 → 0, 285 → 1, 286 → 0, 287 → 1, 288 → 1, 289 → 0, 290 → 0, 291 → 0, 292 → 1, 293 → 1, 294 → 0, 295 → 0, 296 → 0, 297 → 1, 298 → 1, 299 → 0, 300 → 1, 301 → 1, 302 → 1, 303 → 0, 304 → 0, 305 → 0, 306 → 0, 307 → 0, 308 → 1, 309 → 0, 310 → 0, 311 → 0, 312 → 1, 313 → 1, 314 → 0, 315 → 1, 316 → 0, 317 → 1, 318 → 1, 319 → 1, 320 → 0, 321 → 1, 322 → 0, 323 → 1, 324 → 0, 325 → 0, 326 → 1, 327 → 0, 328 → 1, 329 → 0, 330 → 1, 331 → 1, 332 → 0, 333 → 0, 334 → 1, 335 → 0, 336 → 0, 337 → 1, 338 → 0, 339 → 0, 340 → 0, 341 → 0, 342 → 1, 343 → 0, 344 → 1, 345 → 0, 346 → 0, 347 → 1, 348 → 0, 349 → 0, 350 → 1, 351 → 0, 352 → 0, 353 → 0, 354 → 1, 355 → 0, 356 → 0, 357 → 0, 358 → 0, 359 → 1, 360 → 0, 361 → 0, 362 → 0, 363 → 0, 364 → 1, 365 → 0, 366 → 1, 367 → 0, 368 → 0, 369 → 1, 370 → 0, 371 → 1, 372 → 0, 373 → 0, 374 → 1, 375 → 0, 376 → 0, 377 → 0, 378 → 0, 379 → 0, 380 → 0, 381 → 0, 382 → 0, 383 → 0, 384 → 0, 385 → 0, 386 → 1, 387 → 0, 388 → 0, 389 → 0, 390 → 0, 391 → 0, 392 → 0, 393 → 0, 394 → 0, 395 → 0, 396 → 1, 397 → 0, 398 → 0, 399 → 0, 400 → 0, 401 → 0, 402 → 0, 403 → 1, 404 → 1, 405 → 0, 406 → 0, 407 → 0, 408 → 0, 409 → 0, 410 → 0, 411 → 0, 412 → 0, 413 → 0, 414 → 1, 415 → 1, 416 → 0, 417 → 0, 418 → 1, 419 → 0, 420 → 1, 421 → 0, 422 → 1, 423 → 0, 424 → 0, 425 → 1, 426 → 1, 427 → 0, 428 → 1, 429 → 0, 430 → 0, 431 → 1, 432 → 0, 433 → 1, 434 → 1, 435 → 0, 436 → 1, 437 → 0, 438 → 1, 439 → 0, 440 → 1, 441 → 1, 442 → 1, 443 → 0, 444 → 0, 445 → 0, 446 → 0, 447 → 0, 448 → 0, 449 → 0, 450 → 0, 451 → 0, 452 → 0, 453 → 0, 454 → 0, 455 → 0, 456 → 0, 457 → 0, 458 → 0, 459 → 0, 460 → 0, 461 → 0, 462 → 0, 463 → 0, 464 → 0, 465 → 0, 466 → 0, 467 → 0, 468 → 0, 469 → 0, 470 → 0, 471 → 0, 472 → 0, 473 → 0, 474 → 0, 475 → 0, 476 → 0, 477 → 0, 478 → 0, 479 → 0, 480 → 0, 481 → 0, 482 → 0, 483 → 0, 484 → 0, 485 → 0, 486 → 0, 487 → 0, 488 → 0, 489 → 0, 490 → 0, 491 → 0, 492 → 0, 493 → 0, 494 → 0, 495 → 0, 496 → 0, 497 → 0, 498 → 0, 499 → 0, 500 → 0, 501 → 0, 502 → 0, 503 → 0, 504 → 0, 505 → 0, 506 → 0, 507 → 0, 508 → 0, 509 → 0, 510 → 0, 511 → 0, 512 → 0, 513 → 0, 514 → 0, 515 → 0, 516 → 0, 517 → 0, 518 → 0, 519 → 0, 520 → 0, 521 → 0, 522 → 0, 523 → 0, 524 → 0, 525 → 0, 526 → 0, 527 → 0, 528 → 0, 529 → 0, 530 → 0, 531 → 0, 532 → 0, 533 → 0, 534 → 0, 535 → 0, 536 → 0, 537 → 0, 538 → 0, 539 → 0, 540 → 0, 541 → 0, 542 → 0, 543 → 0, 544 → 0, 545 → 0, 546 → 0, 547 → 0, 548 → 0, 549 → 0, 550 → 0, 551 → 0, 552 → 0, 553 → 0, 554 → 0, 555 → 0, 556 → 0, 557 → 0, 558 → 0, 559 → 0, 560 → 0, 561 → 0, 562 → 0, 563 → 0, 564 → 0, 565 → 0, 566 → 0, 567 → 0, 568 → 0, 569 → 0, 570 → 0, 571 → 0, 572 → 0, 573 → 0, 574 → 0, 575 → 0, 576 → 0, 577 → 0, 578 → 0, 579 → 0, 580 → 0, 581 → 0, 582 → 0, 583 → 0, 584 → 0, 585 → 0, 586 → 0, 587 → 0, 588 → 0, 589 → 0, 590 → 0, 591 → 0, 592 → 0, 593 → 0, 594 → 0, 595 → 1, 596 → 1, 597 → 1, 598 → 1, 599 → 1, 600 → 1, 601 → 1, 602 → 1, 603 → 1, 604 → 1, 605 → 1, 606 → 1, 607 → 1, 608 → 1, 609 → 1, 610 → 1, 611 → 1, 612 → 1, 613 → 1, 614 → 1, 615 → 1, 616 → 1, 617 → 1, 618 → 1, 619 → 1, 620 → 1, 621 → 1, 622 → 1, 623 → 1, 624 → 1, 625 → 1, 626 → 1, 627 → 1, 628 → 1, 629 → 1, 630 → 1, 631 → 1, 632 → 1, 633 → 1, 634 → 1, 635 → 1, 636 → 1, 637 → 1, 638 → 1, 639 → 1, 640 → 1, 641 → 1, 642 → 1, 643 → 1, 644 → 1, 645 → 1, 646 → 1, 647 → 1, 648 → 1, 649 → 1, 650 → 1, 651 → 1, 652 → 1, 653 → 1, 654 → 1, 655 → 1, 656 → 1, 657 → 1, 658 → 1, 659 → 1, 660 → 1, 661 → 1, 662 → 1, 663 → 1, 664 → 1, 665 → 1, 666 → 1, 667 → 1, 668 → 1, 669 → 1, 670 → 1, 671 → 1, 672 → 1, 673 → 1, 674 → 1, 675 → 1, 676 → 1, 677 → 1, 678 → 1, 679 → 1, 680 → 1, 681 → 1, 682 → 1, 683 → 1, 684 → 1, 685 → 1, 686 → 1, 687 → 1, 688 → 1, 689 → 1, 690 → 1, 691 → 1, 692 → 1, 693 → 1, 694 → 1, 695 → 1

```

696 → 1, 697 → 1, 698 → 1, 699 → 1, 700 → 1, 701 → 1, 702 → 1, 703 → 1, 704 → 1,
705 → 1, 706 → 1, 707 → 1, 708 → 1, 709 → 1, 710 → 1, 711 → 1, 712 → 1, 713 → 1,
714 → 1, 715 → 1, 716 → 1, 717 → 1, 718 → 1, 719 → 1, 720 → 1, 721 → 1, 722 → 1,
723 → 1, 724 → 1, 725 → 1, 726 → 1, 727 → 1, 728 → 1, 729 → 1, 730 → 1, 731 → 1,
732 → 1, 733 → 1, 734 → 1, 735 → 1, 736 → 1, 737 → 1, 738 → 1, 739 → 1, 740 → 1,
741 → 1, 742 → 1, 743 → 1, 744 → 1, 745 → 1, 746 → 1, 747 → 1, 748 → 1, 749 → 1,
750 → 1, 751 → 1, 752 → 1, 753 → 1, 754 → 1, 755 → 1, 756 → 1, 757 → 1, 758 → 1,
759 → 1, 760 → 1, 761 → 1, 762 → 1, 763 → 1, 764 → 1, 765 → 1, 766 → 1, 767 → 1,
768 → 1, 769 → 1, 770 → 1, 771 → 1, 772 → 1, 773 → 1, 774 → 1, 775 → 1, 776 → 1,
777 → 1, 778 → 1, 779 → 1, 780 → 1, 781 → 1, 782 → 1, 783 → 1, 784 → 1, 785 → 1,
786 → 1, 787 → 1, 788 → 1, 789 → 1, 790 → 1, 791 → 1, 792 → 1, 793 → 1, 794 → 1,
795 → 1, 796 → 1, 797 → 1, 798 → 1, 799 → 1, 800 → 1, 801 → 1, 802 → 1, 803 → 1,
804 → 1, 805 → 1, 806 → 1, 807 → 1, 808 → 1, 809 → 1, 810 → 1, 811 → 1, 812 → 1,
813 → 1, 814 → 1, 815 → 1, 816 → 1, 817 → 1, 818 → 1, 819 → 1, 820 → 1, 821 → 1,
822 → 1, 823 → 1, 824 → 1, 825 → 1, 826 → 1, 827 → 1, 828 → 1, 829 → 1, 830 → 1,
831 → 1, 832 → 1, 833 → 1, 834 → 1, 835 → 1, 836 → 1, 837 → 1, 838 → 1, 839 → 1,
840 → 1, 841 → 1, 842 → 1, 843 → 1, 844 → 1, 845 → 1, 846 → 1, 847 → 1, 848 → 1,
849 → 1, 850 → 1, 851 → 1, 852 → 1, 853 → 1, 854 → 1, 855 → 1, 856 → 1, 857 → 1,
858 → 1, 859 → 1, 860 → 1, 861 → 1, 862 → 1, 863 → 1, 864 → 1, 865 → 1, 866 → 1,
867 → 1, 868 → 1, 869 → 1, 870 → 1, 871 → 1, 872 → 1, 873 → 1, 874 → 1, 875 → 1,
876 → 1, 877 → 1, 878 → 1, 879 → 1, 880 → 1, 881 → 1, 882 → 1, 883 → 1, 884 → 1,
885 → 1, 886 → 1, 887 → 1, 888 → 1, 889 → 1, 890 → 1, 891 → 1, 892 → 1, 893 → 1,
894 → 1, 895 → 1, 896 → 1, 897 → 1, 898 → 1, 899 → 1, 900 → 1, 901 → 1, 902 → 1,
903 → 1, 904 → 1, 905 → 1, 906 → 1, 907 → 1, 908 → 1, 909 → 1, 910 → 1, 911 → 1,
912 → 1, 913 → 1, 914 → 1, 915 → 1, 916 → 1, 917 → 1, 918 → 1, 919 → 1, 920 → 1,
921 → 1, 922 → 1, 923 → 1, 924 → 1, 925 → 1, 926 → 1}, InputAlphabet → {0, 1}]

```

```

edge[x_, ___] := {Arrowheads[0.015], Arrow[x, 0.1]}

```

```

AutomatonGraph[automatonsigma82, VertexSize → 0.3, EdgeShapeFunction → edge]

```

Out[ ]:=

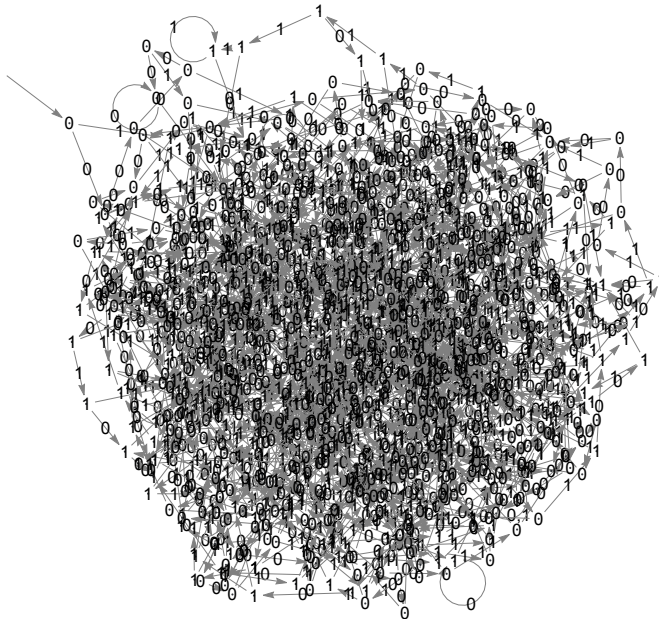

Supplement: Supplementary file 1 [file automata-of-finite-order.pdf]
