# Supplementary material for: Automata and finite order elements in the Nottingham group
Source: arXiv:2008.04971 ancillary file (2020-10-01)
Supplement: Supplementary file 2 [file verfication-of-synchronisation.pdf]

In[ ]:=

# Verification of the synchronising property of some automata

This Mathematica notebook accompanies the paper *Automata and finite order elements of the Nottingham group* by Jakub Byszewski, Gunther Cornelissen and Djurre Tijsma. It is verified that the automata corresponding to three series given in the notebook `automata-of-finite-order' satisfy the following criterion to be synchronising: there is a unique absorbing state and a path from any vertex to that absorbing.

[written by Jakub Byszewski, Gunther Cornelissen and Djurre Tijsma]

$\sigma_{(1,9)}$

The edge labelled graph A1

```

In[ ]:= A1 = {{1 → 2, 0}, {1 → 3, 1}, {4 → 5, 0}, {4 → 6, 1}, {2 → 7, 0}, {2 → 8, 1}, {9 → 10, 0},
{9 → 11, 1}, {5 → 12, 0}, {5 → 13, 1}, {14 → 15, 0}, {14 → 16, 1}, {17 → 18, 0},
{17 → 19, 1}, {7 → 20, 0}, {7 → 16, 1}, {21 → 22, 0}, {21 → 23, 1}, {24 → 20, 0},
{24 → 25, 1}, {26 → 27, 0}, {26 → 6, 1}, {28 → 29, 0}, {28 → 19, 1}, {18 → 30, 0},
{18 → 13, 1}, {31 → 22, 0}, {31 → 32, 1}, {33 → 34, 0}, {33 → 11, 1}, {35 → 7, 0},
{35 → 36, 1}, {10 → 24, 0}, {10 → 37, 1}, {38 → 7, 0}, {38 → 39, 1}, {12 → 24, 0},
{12 → 40, 1}, {41 → 42, 0}, {41 → 36, 1}, {43 → 22, 0}, {43 → 36, 1}, {15 → 20, 0},
{15 → 37, 1}, {44 → 45, 0}, {44 → 46, 1}, {47 → 22, 0}, {47 → 39, 1}, {42 → 20, 0},
{42 → 40, 1}, {20 → 48, 0}, {20 → 49, 1}, {48 → 50, 0}, {48 → 51, 1}, {52 → 53, 0},
{52 → 54, 1}, {55 → 49, 0}, {55 → 56, 1}, {50 → 50, 0}, {50 → 50, 1}, {57 → 58, 0},
{57 → 57, 1}, {54 → 59, 0}, {54 → 57, 1}, {56 → 51, 0}, {56 → 50, 1}, {22 → 48, 0},
{22 → 60, 1}, {61 → 60, 0}, {61 → 56, 1}, {58 → 62, 0}, {58 → 54, 1}, {63 → 30, 0},
{63 → 54, 1}, {49 → 35, 0}, {49 → 54, 1}, {64 → 43, 0}, {64 → 50, 1}, {53 → 21, 0},
{53 → 50, 1}, {65 → 21, 0}, {65 → 51, 1}, {45 → 31, 0}, {45 → 60, 1}, {34 → 31, 0},
{34 → 49, 1}, {51 → 48, 0}, {51 → 9, 1}, {59 → 66, 0}, {59 → 4, 1}, {67 → 65, 0},
{67 → 4, 1}, {29 → 62, 0}, {29 → 28, 1}, {66 → 21, 0}, {66 → 7, 1}, {60 → 38, 0},
{60 → 4, 1}, {62 → 21, 0}, {62 → 43, 1}, {27 → 35, 0}, {27 → 28, 1}, {68 → 47, 0},
{68 → 9, 1}, {30 → 31, 0}, {30 → 9, 1}, {3 → 3, 0}, {3 → 69, 1}, {70 → 70, 0},
{70 → 71, 1}, {16 → 8, 0}, {16 → 72, 1}, {19 → 73, 0}, {19 → 74, 1}, {72 → 75, 0},
{72 → 76, 1}, {77 → 70, 0}, {77 → 78, 1}, {74 → 79, 0}, {74 → 78, 1}, {79 → 77, 0},
{79 → 80, 1}, {75 → 81, 0}, {75 → 82, 1}, {76 → 69, 0}, {76 → 76, 1}, {78 → 83, 0},
{78 → 78, 1}, {11 → 84, 0}, {11 → 74, 1}, {6 → 85, 0}, {6 → 72, 1}, {86 → 77, 0},
{86 → 87, 1}, {8 → 88, 0}, {8 → 89, 1}, {81 → 88, 0}, {81 → 90, 1}, {23 → 91, 0},
{23 → 92, 1}, {87 → 93, 0}, {87 → 94, 1}, {95 → 91, 0}, {95 → 96, 1}, {73 → 97, 0},
{73 → 98, 1}, {69 → 8, 0}, {69 → 98, 1}, {99 → 77, 0}, {99 → 92, 1}, {71 → 100, 0},
{71 → 92, 1}, {83 → 70, 0}, {83 → 89, 1}, {101 → 77, 0}, {101 → 96, 1},
{100 → 70, 0}, {100 → 90, 1}, {25 → 81, 0}, {25 → 94, 1}, {80 → 102, 0},
{80 → 72, 1}, {82 → 103, 0}, {82 → 74, 1}, {84 → 39, 0}, {84 → 82, 1}, {13 → 104, 0},
{13 → 76, 1}, {85 → 91, 0}, {85 → 80, 1}, {32 → 88, 0}, {32 → 78, 1}, {88 → 79, 0},
{88 → 64, 1}, {89 → 99, 0}, {89 → 52, 1}, {98 → 16, 0}, {98 → 55, 1}, {105 → 86, 0},
{105 → 52, 1}, {106 → 86, 0}, {106 → 67, 1}, {37 → 23, 0}, {37 → 61, 1},
{91 → 79, 0}, {91 → 68, 1}, {92 → 36, 0}, {92 → 61, 1}, {36 → 105, 0}, {36 → 52, 1},
{102 → 106, 0}, {102 → 64, 1}, {94 → 107, 0}, {94 → 63, 1}, {93 → 106, 0},
{93 → 68, 1}, {108 → 105, 0}, {108 → 67, 1}, {46 → 40, 0}, {46 → 55, 1},
{90 → 101, 0}, {90 → 14, 1}, {40 → 95, 0}, {40 → 17, 1}, {104 → 23, 0},
{104 → 26, 1}, {103 → 109, 0}, {103 → 26, 1}, {109 → 105, 0}, {109 → 44, 1},
{39 → 106, 0}, {39 → 14, 1}, {96 → 108, 0}, {96 → 17, 1}, {107 → 110, 0},
{107 → 17, 1}, {110 → 105, 0}, {110 → 33, 1}, {97 → 106, 0}, {97 → 41, 1}};

```

Constructing the corresponding directed graph:

```

In[ ]:= E1 = {}; For[k = 1, k < 221, k++, E1 = Append[E1, {A1[[k, 1]]}][[1]]];
In[ ]:= g1 = Graph[Range[110], E1];

```

The unique absorbing state is number 50:

```

In[ ]:= Position[Normal[Diagonal[AdjacencyMatrix[g1]]], 2]
Out[ ]:= {{50}}

```

The list of minimal distances from any vertex to the absorbing one has only finite entries:

```
In[*]:= Transpose[GraphDistanceMatrix[g1]] [[50]]
```

```
Out[*]= {5, 4, 5, 6, 5, 5, 3, 3, 5, 4, 6, 4, 6, 4, 3, 4, 6, 5, 5, 2, 3, 2, 4, 3, 4, 6, 5, 6, 5,
4, 3, 3, 5, 4, 4, 3, 3, 4, 5, 7, 4, 3, 3, 4, 4, 3, 3, 1, 5, 0, 2, 2, 1, 6, 2, 1,
6, 5, 5, 5, 2, 4, 5, 1, 3, 4, 4, 4, 4, 5, 4, 5, 4, 5, 4, 5, 6, 5, 4, 3, 3, 6, 4,
6, 4, 7, 6, 2, 3, 5, 5, 3, 5, 6, 6, 5, 5, 3, 4, 6, 6, 2, 5, 5, 3, 5, 5, 4, 4, 4}
```

$\sigma_8$

The edge-labelled graph A2

```
In[*]:= A2 = {{1 → 2, 0}, {1 → 3, 1}, {4 → 5, 0}, {4 → 3, 1}, {6 → 7, 0}, {6 → 8, 1}, {9 → 10, 0},
{9 → 11, 1}, {12 → 13, 0}, {12 → 8, 1}, {14 → 15, 0}, {14 → 11, 1}, {16 → 17, 0},
{16 → 18, 1}, {19 → 20, 0}, {19 → 18, 1}, {21 → 22, 0}, {21 → 23, 1}, {24 → 25, 0},
{24 → 23, 1}, {26 → 9, 0}, {26 → 27, 1}, {28 → 24, 0}, {28 → 27, 1}, {29 → 30, 0},
{29 → 31, 1}, {32 → 32, 0}, {32 → 31, 1}, {33 → 32, 0}, {33 → 34, 1}, {35 → 33, 0},
{35 → 36, 1}, {37 → 33, 0}, {37 → 38, 1}, {39 → 40, 0}, {39 → 41, 1}, {42 → 43, 0},
{42 → 3, 1}, {30 → 44, 0}, {30 → 41, 1}, {45 → 46, 0}, {45 → 3, 1}, {47 → 35, 0},
{47 → 48, 1}, {49 → 37, 0}, {49 → 50, 1}, {51 → 35, 0}, {51 → 8, 1}, {52 → 37, 0},
{52 → 53, 1}, {54 → 55, 0}, {54 → 18, 1}, {56 → 57, 0}, {56 → 27, 1}, {2 → 58, 0},
{2 → 59, 1}, {22 → 60, 0}, {22 → 61, 1}, {62 → 63, 0}, {62 → 64, 1}, {5 → 65, 0},
{5 → 66, 1}, {67 → 65, 0}, {67 → 68, 1}, {69 → 70, 0}, {69 → 71, 1}, {25 → 70, 0},
{25 → 72, 1}, {73 → 74, 0}, {73 → 75, 1}, {17 → 76, 0}, {17 → 77, 1}, {20 → 78, 0},
{20 → 79, 1}, {80 → 81, 0}, {80 → 82, 1}, {83 → 81, 0}, {83 → 84, 1}, {85 → 86, 0},
{85 → 87, 1}, {88 → 86, 0}, {88 → 89, 1}, {90 → 91, 0}, {90 → 92, 1}, {93 → 94, 0},
{93 → 89, 1}, {95 → 96, 0}, {95 → 97, 1}, {98 → 99, 0}, {98 → 79, 1},
{55 → 99, 0}, {55 → 100, 1}, {44 → 96, 0}, {44 → 101, 1}, {102 → 103, 0},
{102 → 101, 1}, {104 → 105, 0}, {104 → 89, 1}, {106 → 4, 0}, {106 → 107, 1},
{108 → 54, 0}, {108 → 109, 1}, {40 → 51, 0}, {40 → 109, 1}, {110 → 56, 0},
{110 → 107, 1}, {94 → 111, 0}, {94 → 107, 1}, {112 → 113, 0}, {112 → 114, 1},
{43 → 115, 0}, {43 → 116, 1}, {117 → 118, 0}, {117 → 116, 1}, {119 → 120, 0},
{119 → 114, 1}, {121 → 62, 0}, {121 → 68, 1}, {122 → 73, 0}, {122 → 123, 1},
{46 → 80, 0}, {46 → 68, 1}, {124 → 90, 0}, {124 → 123, 1}, {96 → 125, 0},
{96 → 123, 1}, {125 → 126, 0}, {125 → 127, 1}, {126 → 126, 0}, {126 → 75, 1},
{99 → 125, 0}, {99 → 128, 1}, {103 → 52, 0}, {103 → 114, 1}, {105 → 85, 0},
{105 → 89, 1}, {111 → 129, 0}, {111 → 130, 1}, {115 → 131, 0}, {115 → 132, 1},
{133 → 131, 0}, {133 → 134, 1}, {135 → 129, 0}, {135 → 27, 1}, {7 → 136, 0},
{7 → 137, 1}, {113 → 138, 0}, {113 → 139, 1}, {10 → 140, 0}, {10 → 141, 1},
{57 → 142, 0}, {57 → 143, 1}, {144 → 140, 0}, {144 → 145, 1}, {146 → 142, 0},
{146 → 11, 1}, {13 → 147, 0}, {13 → 38, 1}, {118 → 148, 0}, {118 → 149, 1},
{120 → 150, 0}, {120 → 50, 1}, {15 → 151, 0}, {15 → 152, 1}, {58 → 60, 0},
{58 → 93, 1}, {60 → 60, 0}, {60 → 106, 1}, {63 → 58, 0}, {63 → 112, 1},
{153 → 58, 0}, {153 → 124, 1}, {154 → 155, 0}, {154 → 121, 1}, {156 → 157, 0},
{156 → 121, 1}, {158 → 159, 0}, {158 → 46, 1}, {160 → 161, 0}, {160 → 46, 1},
{162 → 163, 0}, {162 → 122, 1}, {164 → 165, 0}, {164 → 122, 1}, {166 → 167, 0},
{166 → 124, 1}, {168 → 169, 0}, {168 → 124, 1}, {170 → 171, 0}, {170 → 26, 1},
```

$\{129 \rightarrow 153, 0\}$ ,  $\{129 \rightarrow 28, 1\}$ ,  $\{172 \rightarrow 173, 0\}$ ,  $\{172 \rightarrow 28, 1\}$ ,  $\{131 \rightarrow 153, 0\}$ ,  
 $\{131 \rightarrow 42, 1\}$ ,  $\{142 \rightarrow 63, 0\}$ ,  $\{142 \rightarrow 6, 1\}$ ,  $\{140 \rightarrow 63, 0\}$ ,  $\{140 \rightarrow 16, 1\}$ ,  
 $\{174 \rightarrow 175, 0\}$ ,  $\{174 \rightarrow 26, 1\}$ ,  $\{171 \rightarrow 176, 0\}$ ,  $\{171 \rightarrow 29, 1\}$ ,  $\{177 \rightarrow 178, 0\}$ ,  
 $\{177 \rightarrow 32, 1\}$ ,  $\{179 \rightarrow 86, 0\}$ ,  $\{179 \rightarrow 32, 1\}$ ,  $\{180 \rightarrow 181, 0\}$ ,  $\{180 \rightarrow 29, 1\}$ ,  
 $\{182 \rightarrow 183, 0\}$ ,  $\{182 \rightarrow 29, 1\}$ ,  $\{173 \rightarrow 65, 0\}$ ,  $\{173 \rightarrow 46, 1\}$ ,  $\{175 \rightarrow 184, 0\}$ ,  
 $\{175 \rightarrow 26, 1\}$ ,  $\{185 \rightarrow 154, 0\}$ ,  $\{185 \rightarrow 186, 1\}$ ,  $\{187 \rightarrow 129, 0\}$ ,  $\{187 \rightarrow 188, 1\}$ ,  
 $\{189 \rightarrow 179, 0\}$ ,  $\{189 \rightarrow 188, 1\}$ ,  $\{190 \rightarrow 162, 0\}$ ,  $\{190 \rightarrow 186, 1\}$ ,  $\{186 \rightarrow 191, 0\}$ ,  
 $\{186 \rightarrow 192, 1\}$ ,  $\{192 \rightarrow 187, 0\}$ ,  $\{192 \rightarrow 193, 1\}$ ,  $\{193 \rightarrow 193, 0\}$ ,  $\{193 \rightarrow 193, 1\}$ ,  
 $\{188 \rightarrow 194, 0\}$ ,  $\{188 \rightarrow 192, 1\}$ ,  $\{151 \rightarrow 148, 0\}$ ,  $\{151 \rightarrow 194, 1\}$ ,  $\{148 \rightarrow 193, 0\}$ ,  
 $\{148 \rightarrow 187, 1\}$ ,  $\{195 \rightarrow 148, 0\}$ ,  $\{195 \rightarrow 191, 1\}$ ,  $\{196 \rightarrow 197, 0\}$ ,  $\{196 \rightarrow 162, 1\}$ ,  
 $\{191 \rightarrow 198, 0\}$ ,  $\{191 \rightarrow 164, 1\}$ ,  $\{199 \rightarrow 200, 0\}$ ,  $\{199 \rightarrow 164, 1\}$ ,  $\{201 \rightarrow 202, 0\}$ ,  
 $\{201 \rightarrow 162, 1\}$ ,  $\{203 \rightarrow 204, 0\}$ ,  $\{203 \rightarrow 166, 1\}$ ,  $\{194 \rightarrow 205, 0\}$ ,  $\{194 \rightarrow 166, 1\}$ ,  
 $\{206 \rightarrow 207, 0\}$ ,  $\{206 \rightarrow 168, 1\}$ ,  $\{208 \rightarrow 209, 0\}$ ,  $\{208 \rightarrow 168, 1\}$ ,  $\{65 \rightarrow 151, 0\}$ ,  
 $\{65 \rightarrow 129, 1\}$ ,  $\{86 \rightarrow 195, 0\}$ ,  $\{86 \rightarrow 162, 1\}$ ,  $\{70 \rightarrow 151, 0\}$ ,  $\{70 \rightarrow 179, 1\}$ ,  
 $\{81 \rightarrow 195, 0\}$ ,  $\{81 \rightarrow 154, 1\}$ ,  $\{178 \rightarrow 142, 0\}$ ,  $\{178 \rightarrow 168, 1\}$ ,  $\{181 \rightarrow 210, 0\}$ ,  
 $\{181 \rightarrow 192, 1\}$ ,  $\{183 \rightarrow 211, 0\}$ ,  $\{183 \rightarrow 186, 1\}$ ,  $\{155 \rightarrow 95, 0\}$ ,  $\{155 \rightarrow 203, 1\}$ ,  
 $\{74 \rightarrow 95, 0\}$ ,  $\{74 \rightarrow 199, 1\}$ ,  $\{176 \rightarrow 44, 0\}$ ,  $\{176 \rightarrow 189, 1\}$ ,  $\{78 \rightarrow 44, 0\}$ ,  
 $\{78 \rightarrow 192, 1\}$ ,  $\{197 \rightarrow 67, 0\}$ ,  $\{197 \rightarrow 194, 1\}$ ,  $\{198 \rightarrow 98, 0\}$ ,  $\{198 \rightarrow 177, 1\}$ ,  
 $\{136 \rightarrow 55, 0\}$ ,  $\{136 \rightarrow 164, 1\}$ ,  $\{138 \rightarrow 98, 0\}$ ,  $\{138 \rightarrow 172, 1\}$ ,  $\{210 \rightarrow 55, 0\}$ ,  
 $\{210 \rightarrow 156, 1\}$ ,  $\{157 \rightarrow 33, 0\}$ ,  $\{157 \rightarrow 206, 1\}$ ,  $\{159 \rightarrow 69, 0\}$ ,  $\{159 \rightarrow 179, 1\}$ ,  
 $\{200 \rightarrow 37, 0\}$ ,  $\{200 \rightarrow 180, 1\}$ ,  $\{161 \rightarrow 144, 0\}$ ,  $\{161 \rightarrow 182, 1\}$ ,  $\{202 \rightarrow 146, 0\}$ ,  
 $\{202 \rightarrow 208, 1\}$ ,  $\{163 \rightarrow 47, 0\}$ ,  $\{163 \rightarrow 19, 1\}$ ,  $\{76 \rightarrow 51, 0\}$ ,  $\{76 \rightarrow 26, 1\}$ ,  
 $\{91 \rightarrow 47, 0\}$ ,  $\{91 \rightarrow 12, 1\}$ ,  $\{184 \rightarrow 51, 0\}$ ,  $\{184 \rightarrow 45, 1\}$ ,  $\{204 \rightarrow 126, 0\}$ ,  
 $\{204 \rightarrow 108, 1\}$ ,  $\{165 \rightarrow 99, 0\}$ ,  $\{165 \rightarrow 21, 1\}$ ,  $\{205 \rightarrow 49, 0\}$ ,  $\{205 \rightarrow 110, 1\}$ ,  
 $\{147 \rightarrow 52, 0\}$ ,  $\{147 \rightarrow 122, 1\}$ ,  $\{150 \rightarrow 49, 0\}$ ,  $\{150 \rightarrow 104, 1\}$ ,  $\{211 \rightarrow 52, 0\}$ ,  
 $\{211 \rightarrow 119, 1\}$ ,  $\{167 \rightarrow 133, 0\}$ ,  $\{167 \rightarrow 106, 1\}$ ,  $\{207 \rightarrow 135, 0\}$ ,  $\{207 \rightarrow 16, 1\}$ ,  
 $\{169 \rightarrow 83, 0\}$ ,  $\{169 \rightarrow 40, 1\}$ ,  $\{209 \rightarrow 88, 0\}$ ,  $\{209 \rightarrow 24, 1\}$ ,  $\{3 \rightarrow 82, 0\}$ ,  
 $\{3 \rightarrow 185, 1\}$ ,  $\{27 \rightarrow 89, 0\}$ ,  $\{27 \rightarrow 190, 1\}$ ,  $\{41 \rightarrow 84, 0\}$ ,  $\{41 \rightarrow 185, 1\}$ ,  
 $\{31 \rightarrow 87, 0\}$ ,  $\{31 \rightarrow 190, 1\}$ ,  $\{149 \rightarrow 212, 0\}$ ,  $\{149 \rightarrow 156, 1\}$ ,  $\{137 \rightarrow 213, 0\}$ ,  
 $\{137 \rightarrow 156, 1\}$ ,  $\{38 \rightarrow 214, 0\}$ ,  $\{38 \rightarrow 154, 1\}$ ,  $\{132 \rightarrow 215, 0\}$ ,  $\{132 \rightarrow 154, 1\}$ ,  
 $\{216 \rightarrow 212, 0\}$ ,  $\{216 \rightarrow 164, 1\}$ ,  $\{217 \rightarrow 218, 0\}$ ,  $\{217 \rightarrow 172, 1\}$ ,  $\{219 \rightarrow 218, 0\}$ ,  
 $\{219 \rightarrow 177, 1\}$ ,  $\{220 \rightarrow 68, 0\}$ ,  $\{220 \rightarrow 187, 1\}$ ,  $\{221 \rightarrow 66, 0\}$ ,  $\{221 \rightarrow 187, 1\}$ ,  
 $\{130 \rightarrow 71, 0\}$ ,  $\{130 \rightarrow 189, 1\}$ ,  $\{34 \rightarrow 72, 0\}$ ,  $\{34 \rightarrow 189, 1\}$ ,  $\{222 \rightarrow 223, 0\}$ ,  
 $\{222 \rightarrow 158, 1\}$ ,  $\{36 \rightarrow 224, 0\}$ ,  $\{36 \rightarrow 160, 1\}$ ,  $\{134 \rightarrow 225, 0\}$ ,  $\{134 \rightarrow 160, 1\}$ ,  
 $\{226 \rightarrow 227, 0\}$ ,  $\{226 \rightarrow 203, 1\}$ ,  $\{228 \rightarrow 227, 0\}$ ,  $\{228 \rightarrow 199, 1\}$ ,  $\{229 \rightarrow 230, 0\}$ ,  
 $\{229 \rightarrow 192, 1\}$ ,  $\{231 \rightarrow 230, 0\}$ ,  $\{231 \rightarrow 189, 1\}$ ,  $\{232 \rightarrow 233, 0\}$ ,  $\{232 \rightarrow 190, 1\}$ ,  
 $\{234 \rightarrow 235, 0\}$ ,  $\{234 \rightarrow 154, 1\}$ ,  $\{236 \rightarrow 237, 0\}$ ,  $\{236 \rightarrow 160, 1\}$ ,  $\{238 \rightarrow 239, 0\}$ ,  
 $\{238 \rightarrow 196, 1\}$ ,  $\{240 \rightarrow 241, 0\}$ ,  $\{240 \rightarrow 170, 1\}$ ,  $\{242 \rightarrow 243, 0\}$ ,  $\{242 \rightarrow 129, 1\}$ ,  
 $\{244 \rightarrow 243, 0\}$ ,  $\{244 \rightarrow 179, 1\}$ ,  $\{245 \rightarrow 246, 0\}$ ,  $\{245 \rightarrow 162, 1\}$ ,  $\{247 \rightarrow 246, 0\}$ ,  
 $\{247 \rightarrow 154, 1\}$ ,  $\{243 \rightarrow 248, 0\}$ ,  $\{243 \rightarrow 194, 1\}$ ,  $\{248 \rightarrow 249, 0\}$ ,  $\{248 \rightarrow 187, 1\}$ ,  
 $\{249 \rightarrow 249, 0\}$ ,  $\{249 \rightarrow 193, 1\}$ ,  $\{246 \rightarrow 248, 0\}$ ,  $\{246 \rightarrow 191, 1\}$ ,  $\{250 \rightarrow 216, 0\}$ ,  
 $\{250 \rightarrow 199, 1\}$ ,  $\{251 \rightarrow 252, 0\}$ ,  $\{251 \rightarrow 201, 1\}$ ,  $\{253 \rightarrow 217, 0\}$ ,  $\{253 \rightarrow 172, 1\}$ ,  
 $\{254 \rightarrow 255, 0\}$ ,  $\{254 \rightarrow 174, 1\}$ ,  $\{256 \rightarrow 257, 0\}$ ,  $\{256 \rightarrow 6, 1\}$ ,  $\{241 \rightarrow 257, 0\}$ ,  
 $\{241 \rightarrow 16, 1\}$ ,  $\{252 \rightarrow 258, 0\}$ ,  $\{252 \rightarrow 42, 1\}$ ,  $\{259 \rightarrow 258, 0\}$ ,  $\{259 \rightarrow 28, 1\}$ ,  
 $\{257 \rightarrow 260, 0\}$ ,  $\{257 \rightarrow 112, 1\}$ ,  $\{260 \rightarrow 261, 0\}$ ,  $\{260 \rightarrow 93, 1\}$ ,  $\{261 \rightarrow 261, 0\}$ ,  
 $\{261 \rightarrow 106, 1\}$ ,  $\{258 \rightarrow 260, 0\}$ ,  $\{258 \rightarrow 124, 1\}$ ,  $\{262 \rightarrow 263, 0\}$ ,  $\{262 \rightarrow 12, 1\}$ ,  
 $\{264 \rightarrow 244, 0\}$ ,  $\{264 \rightarrow 44, 1\}$ ,  $\{265 \rightarrow 228, 0\}$ ,  $\{265 \rightarrow 102, 1\}$ ,  $\{266 \rightarrow 229, 0\}$ ,

```

{266 → 14, 1}, {267 → 247, 0}, {267 → 9, 1}, {268 → 269, 0}, {268 → 104, 1},
{143 → 270, 0}, {143 → 112, 1}, {239 → 271, 0}, {239 → 122, 1}, {48 → 272, 0},
{48 → 112, 1}, {273 → 271, 0}, {273 → 119, 1}, {274 → 275, 0}, {274 → 119, 1},
{276 → 277, 0}, {276 → 110, 1}, {255 → 277, 0}, {255 → 104, 1}, {8 → 278, 0},
{8 → 43, 1}, {18 → 279, 0}, {18 → 117, 1}, {23 → 280, 0}, {23 → 117, 1},
{11 → 281, 0}, {11 → 43, 1}, {53 → 282, 0}, {53 → 39, 1}, {145 → 283, 0},
{145 → 39, 1}, {284 → 285, 0}, {284 → 30, 1}, {286 → 287, 0}, {286 → 30, 1},
{139 → 288, 0}, {139 → 42, 1}, {152 → 289, 0}, {152 → 42, 1}, {50 → 290, 0},
{50 → 45, 1}, {141 → 291, 0}, {141 → 45, 1}, {263 → 292, 0}, {263 → 26, 1},
{293 → 292, 0}, {293 → 45, 1}, {269 → 294, 0}, {269 → 12, 1}, {295 → 294, 0},
{295 → 19, 1}, {296 → 297, 0}, {296 → 39, 1}, {298 → 299, 0}, {298 → 112, 1},
{300 → 301, 0}, {300 → 43, 1}, {59 → 238, 0}, {59 → 128, 1}, {128 → 240, 0},
{128 → 66, 1}, {66 → 242, 0}, {66 → 66, 1}, {302 → 242, 0}, {302 → 68, 1},
{303 → 250, 0}, {303 → 128, 1}, {304 → 244, 0}, {304 → 71, 1}, {235 → 244, 0},
{235 → 72, 1}, {114 → 262, 0}, {114 → 303, 1}, {68 → 260, 0}, {68 → 59, 1},
{123 → 264, 0}, {123 → 59, 1}, {116 → 266, 0}, {116 → 303, 1}, {71 → 293, 0},
{71 → 305, 1}, {127 → 296, 0}, {127 → 305, 1}, {306 → 298, 0}, {306 → 307, 1},
{308 → 300, 0}, {308 → 307, 1}, {282 → 226, 0}, {282 → 128, 1}, {75 → 232, 0},
{75 → 97, 1}, {72 → 231, 0}, {72 → 97, 1}, {92 → 234, 0}, {92 → 87, 1},
{61 → 236, 0}, {61 → 87, 1}, {309 → 245, 0}, {309 → 89, 1}, {310 → 247, 0},
{310 → 84, 1}, {285 → 245, 0}, {285 → 87, 1}, {301 → 247, 0}, {301 → 82, 1},
{283 → 295, 0}, {283 → 303, 1}, {287 → 258, 0}, {287 → 307, 1}, {82 → 256, 0},
{82 → 143, 1}, {64 → 265, 0}, {64 → 48, 1}, {79 → 267, 0}, {79 → 143, 1},
{77 → 268, 0}, {77 → 48, 1}, {311 → 241, 0}, {311 → 145, 1}, {312 → 256, 0},
{312 → 11, 1}, {237 → 241, 0}, {237 → 141, 1}, {89 → 149, 0}, {89 → 220, 1},
{107 → 3, 0}, {107 → 221, 1}, {109 → 221, 0}, {109 → 221, 1}, {101 → 222, 0},
{101 → 220, 1}, {97 → 23, 0}, {97 → 34, 1}, {305 → 152, 0}, {305 → 130, 1},
{87 → 273, 0}, {87 → 34, 1}, {307 → 284, 0}, {307 → 130, 1}, {100 → 251, 0},
{100 → 273, 1}, {84 → 246, 0}, {84 → 273, 1}, {313 → 253, 0}, {313 → 274, 1},
{314 → 254, 0}, {314 → 274, 1}, {288 → 249, 0}, {288 → 221, 1}, {289 → 259, 0},
{289 → 130, 1}, {315 → 259, 0}, {315 → 27, 1}, {316 → 252, 0}, {316 → 134, 1},
{299 → 252, 0}, {299 → 132, 1}, {290 → 276, 0}, {290 → 48, 1}, {291 → 219, 0},
{291 → 274, 1}, {270 → 302, 0}, {270 → 222, 1}, {271 → 317, 0}, {271 → 53, 1},
{294 → 223, 0}, {294 → 48, 1}, {292 → 223, 0}, {292 → 8, 1}, {277 → 317, 0},
{277 → 50, 1}, {317 → 318, 0}, {317 → 38, 1}, {223 → 318, 0}, {223 → 36, 1},
{318 → 233, 0}, {318 → 34, 1}, {233 → 233, 0}, {233 → 31, 1}, {224 → 311, 0},
{224 → 145, 1}, {272 → 312, 0}, {272 → 134, 1}, {275 → 218, 0}, {275 → 286, 1},
{225 → 304, 0}, {225 → 284, 1}, {212 → 319, 0}, {212 → 100, 1}, {227 → 297, 0},
{227 → 97, 1}, {230 → 297, 0}, {230 → 101, 1}, {218 → 319, 0}, {218 → 79, 1},
{278 → 309, 0}, {278 → 84, 1}, {319 → 280, 0}, {319 → 128, 1}, {280 → 320, 0},
{280 → 127, 1}, {320 → 320, 0}, {320 → 75, 1}, {297 → 280, 0}, {297 → 123, 1},
{213 → 294, 0}, {213 → 313, 1}, {214 → 310, 0}, {214 → 71, 1}, {279 → 277, 0},
{279 → 306, 1}, {281 → 315, 0}, {281 → 314, 1}, {215 → 316, 0}, {215 → 308, 1}};

```

Constructing the corresponding graph:

```
In[ ]:= E2 = {}; For[k = 1, k < 641, k++, E2 = Append[E2, {A2[[k, 1]]}[[1]]];
```

```
In[ ]:= g2 = Graph[Range[320], E2];
```

The unique absorbing vertex is number 193:

```
In[ ]:= Position[Normal[Diagonal[AdjacencyMatrix[g2]]], 2]
```

```
Out[ ]:= {{193}}
```

The list of minimal distances from any vertex to the absorbing one has only finite entries:

```
In[ ]:= Transpose[GraphDistanceMatrix[g2]][[193]]
```

```
Out[ ]:= {5, 8, 4, 5, 4, 7, 9, 6, 7, 7, 6, 7, 8, 4, 3, 5, 7, 4, 4, 3, 5, 7, 4, 5, 4, 5, 4,
5, 5, 5, 4, 5, 5, 4, 6, 7, 6, 7, 5, 6, 4, 5, 5, 6, 5, 5, 7, 6, 7, 6, 7, 7, 6, 5,
8, 5, 7, 7, 7, 7, 6, 7, 6, 7, 3, 5, 4, 8, 4, 3, 6, 5, 6, 6, 5, 6, 7, 2, 6, 4, 3,
7, 4, 4, 4, 3, 5, 4, 5, 7, 8, 6, 6, 6, 6, 7, 5, 7, 7, 8, 5, 6, 8, 6, 5, 6, 5, 6,
5, 6, 5, 5, 4, 8, 7, 4, 3, 2, 8, 7, 8, 7, 6, 7, 7, 6, 6, 6, 6, 4, 6, 8, 7, 7, 5,
8, 8, 6, 3, 6, 6, 7, 6, 7, 6, 7, 8, 1, 8, 7, 2, 6, 8, 8, 7, 7, 6, 6, 5, 6, 5, 6,
5, 7, 6, 8, 7, 6, 5, 6, 5, 5, 4, 6, 6, 4, 6, 7, 4, 3, 2, 4, 3, 6, 3, 2, 3, 2, 3,
3, 8, 1, 0, 8, 2, 6, 5, 7, 5, 4, 7, 7, 8, 7, 7, 7, 6, 6, 5, 8, 8, 8, 8, 6, 7, 8,
6, 7, 7, 4, 4, 7, 6, 7, 6, 7, 6, 6, 2, 6, 4, 4, 5, 6, 5, 7, 7, 7, 8, 7, 6, 4,
3, 4, 4, 3, 4, 2, 1, 6, 7, 6, 6, 7, 7, 7, 6, 8, 6, 7, 7, 7, 6, 5, 7, 3, 5, 7,
8, 6, 7, 8, 8, 8, 7, 7, 7, 5, 7, 7, 6, 7, 6, 6, 5, 6, 6, 2, 5, 7, 8, 7, 6, 7,
5, 6, 7, 6, 7, 6, 5, 5, 7, 5, 5, 6, 5, 6, 5, 5, 7, 7, 7, 8, 5, 7, 6, 5, 7, 6}
```

## $\sigma_{V,3}$

The edge-labelled graph A3

```
In[ ]:= A3 = {{1 → 2, 0}, {1 → 3, 1}, {4 → 5, 0}, {4 → 6, 1}, {2 → 7, 0}, {2 → 6, 1},
{5 → 8, 0}, {5 → 9, 1}, {10 → 8, 0}, {10 → 11, 1}, {12 → 13, 0}, {12 → 14, 1},
{15 → 5, 0}, {15 → 14, 1}, {7 → 10, 0}, {7 → 4, 1}, {8 → 16, 0}, {8 → 12, 1},
{13 → 17, 0}, {13 → 15, 1}, {16 → 16, 0}, {16 → 16, 1}, {17 → 17, 0},
{17 → 18, 1}, {18 → 12, 0}, {18 → 16, 1}, {3 → 19, 0}, {3 → 6, 1}, {20 → 21, 0},
{20 → 22, 1}, {23 → 24, 0}, {23 → 23, 1}, {6 → 20, 0}, {6 → 23, 1},
{9 → 24, 0}, {9 → 11, 1}, {22 → 20, 0}, {22 → 11, 1}, {19 → 9, 0}, {19 → 4, 1},
{11 → 11, 0}, {11 → 18, 1}, {25 → 25, 0}, {25 → 16, 1}, {21 → 11, 0},
{21 → 15, 1}, {24 → 25, 0}, {24 → 12, 1}, {14 → 9, 0}, {14 → 18, 1}};
```

Constructing the corresponding graph:

```
In[ ]:= E3 = {}; For[k = 1, k < 51, k++, E3 = Append[E3, {A3[[k, 1]]}][[1]]];
```

```
In[ ]:= g3 = Graph[Range[25], E3];
```

Verification that vertex 16 is the unique absorbing state:

```
In[ ]:= Position[Normal[Diagonal[AdjacencyMatrix[g3]]], 2]
```

```
Out[ ]:= {{16}}
```

The list of minimal distances from any vertex to the absorbing one has only finite entries:

```
In[ ]:= Transpose[GraphDistanceMatrix[g3]][[16]]
```

```
Out[ ]:= {5, 4, 5, 3, 2, 4, 3, 1, 3, 2, 2, 3, 3, 2, 3, 0, 2, 1, 4, 4, 3, 3, 3, 2, 1}
```
