# Supplementary material for: Automata and finite order elements in the Nottingham group
Source: arXiv:2008.04971 ancillary file (2020-10-01)
Supplement: Supplementary file 3 [file verification-of-non-sparseness.pdf]

# Verification of non-membership in $\hat{S}$

This Mathematica notebook accompanies the paper *Automata and finite order elements of the Nottingham group* by Jakub Byszewski, Gunther Cornelissen and Djurre Tijsma.

In the notebook, we verify that the automaton corresponding to the series  $\sigma_{(1,9)}$  satisfy the combinatorial conditions to prove non-membership in  $\hat{S}$ .

Remarks:

- In the paper, for  $\sigma_{(1,9)}$  the vertices are described through binary integers, but in the present text, we use the numbering of the vertices in the automaton graph.
- The Package “IntegerSequences”, version 1.53 by Eric Rowland is used to represent automata. For the computation of the automaton for  $\sigma_{(1,9)}$  we refer to the other notebook “automata-of-finite-order.nb”.

[written by Jakub Byszewski, Gunther Cornelissen and Djurre Tijsma]

```
In[ ]:= Import[
  "https://raw.githubusercontent.com/ericrowland/IntegerSequences/master/
  IntegerSequences.m"];
```

The automaton A corresponding to  $\sigma_{(1,9)}$  including the list of vertex labels L

```
In[ ]:= L = {1 → 0, 2 → 0, 3 → 1, 4 → 0, 5 → 0, 6 → 1, 7 → 0, 8 → 1, 9 → 0, 10 → 0, 11 → 1, 12 → 0,
  13 → 1, 14 → 0, 15 → 0, 16 → 1, 17 → 0, 18 → 0, 19 → 1, 20 → 0, 21 → 0, 22 → 0,
  23 → 1, 24 → 0, 25 → 1, 26 → 0, 27 → 0, 28 → 0, 29 → 0, 30 → 0, 31 → 0, 32 → 1,
  33 → 0, 34 → 0, 35 → 0, 36 → 1, 37 → 1, 38 → 0, 39 → 1, 40 → 1, 41 → 0, 42 → 0,
  43 → 0, 44 → 0, 45 → 0, 46 → 1, 47 → 0, 48 → 0, 49 → 0, 50 → 0, 51 → 0, 52 → 0,
  53 → 0, 54 → 0, 55 → 0, 56 → 0, 57 → 0, 58 → 0, 59 → 0, 60 → 0, 61 → 0, 62 → 0,
  63 → 0, 64 → 0, 65 → 0, 66 → 0, 67 → 0, 68 → 0, 69 → 1, 70 → 1, 71 → 1, 72 → 1,
  73 → 1, 74 → 1, 75 → 1, 76 → 1, 77 → 1, 78 → 1, 79 → 1, 80 → 1, 81 → 1, 82 → 1,
  83 → 1, 84 → 1, 85 → 1, 86 → 1, 87 → 1, 88 → 1, 89 → 1, 90 → 1, 91 → 1, 92 → 1,
  93 → 1, 94 → 1, 95 → 1, 96 → 1, 97 → 1, 98 → 1, 99 → 1, 100 → 1, 101 → 1, 102 → 1,
  103 → 1, 104 → 1, 105 → 1, 106 → 1, 107 → 1, 108 → 1, 109 → 1, 110 → 1};
```

```

In[ ]:= A = Automaton[{{1 → 2, 0}, {1 → 3, 1}, {4 → 5, 0}, {4 → 6, 1}, {2 → 7, 0}, {2 → 8, 1},
  {9 → 10, 0}, {9 → 11, 1}, {5 → 12, 0}, {5 → 13, 1}, {14 → 15, 0}, {14 → 16, 1},
  {17 → 18, 0}, {17 → 19, 1}, {7 → 20, 0}, {7 → 16, 1}, {21 → 22, 0}, {21 → 23, 1},
  {24 → 20, 0}, {24 → 25, 1}, {26 → 27, 0}, {26 → 6, 1}, {28 → 29, 0}, {28 → 19, 1},
  {18 → 30, 0}, {18 → 13, 1}, {31 → 22, 0}, {31 → 32, 1}, {33 → 34, 0}, {33 → 11, 1},
  {35 → 7, 0}, {35 → 36, 1}, {10 → 24, 0}, {10 → 37, 1}, {38 → 7, 0}, {38 → 39, 1},
  {12 → 24, 0}, {12 → 40, 1}, {41 → 42, 0}, {41 → 36, 1}, {43 → 22, 0}, {43 → 36, 1},
  {15 → 20, 0}, {15 → 37, 1}, {44 → 45, 0}, {44 → 46, 1}, {47 → 22, 0}, {47 → 39, 1},
  {42 → 20, 0}, {42 → 40, 1}, {20 → 48, 0}, {20 → 49, 1}, {48 → 50, 0}, {48 → 51, 1},
  {52 → 53, 0}, {52 → 54, 1}, {55 → 49, 0}, {55 → 56, 1}, {50 → 50, 0}, {50 → 50, 1},
  {57 → 58, 0}, {57 → 57, 1}, {54 → 59, 0}, {54 → 57, 1}, {56 → 51, 0}, {56 → 50, 1},
  {22 → 48, 0}, {22 → 60, 1}, {61 → 60, 0}, {61 → 56, 1}, {58 → 62, 0}, {58 → 54, 1},
  {63 → 30, 0}, {63 → 54, 1}, {49 → 35, 0}, {49 → 54, 1}, {64 → 43, 0}, {64 → 50, 1},
  {53 → 21, 0}, {53 → 50, 1}, {65 → 21, 0}, {65 → 51, 1}, {45 → 31, 0},
  {45 → 60, 1}, {34 → 31, 0}, {34 → 49, 1}, {51 → 48, 0}, {51 → 9, 1}, {59 → 66, 0},
  {59 → 4, 1}, {67 → 65, 0}, {67 → 4, 1}, {29 → 62, 0}, {29 → 28, 1}, {66 → 21, 0},
  {66 → 7, 1}, {60 → 38, 0}, {60 → 4, 1}, {62 → 21, 0}, {62 → 43, 1}, {27 → 35, 0},
  {27 → 28, 1}, {68 → 47, 0}, {68 → 9, 1}, {30 → 31, 0}, {30 → 9, 1}, {3 → 3, 0},
  {3 → 69, 1}, {70 → 70, 0}, {70 → 71, 1}, {16 → 8, 0}, {16 → 72, 1}, {19 → 73, 0},
  {19 → 74, 1}, {72 → 75, 0}, {72 → 76, 1}, {77 → 70, 0}, {77 → 78, 1}, {74 → 79, 0},
  {74 → 78, 1}, {79 → 77, 0}, {79 → 80, 1}, {75 → 81, 0}, {75 → 82, 1}, {76 → 69, 0},
  {76 → 76, 1}, {78 → 83, 0}, {78 → 78, 1}, {11 → 84, 0}, {11 → 74, 1}, {6 → 85, 0},
  {6 → 72, 1}, {86 → 77, 0}, {86 → 87, 1}, {8 → 88, 0}, {8 → 89, 1}, {81 → 88, 0},
  {81 → 90, 1}, {23 → 91, 0}, {23 → 92, 1}, {87 → 93, 0}, {87 → 94, 1}, {95 → 91, 0},
  {95 → 96, 1}, {73 → 97, 0}, {73 → 98, 1}, {69 → 8, 0}, {69 → 98, 1}, {99 → 77, 0},
  {99 → 92, 1}, {71 → 100, 0}, {71 → 92, 1}, {83 → 70, 0}, {83 → 89, 1},
  {101 → 77, 0}, {101 → 96, 1}, {100 → 70, 0}, {100 → 90, 1}, {25 → 81, 0},
  {25 → 94, 1}, {80 → 102, 0}, {80 → 72, 1}, {82 → 103, 0}, {82 → 74, 1},
  {84 → 39, 0}, {84 → 82, 1}, {13 → 104, 0}, {13 → 76, 1}, {85 → 91, 0}, {85 → 80, 1},
  {32 → 88, 0}, {32 → 78, 1}, {88 → 79, 0}, {88 → 64, 1}, {89 → 99, 0}, {89 → 52, 1},
  {98 → 16, 0}, {98 → 55, 1}, {105 → 86, 0}, {105 → 52, 1}, {106 → 86, 0},
  {106 → 67, 1}, {37 → 23, 0}, {37 → 61, 1}, {91 → 79, 0}, {91 → 68, 1}, {92 → 36, 0},
  {92 → 61, 1}, {36 → 105, 0}, {36 → 52, 1}, {102 → 106, 0}, {102 → 64, 1},
  {94 → 107, 0}, {94 → 63, 1}, {93 → 106, 0}, {93 → 68, 1}, {108 → 105, 0},
  {108 → 67, 1}, {46 → 40, 0}, {46 → 55, 1}, {90 → 101, 0}, {90 → 14, 1},
  {40 → 95, 0}, {40 → 17, 1}, {104 → 23, 0}, {104 → 26, 1}, {103 → 109, 0},
  {103 → 26, 1}, {109 → 105, 0}, {109 → 44, 1}, {39 → 106, 0}, {39 → 14, 1},
  {96 → 108, 0}, {96 → 17, 1}, {107 → 110, 0}, {107 → 17, 1}, {110 → 105, 0},
  {110 → 33, 1}, {97 → 106, 0}, {97 → 41, 1}}, 1, L1, InputAlphabet → {0, 1}];

```

The associated automaton with no output (in order to be able to follow along the numbering of vertices):

```

In[*]:= Ano = Automaton[{{1 → 2, 0}, {1 → 3, 1}, {4 → 5, 0}, {4 → 6, 1}, {2 → 7, 0}, {2 → 8, 1},
  {9 → 10, 0}, {9 → 11, 1}, {5 → 12, 0}, {5 → 13, 1}, {14 → 15, 0}, {14 → 16, 1},
  {17 → 18, 0}, {17 → 19, 1}, {7 → 20, 0}, {7 → 16, 1}, {21 → 22, 0}, {21 → 23, 1},
  {24 → 20, 0}, {24 → 25, 1}, {26 → 27, 0}, {26 → 6, 1}, {28 → 29, 0}, {28 → 19, 1},
  {18 → 30, 0}, {18 → 13, 1}, {31 → 22, 0}, {31 → 32, 1}, {33 → 34, 0}, {33 → 11, 1},
  {35 → 7, 0}, {35 → 36, 1}, {10 → 24, 0}, {10 → 37, 1}, {38 → 7, 0}, {38 → 39, 1},
  {12 → 24, 0}, {12 → 40, 1}, {41 → 42, 0}, {41 → 36, 1}, {43 → 22, 0}, {43 → 36, 1},
  {15 → 20, 0}, {15 → 37, 1}, {44 → 45, 0}, {44 → 46, 1}, {47 → 22, 0}, {47 → 39, 1},
  {42 → 20, 0}, {42 → 40, 1}, {20 → 48, 0}, {20 → 49, 1}, {48 → 50, 0}, {48 → 51, 1},
  {52 → 53, 0}, {52 → 54, 1}, {55 → 49, 0}, {55 → 56, 1}, {50 → 50, 0}, {50 → 50, 1},
  {57 → 58, 0}, {57 → 57, 1}, {54 → 59, 0}, {54 → 57, 1}, {56 → 51, 0}, {56 → 50, 1},
  {22 → 48, 0}, {22 → 60, 1}, {61 → 60, 0}, {61 → 56, 1}, {58 → 62, 0}, {58 → 54, 1},
  {63 → 30, 0}, {63 → 54, 1}, {49 → 35, 0}, {49 → 54, 1}, {64 → 43, 0}, {64 → 50, 1},
  {53 → 21, 0}, {53 → 50, 1}, {65 → 21, 0}, {65 → 51, 1}, {45 → 31, 0},
  {45 → 60, 1}, {34 → 31, 0}, {34 → 49, 1}, {51 → 48, 0}, {51 → 9, 1}, {59 → 66, 0},
  {59 → 4, 1}, {67 → 65, 0}, {67 → 4, 1}, {29 → 62, 0}, {29 → 28, 1}, {66 → 21, 0},
  {66 → 7, 1}, {60 → 38, 0}, {60 → 4, 1}, {62 → 21, 0}, {62 → 43, 1}, {27 → 35, 0},
  {27 → 28, 1}, {68 → 47, 0}, {68 → 9, 1}, {30 → 31, 0}, {30 → 9, 1}, {3 → 3, 0},
  {3 → 69, 1}, {70 → 70, 0}, {70 → 71, 1}, {16 → 8, 0}, {16 → 72, 1}, {19 → 73, 0},
  {19 → 74, 1}, {72 → 75, 0}, {72 → 76, 1}, {77 → 70, 0}, {77 → 78, 1}, {74 → 79, 0},
  {74 → 78, 1}, {79 → 77, 0}, {79 → 80, 1}, {75 → 81, 0}, {75 → 82, 1}, {76 → 69, 0},
  {76 → 76, 1}, {78 → 83, 0}, {78 → 78, 1}, {11 → 84, 0}, {11 → 74, 1}, {6 → 85, 0},
  {6 → 72, 1}, {86 → 77, 0}, {86 → 87, 1}, {8 → 88, 0}, {8 → 89, 1}, {81 → 88, 0},
  {81 → 90, 1}, {23 → 91, 0}, {23 → 92, 1}, {87 → 93, 0}, {87 → 94, 1}, {95 → 91, 0},
  {95 → 96, 1}, {73 → 97, 0}, {73 → 98, 1}, {69 → 8, 0}, {69 → 98, 1}, {99 → 77, 0},
  {99 → 92, 1}, {71 → 100, 0}, {71 → 92, 1}, {83 → 70, 0}, {83 → 89, 1},
  {101 → 77, 0}, {101 → 96, 1}, {100 → 70, 0}, {100 → 90, 1}, {25 → 81, 0},
  {25 → 94, 1}, {80 → 102, 0}, {80 → 72, 1}, {82 → 103, 0}, {82 → 74, 1},
  {84 → 39, 0}, {84 → 82, 1}, {13 → 104, 0}, {13 → 76, 1}, {85 → 91, 0}, {85 → 80, 1},
  {32 → 88, 0}, {32 → 78, 1}, {88 → 79, 0}, {88 → 64, 1}, {89 → 99, 0}, {89 → 52, 1},
  {98 → 16, 0}, {98 → 55, 1}, {105 → 86, 0}, {105 → 52, 1}, {106 → 86, 0},
  {106 → 67, 1}, {37 → 23, 0}, {37 → 61, 1}, {91 → 79, 0}, {91 → 68, 1}, {92 → 36, 0},
  {92 → 61, 1}, {36 → 105, 0}, {36 → 52, 1}, {102 → 106, 0}, {102 → 64, 1},
  {94 → 107, 0}, {94 → 63, 1}, {93 → 106, 0}, {93 → 68, 1}, {108 → 105, 0},
  {108 → 67, 1}, {46 → 40, 0}, {46 → 55, 1}, {90 → 101, 0}, {90 → 14, 1},
  {40 → 95, 0}, {40 → 17, 1}, {104 → 23, 0}, {104 → 26, 1}, {103 → 109, 0},
  {103 → 26, 1}, {109 → 105, 0}, {109 → 44, 1}, {39 → 106, 0}, {39 → 14, 1},
  {96 → 108, 0}, {96 → 17, 1}, {107 → 110, 0}, {107 → 17, 1}, {110 → 105, 0},
  {110 → 33, 1}, {97 → 106, 0}, {97 → 41, 1}}, 1, InputAlphabet → {0, 1}];

```

The words  $w_0, w_1, w_2$  (“Automaton” reads forward but we have the backwards reading convention!):

```

In[*]:= w0 = {0, 0, 0, 1, 1, 1}; w1 = {1}; w2 = {0, 1, 0, 1, 0, 0, 0, 0, 0};

```

The word  $w_0$  ends at vertex 57, that is mapped to itself by  $w_1$ :

```
In[*]:= Ano[w0]
Ano[Join[w0, w1]]
```

```
Out[*]:= 57
```

```
Out[*]:= 57
```

The vertex  $v$  is reached from start via  $w_2w_0$ :

```
In[*]:= v = Ano[Join[w0, w2]]
v0 = Ano[Join[Join[w0, w2], {0}]]
v1 = Ano[Join[Join[w0, w2], {1}]]
```

```
Out[*]:= 48
```

```
Out[*]:= 50
```

```
Out[*]:= 51
```

The automaton corresponding to  $v_1$  is not sparse; for this, follow the path 001 to a tied vertex  $t$ :

```
In[*]:= t = Ano[Join[Join[Join[w0, w2], {1}], {1, 0, 0}]]
```

```
Out[*]:= 24
```

The two walks  $p_1$  and  $p_2$  are of the same length and go from  $t$  to  $t$ , verifying that  $t$  is tied:

```
In[*]:= p1 = {0, 0, 1, 1, 0, 1, 0, 0, 1, 0, 0, 1, 1, 0, 0, 0, 0, 1, 1, 0, 0};
p2 = {0, 0, 1, 1, 0, 0, 0, 0, 1, 1, 0, 1, 0, 0, 1, 0, 0, 1, 1, 0, 0};
```

```
In[*]:= Ano[Join[Join[Join[Join[w0, w2], {1}], {1, 0, 0}], p1]]
Ano[Join[Join[Join[Join[w0, w2], {1}], {1, 0, 0}], p2]]
```

```
Out[*]:= 24
```

```
Out[*]:= 24
```

The automaton corresponding to  $v_0$  is sparse; for this, we verify that  $v_0$  has label 0 and two self-loops:

```
In[*]:= L[{50}]
Ano[Join[Join[Join[w0, w2], {0}], {0}]]
Ano[Join[Join[Join[w0, w2], {0}], {1}]]
```

```
Out[*]:= 50 → 0
```

```
Out[*]:= 50
```

```
Out[*]:= 50
```
